# Supplementary material for: Mineral snowflakes on exoplanets and brown dwarfs: Effects of micro-porosity, size distributions, and particle shape
Source: arXiv:2004.13502 source file (2020-04-28)

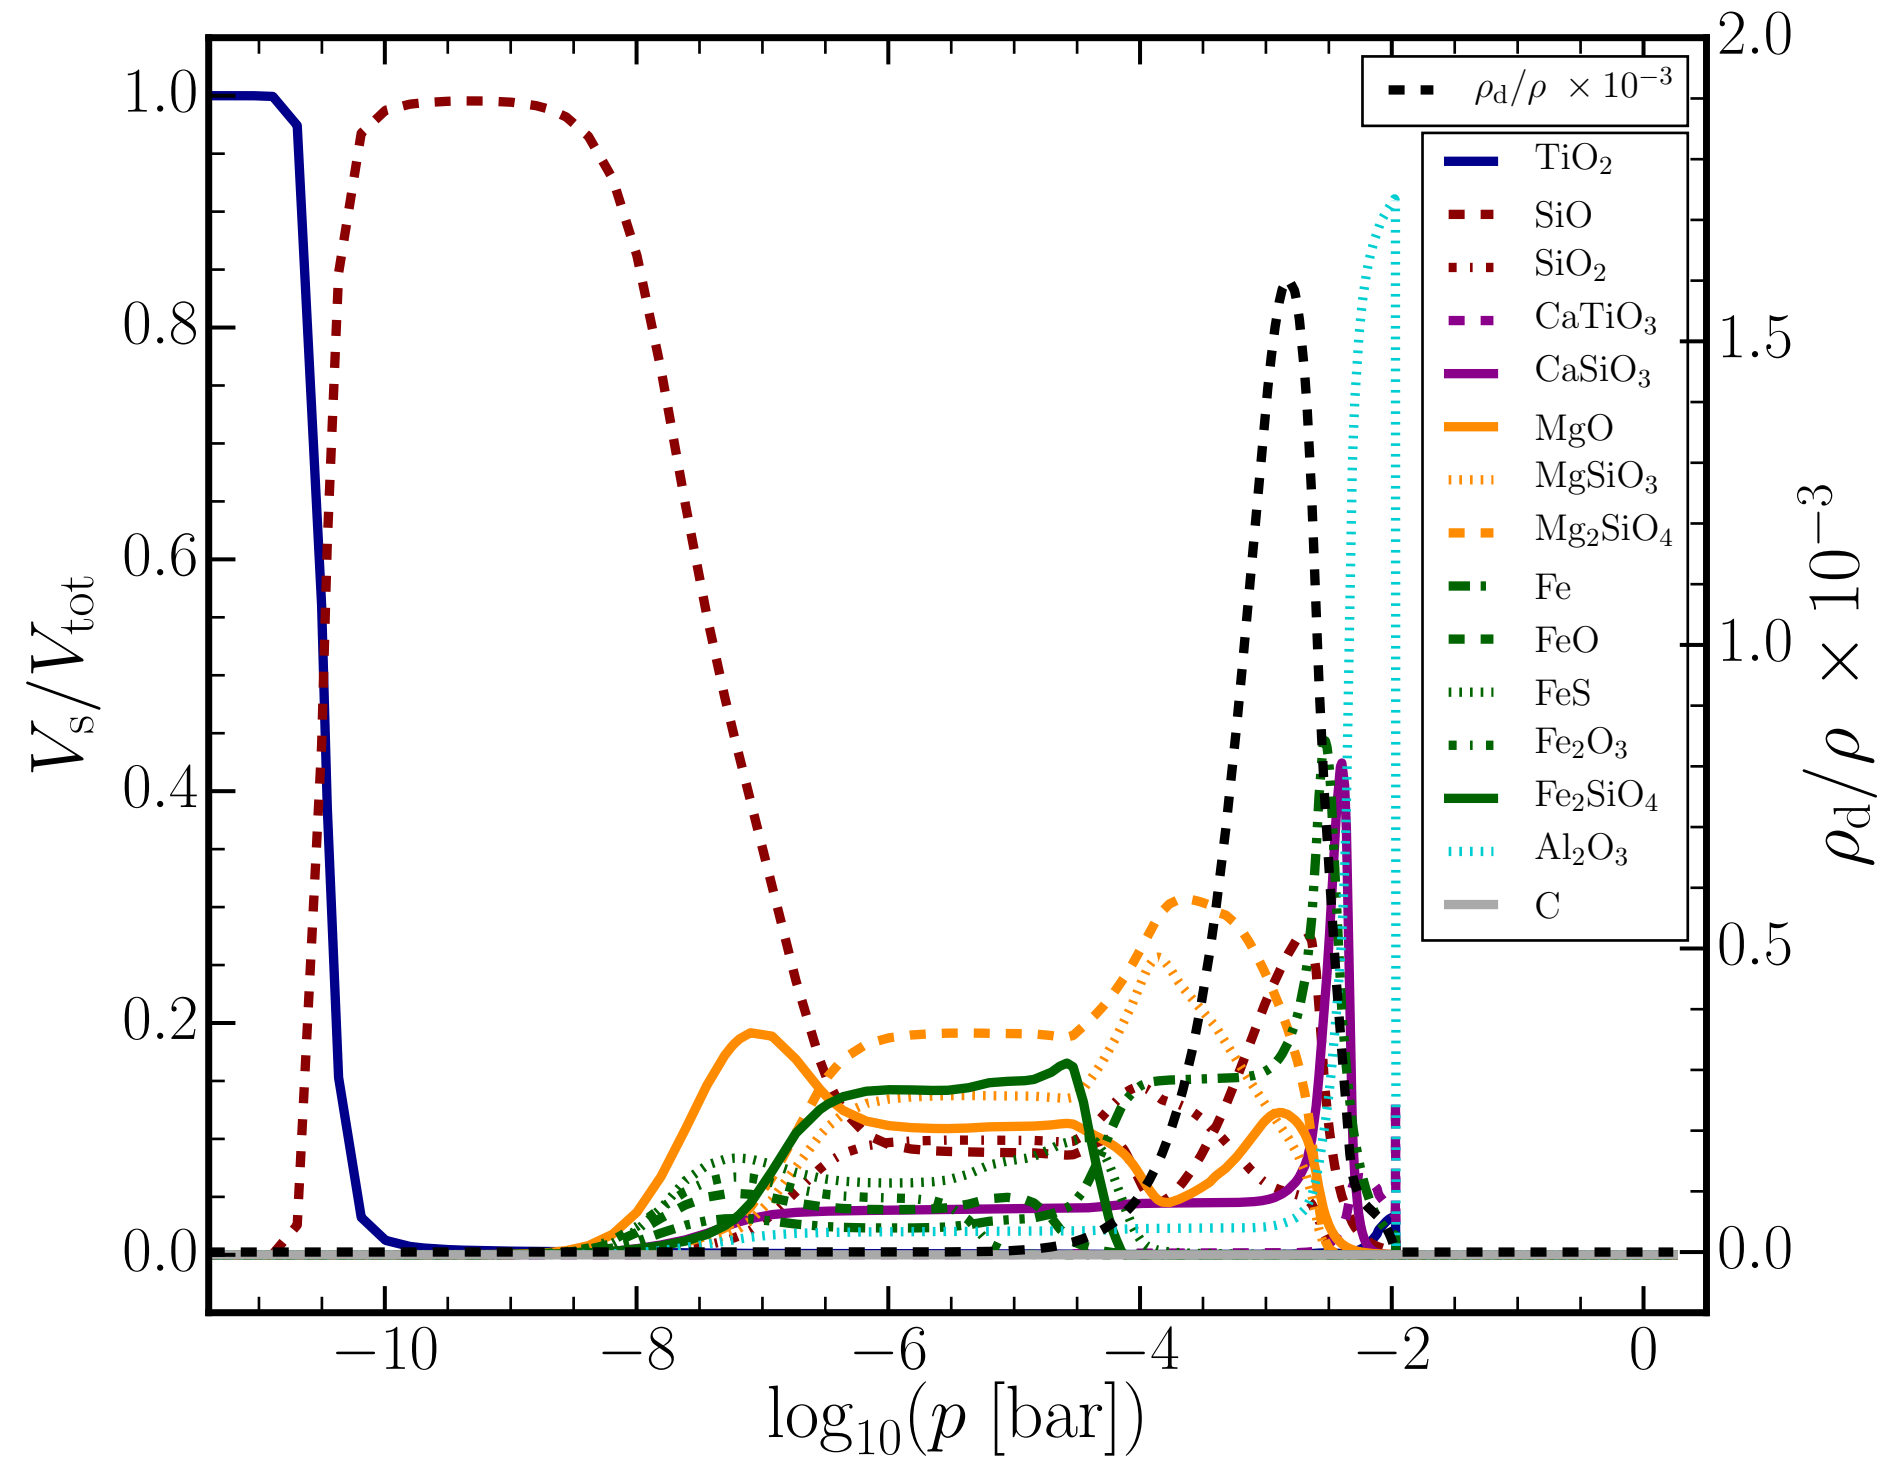

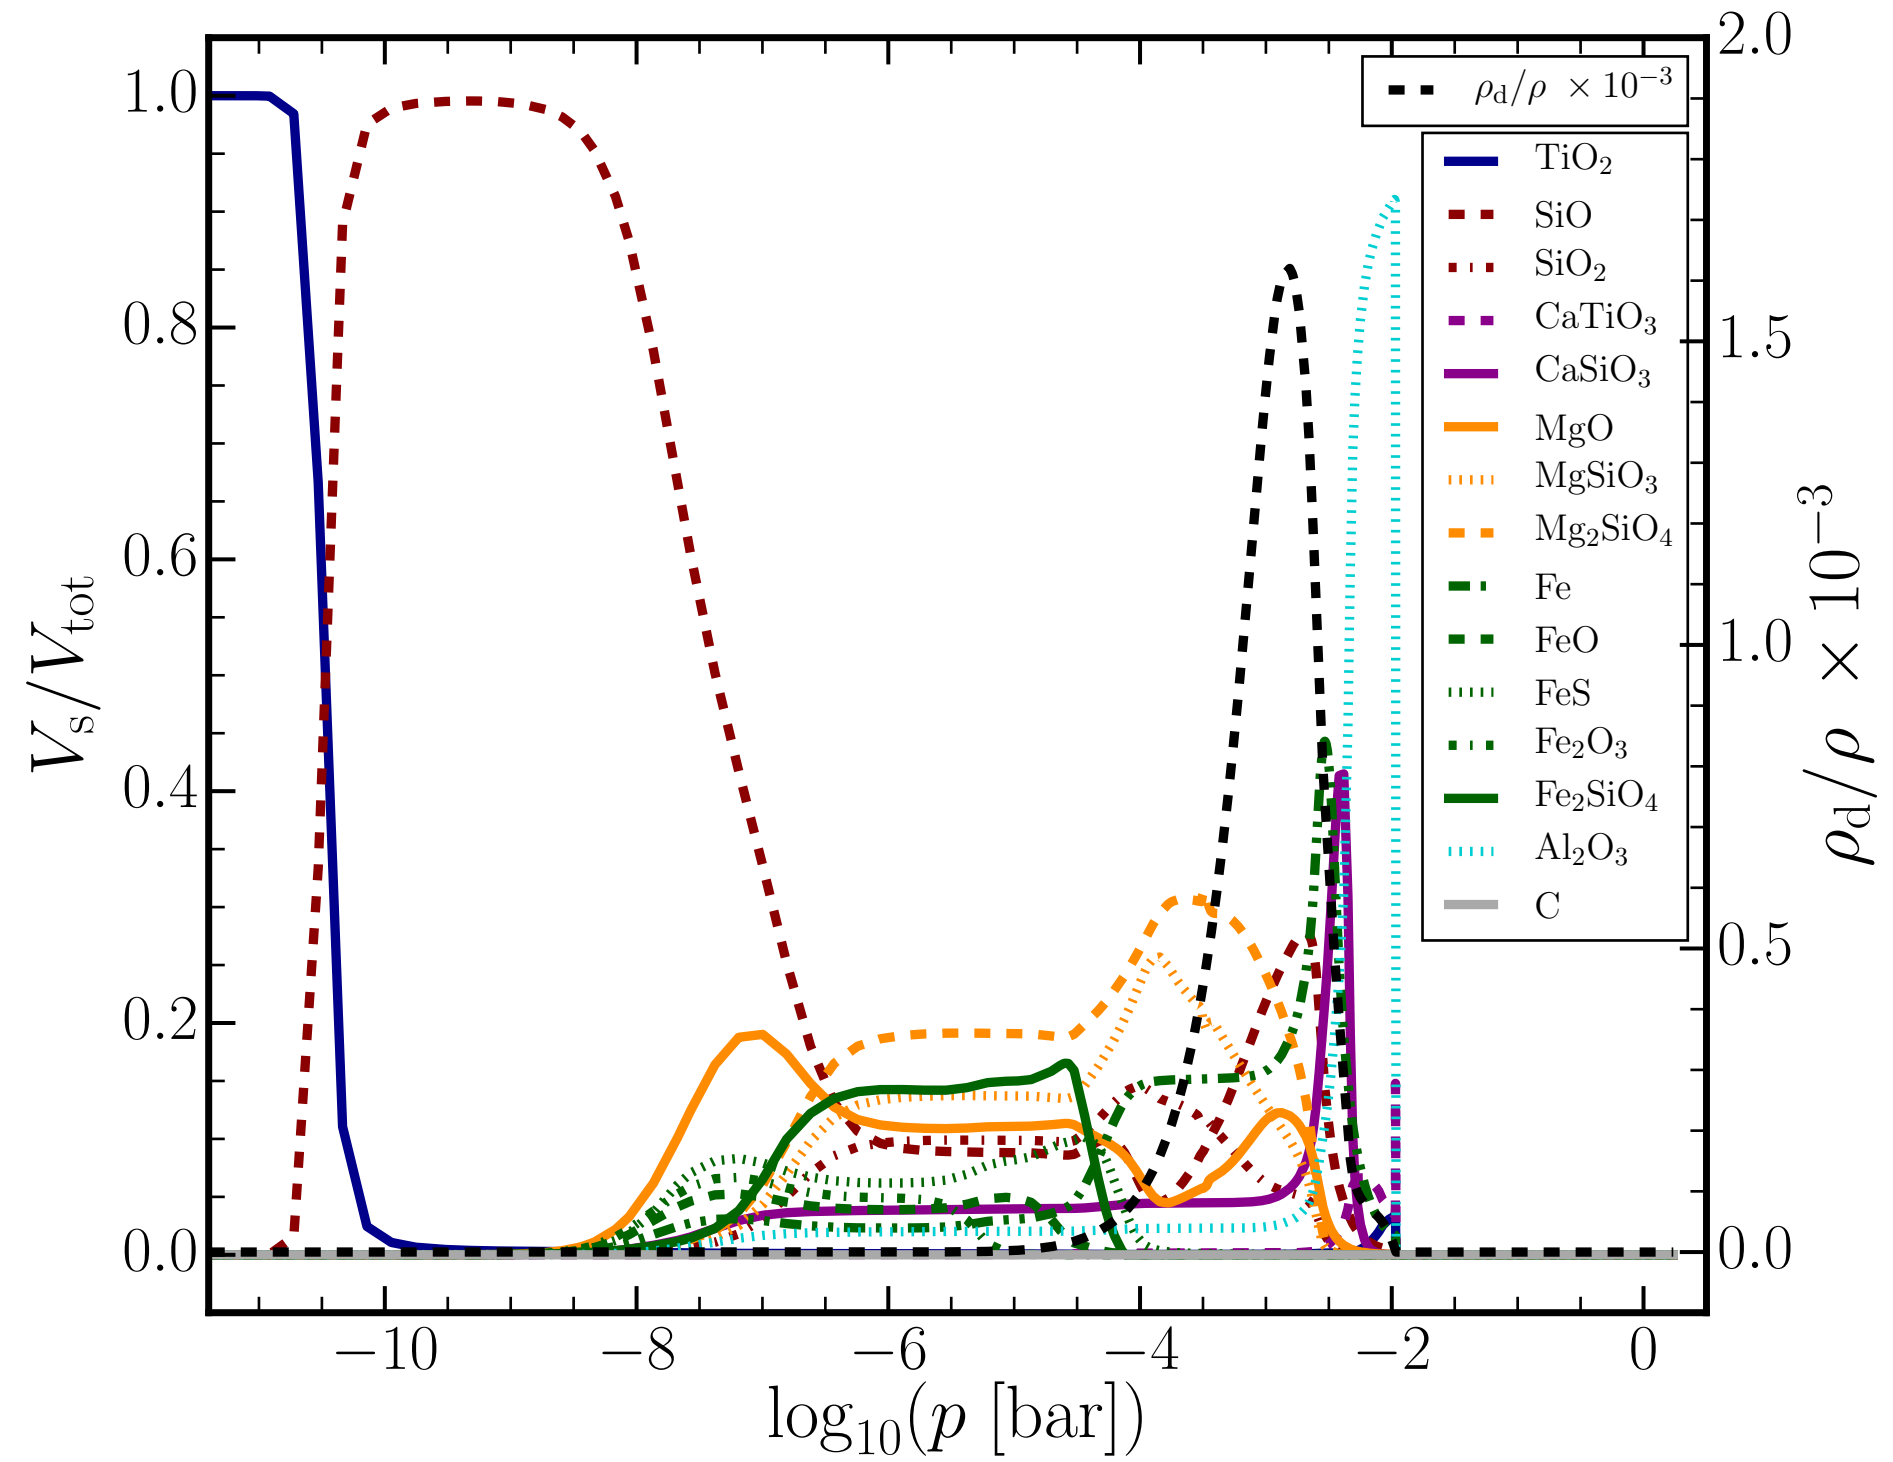

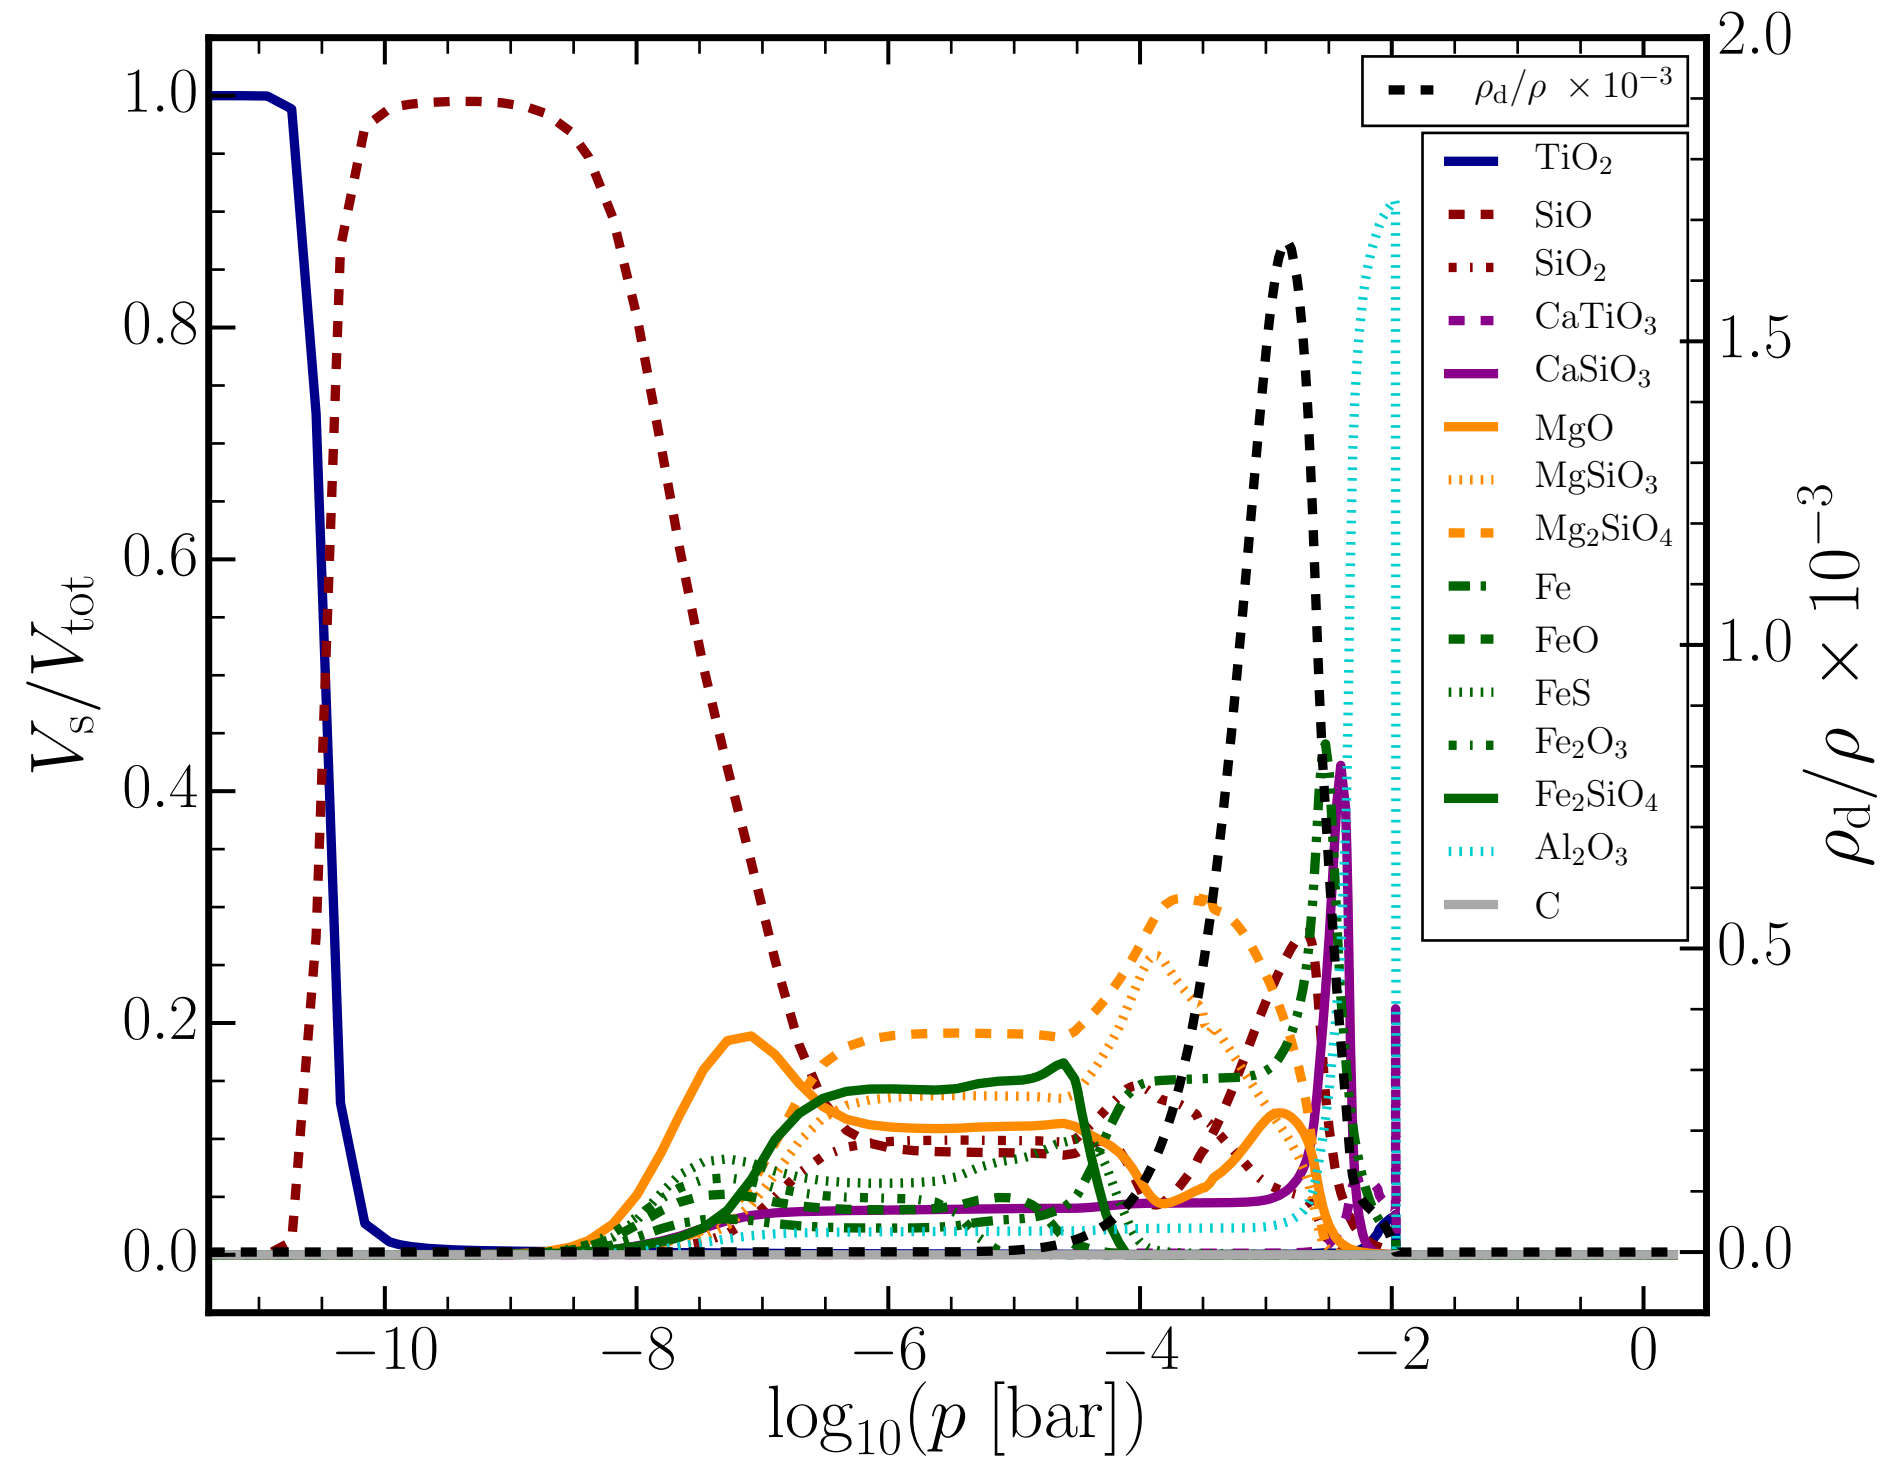

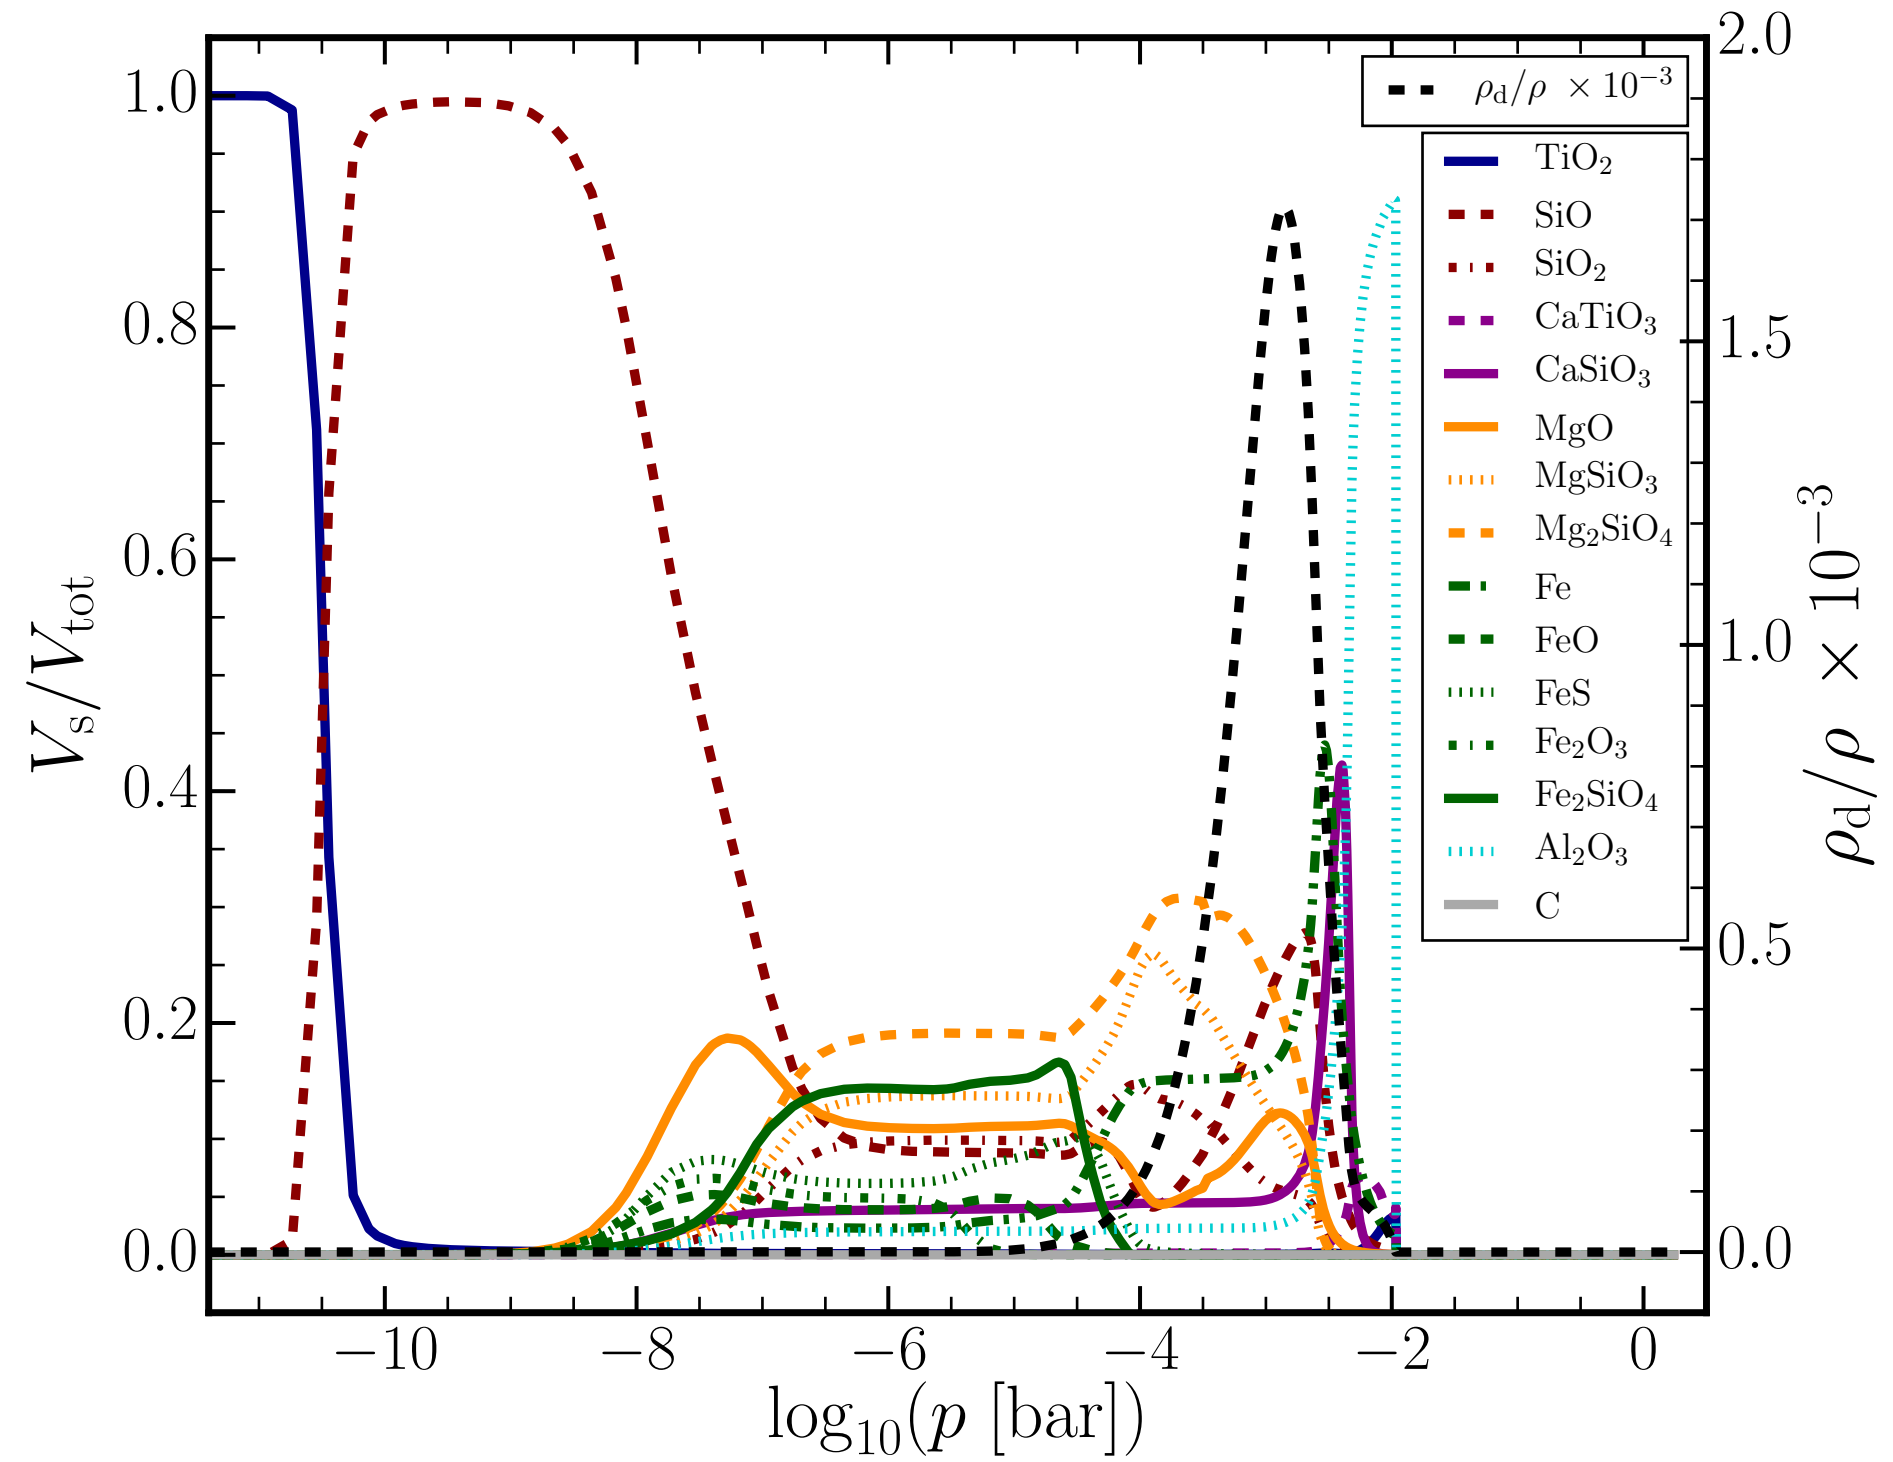

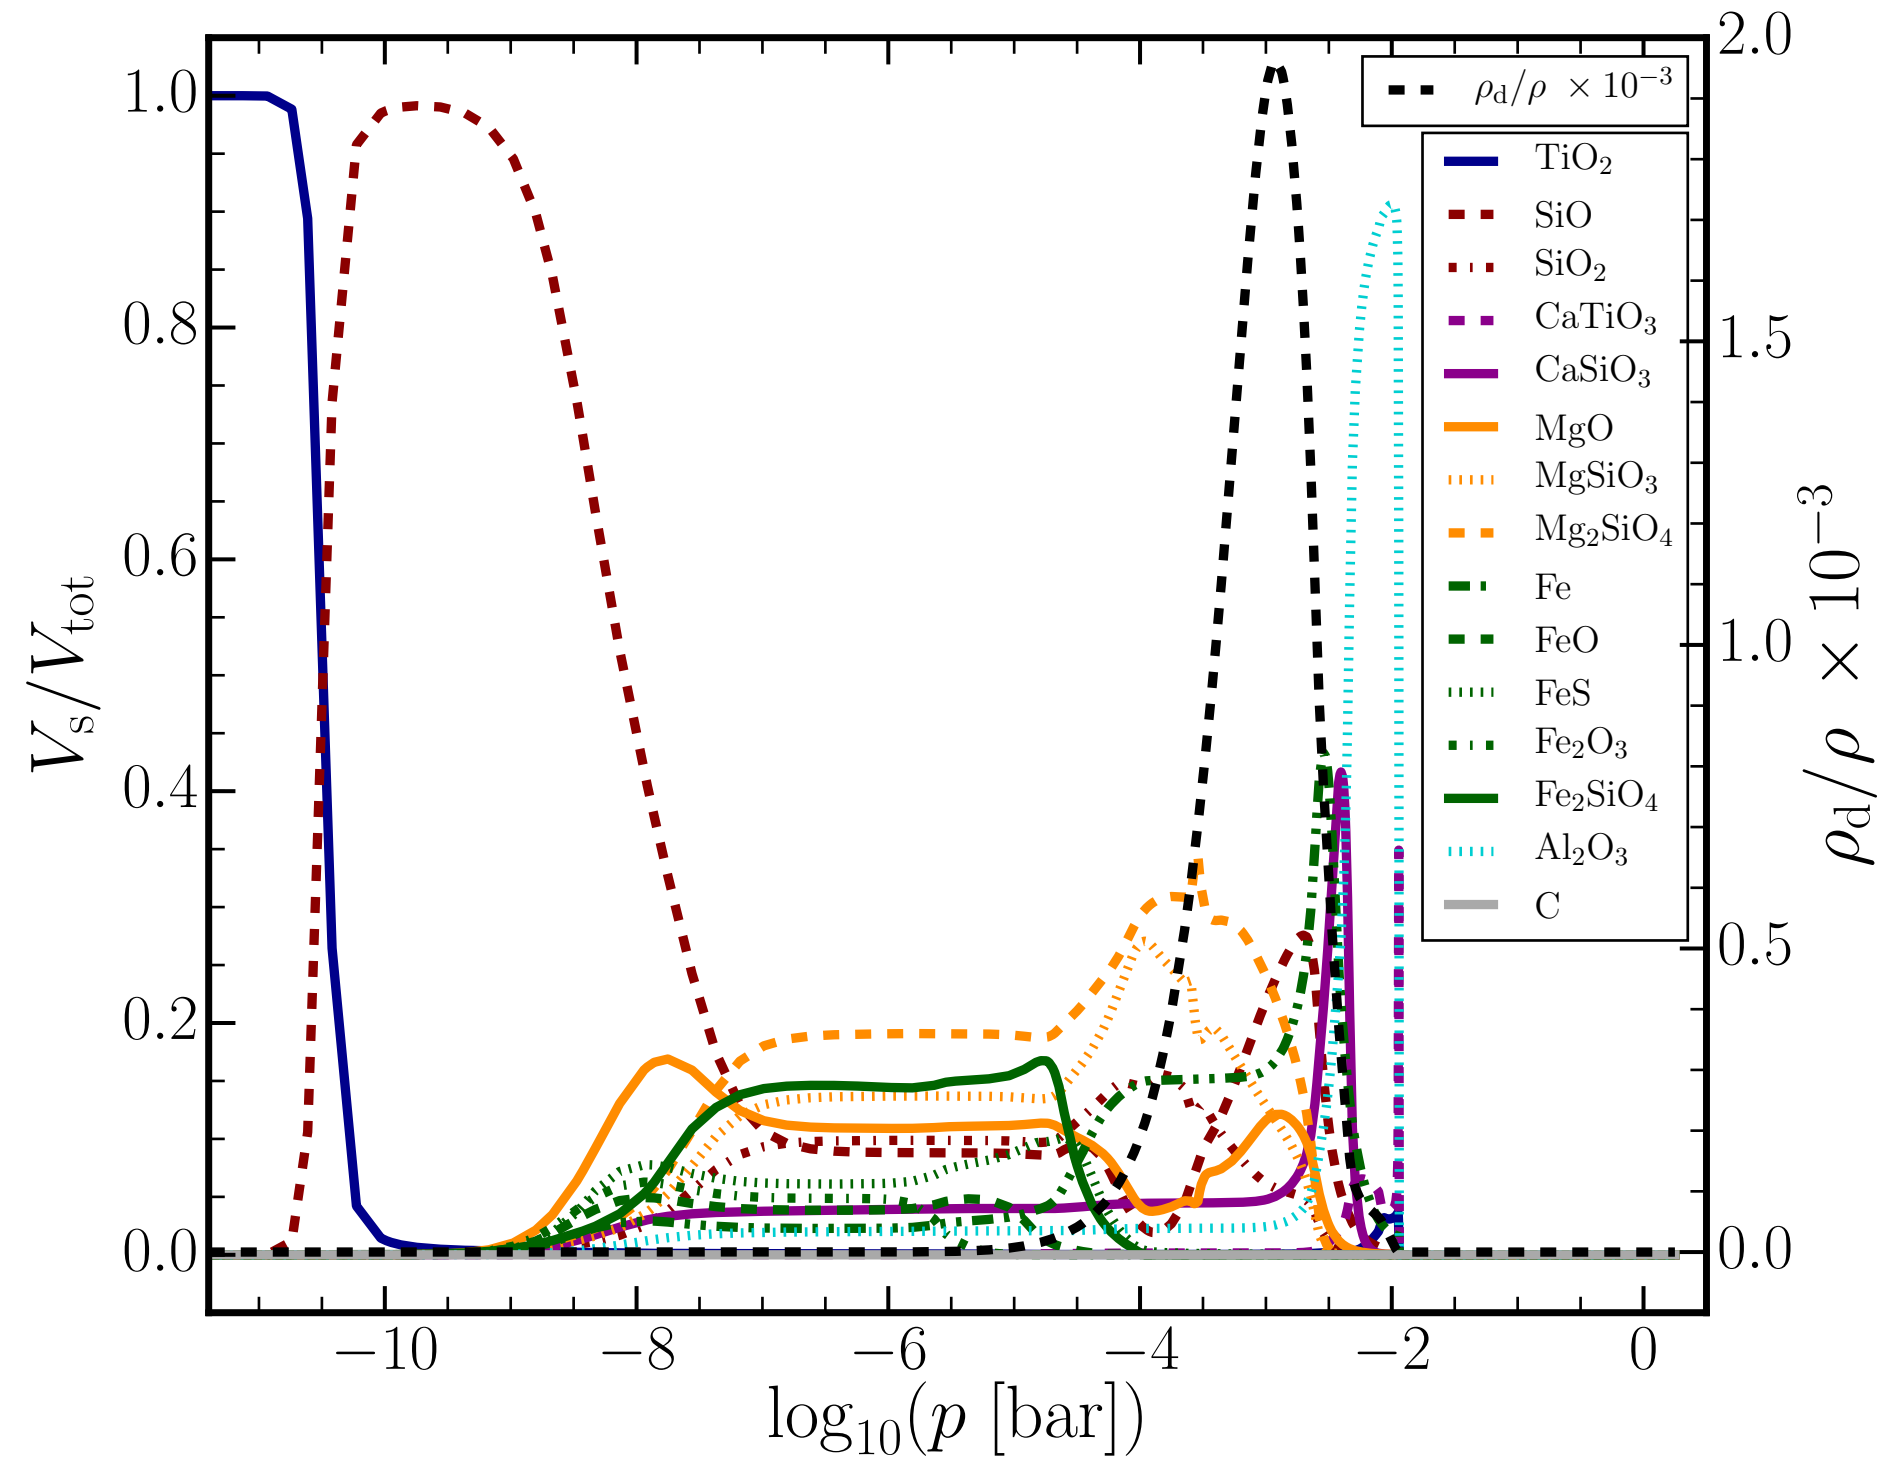

Supplement: Supplementary file 1 [file Material_Comp_Plots_LRGRTXT.pdf]
