# Supplementary material for: Mineral snowflakes on exoplanets and brown dwarfs: Effects of micro-porosity, size distributions, and particle shape
Source: arXiv:2004.13502 source file (2020-04-28)

$T_{\text{eff}} = 1200 \text{ K}, \log(g) = 3.0$

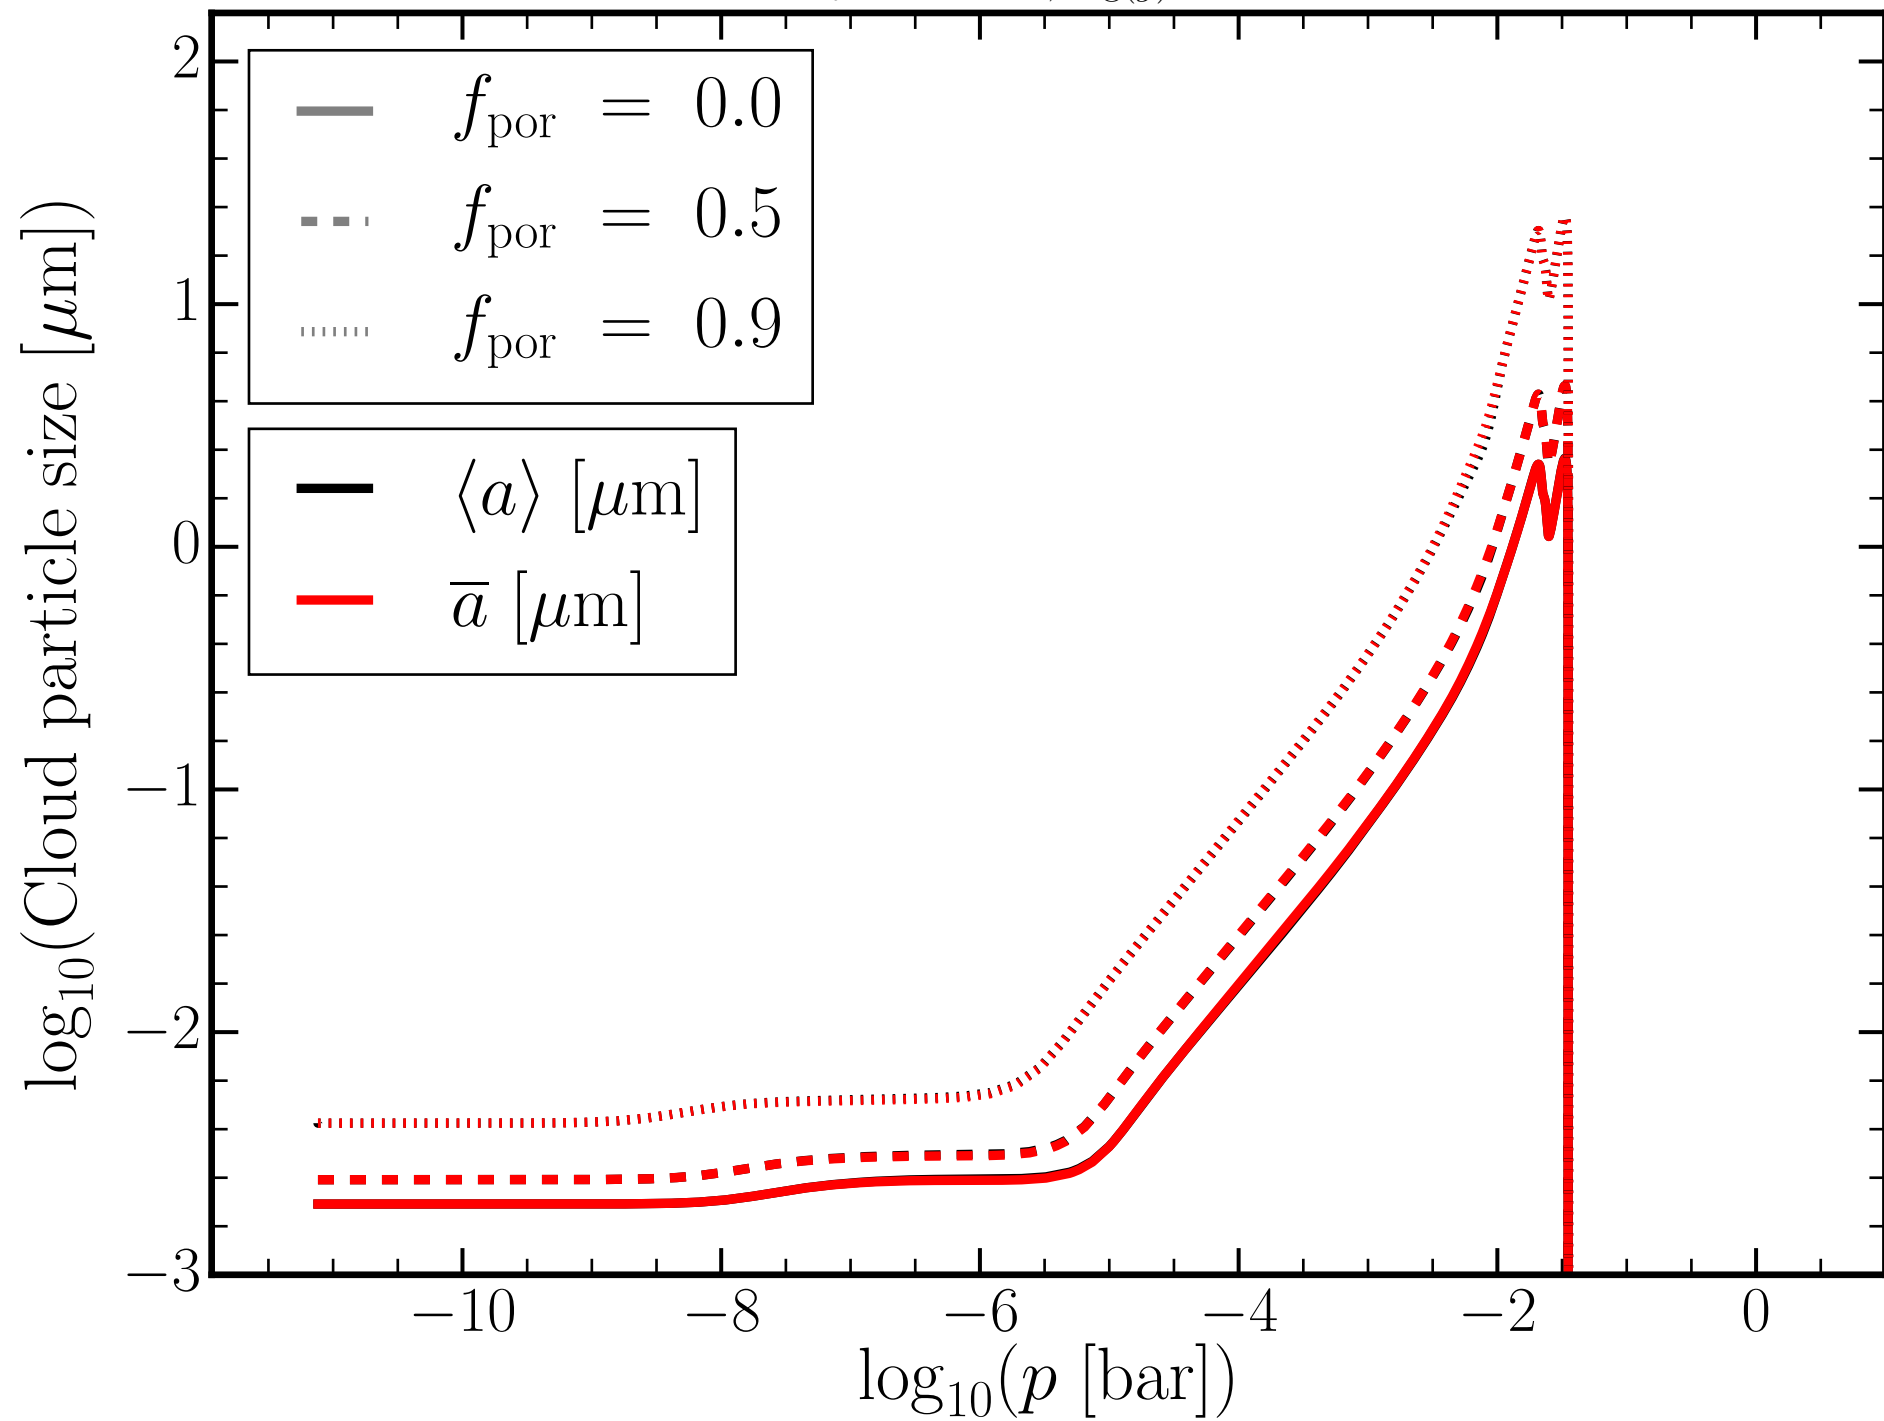

$T_{\text{eff}} = 1200 \text{ K}, \log(g) = 3.0$

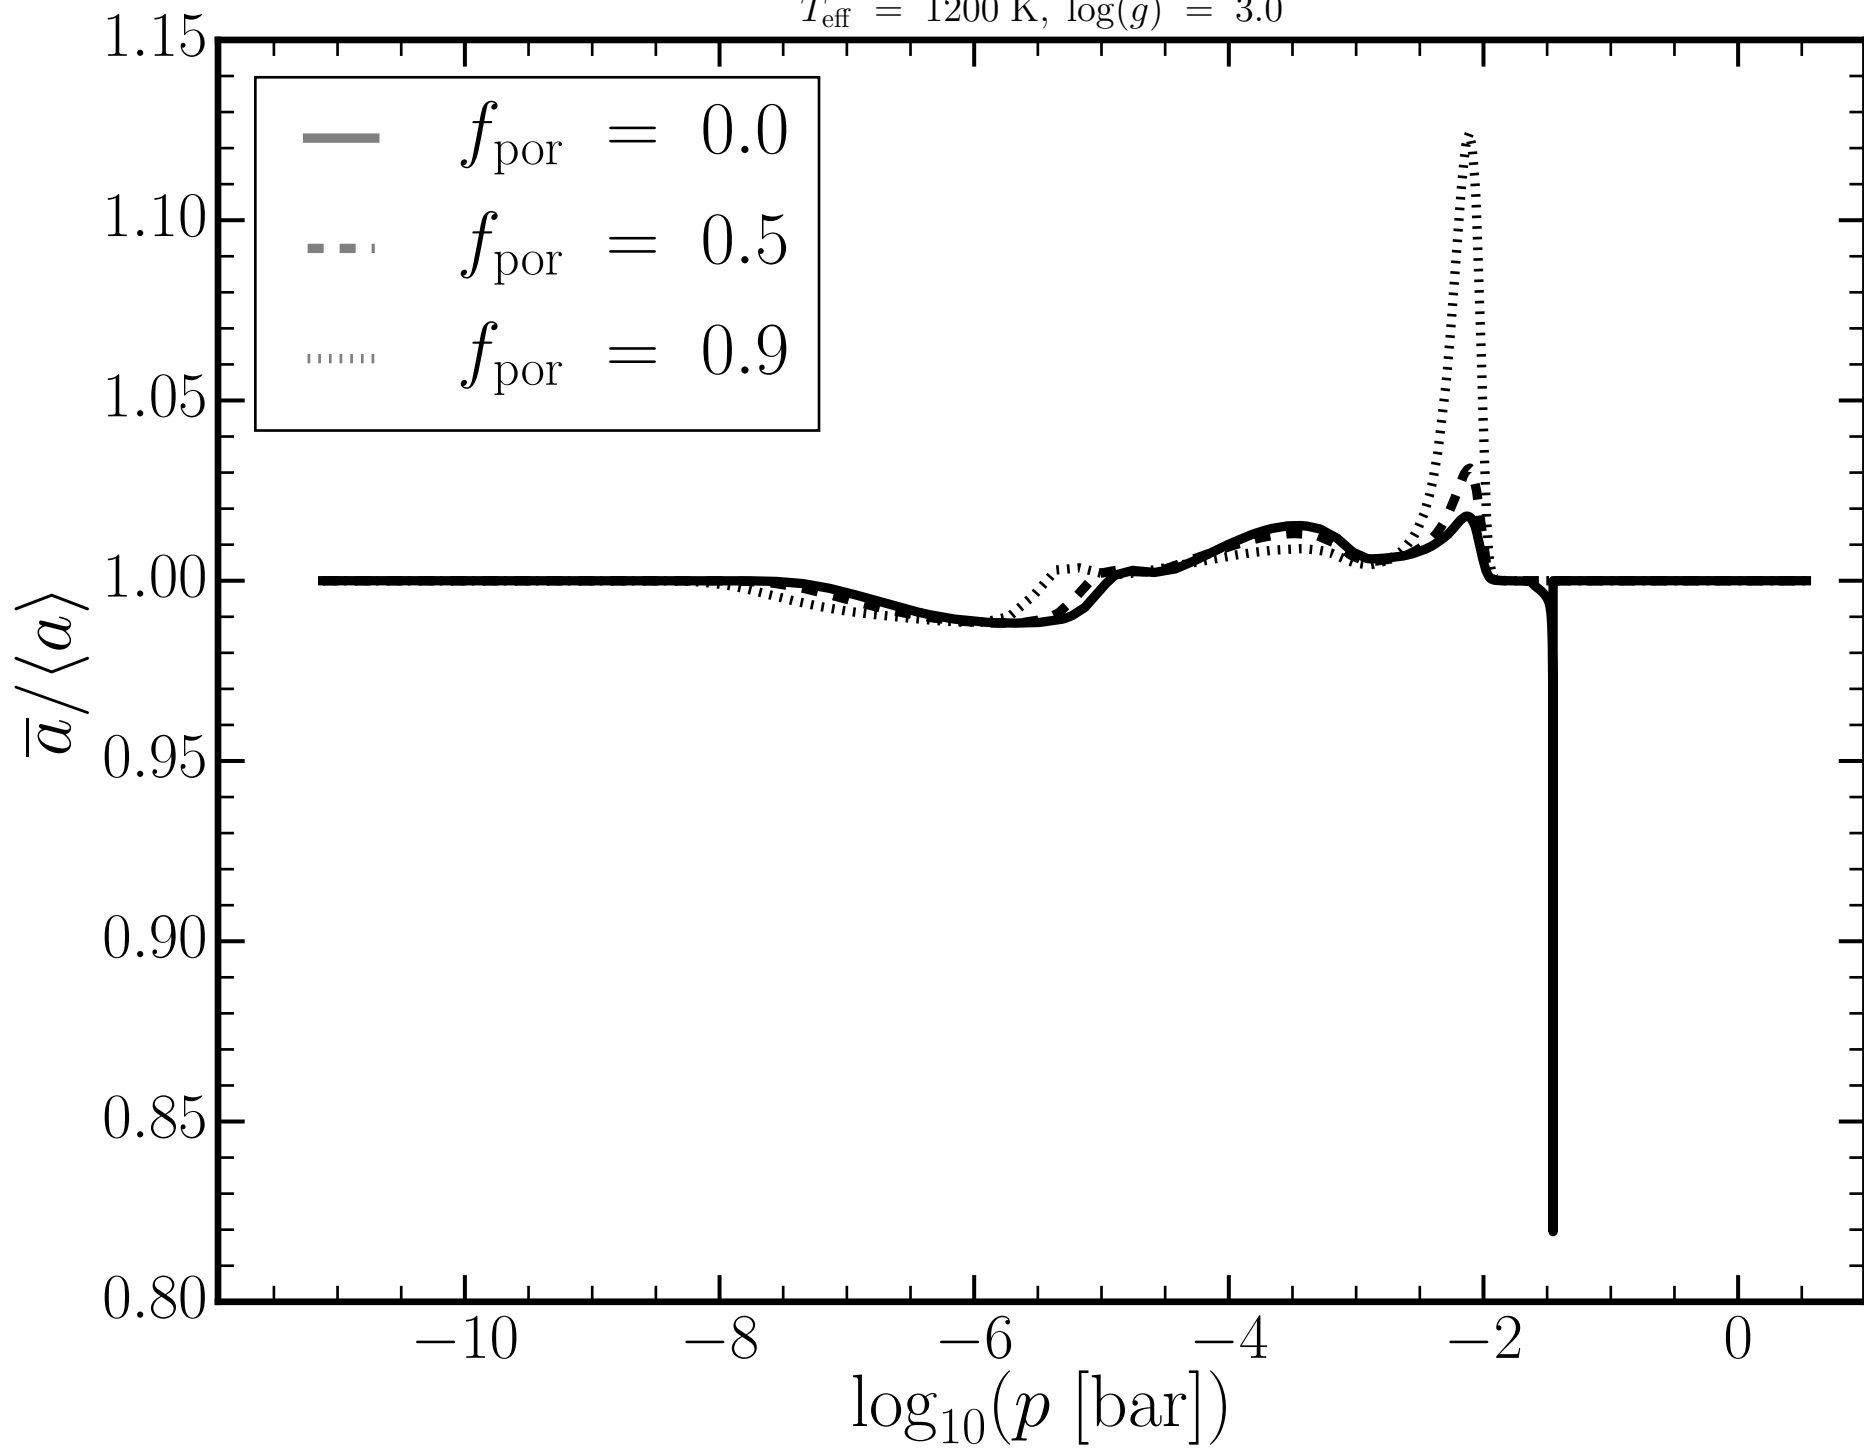

$T_{\text{eff}} = 1200 \text{ K}, \log(g) = 5.0$

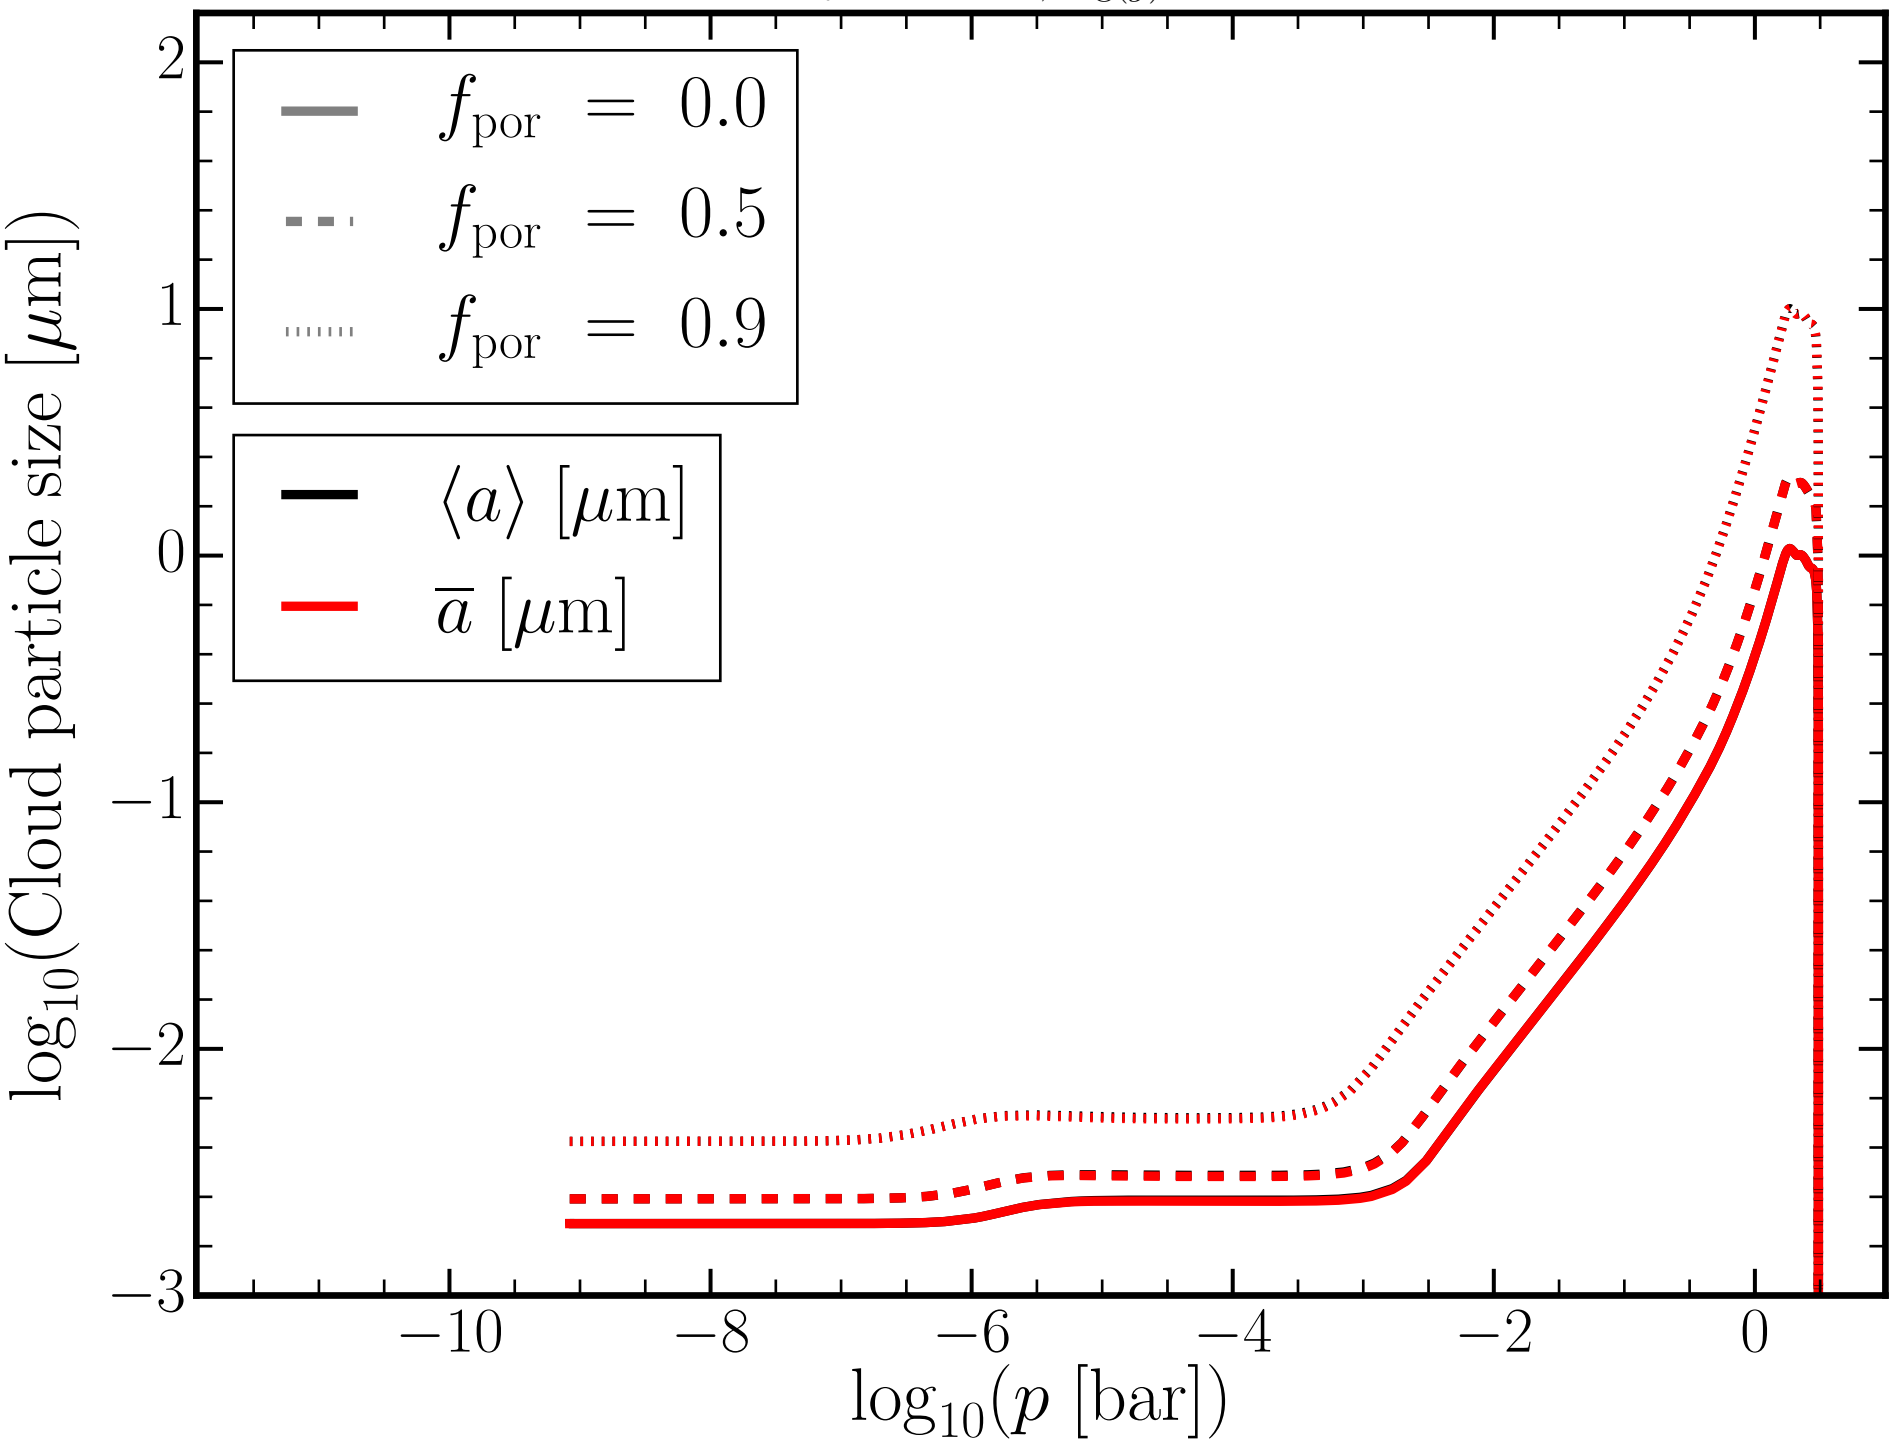

$T_{\text{eff}} = 1200 \text{ K}, \log(g) = 5.0$

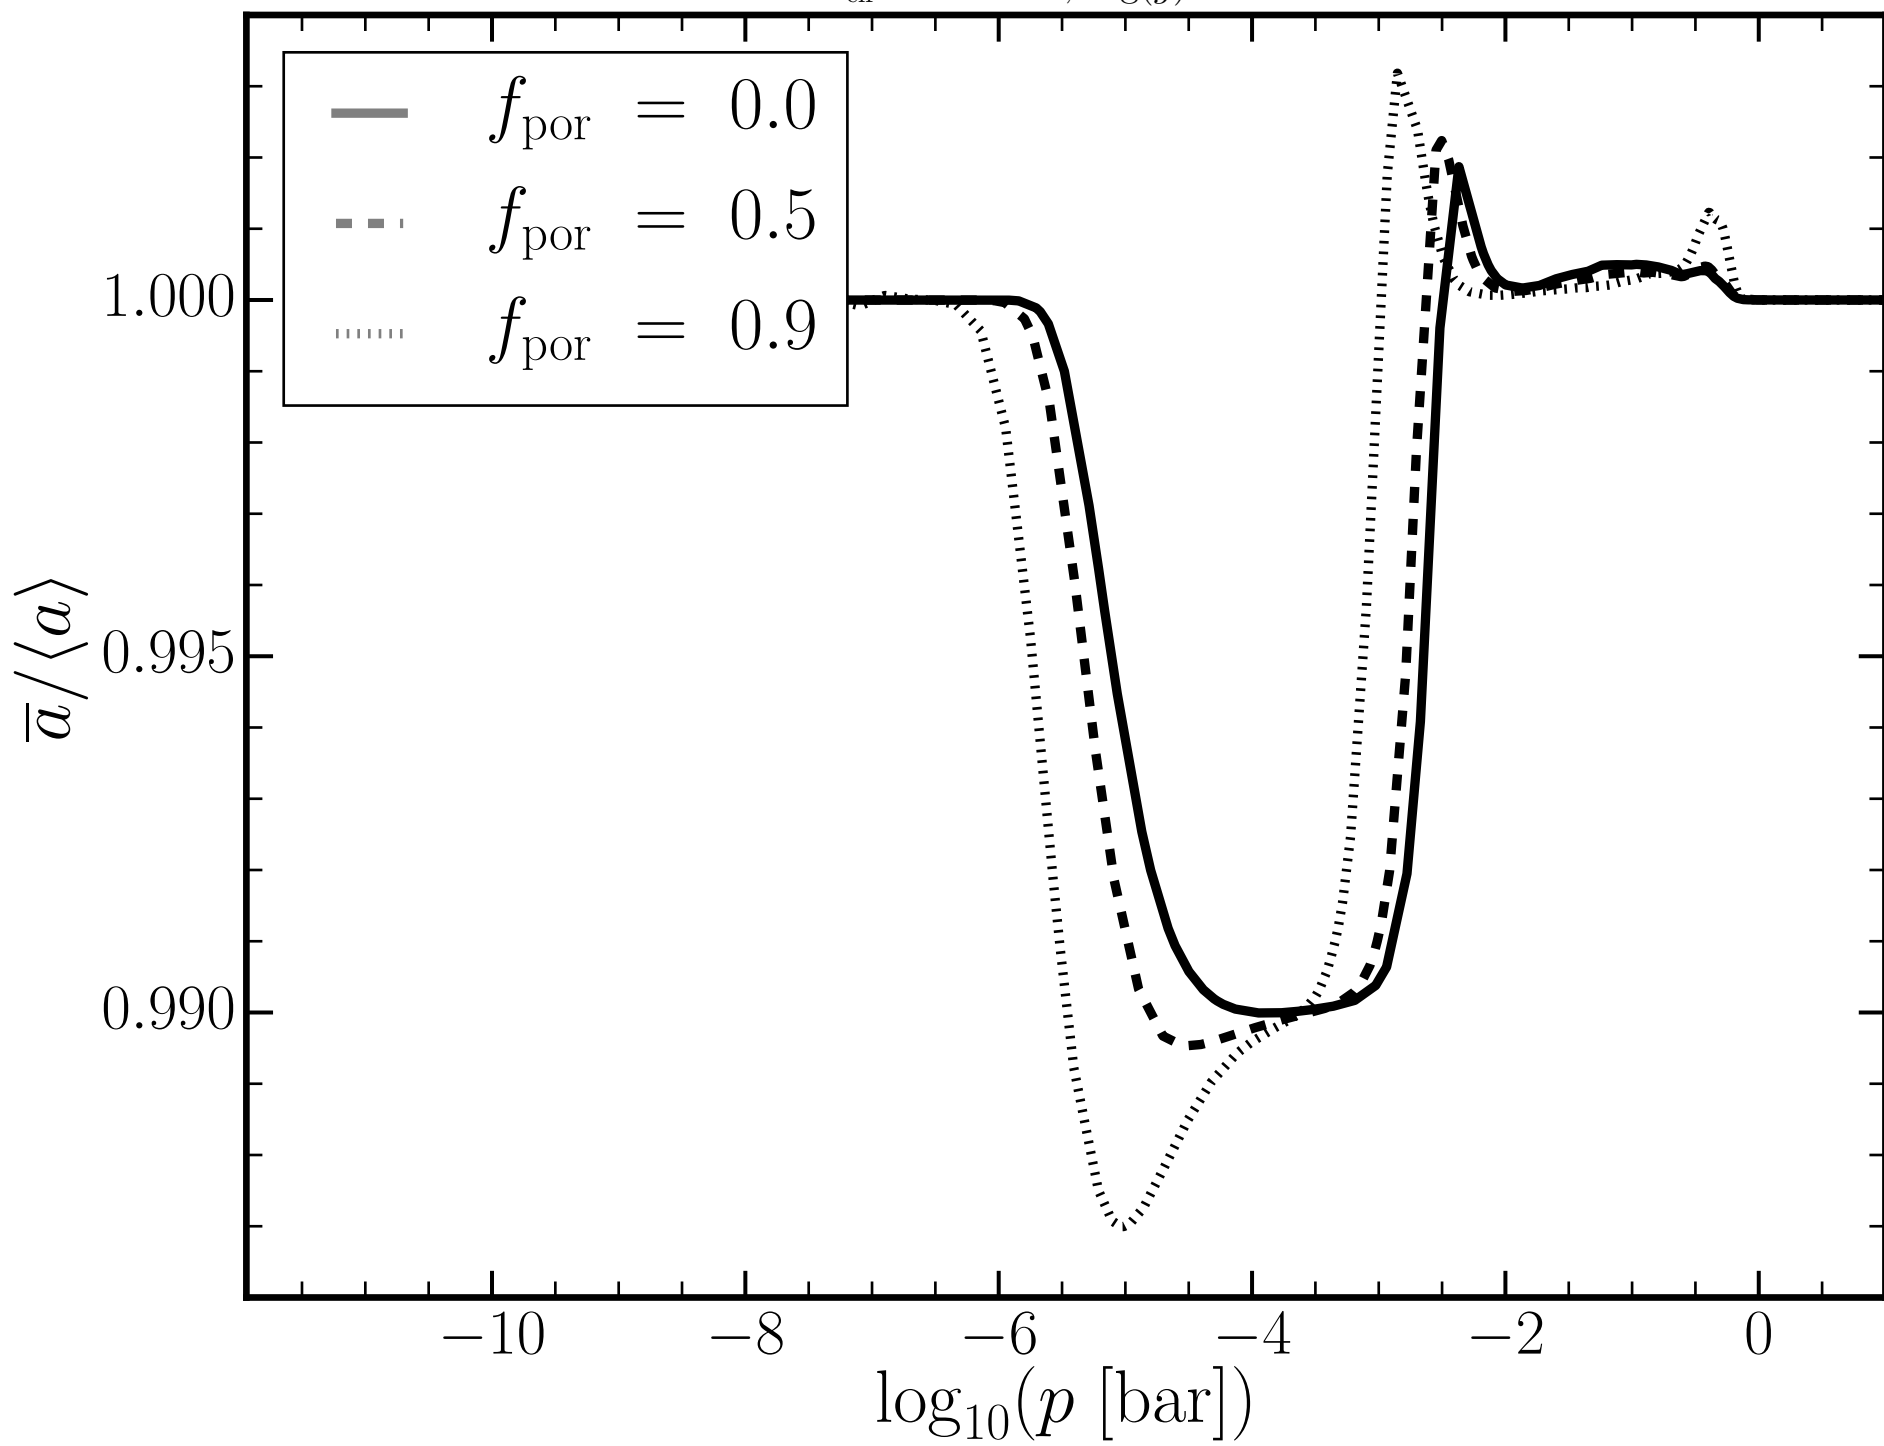

$T_{\text{eff}} = 1800 \text{ K}, \log(g) = 3.0$

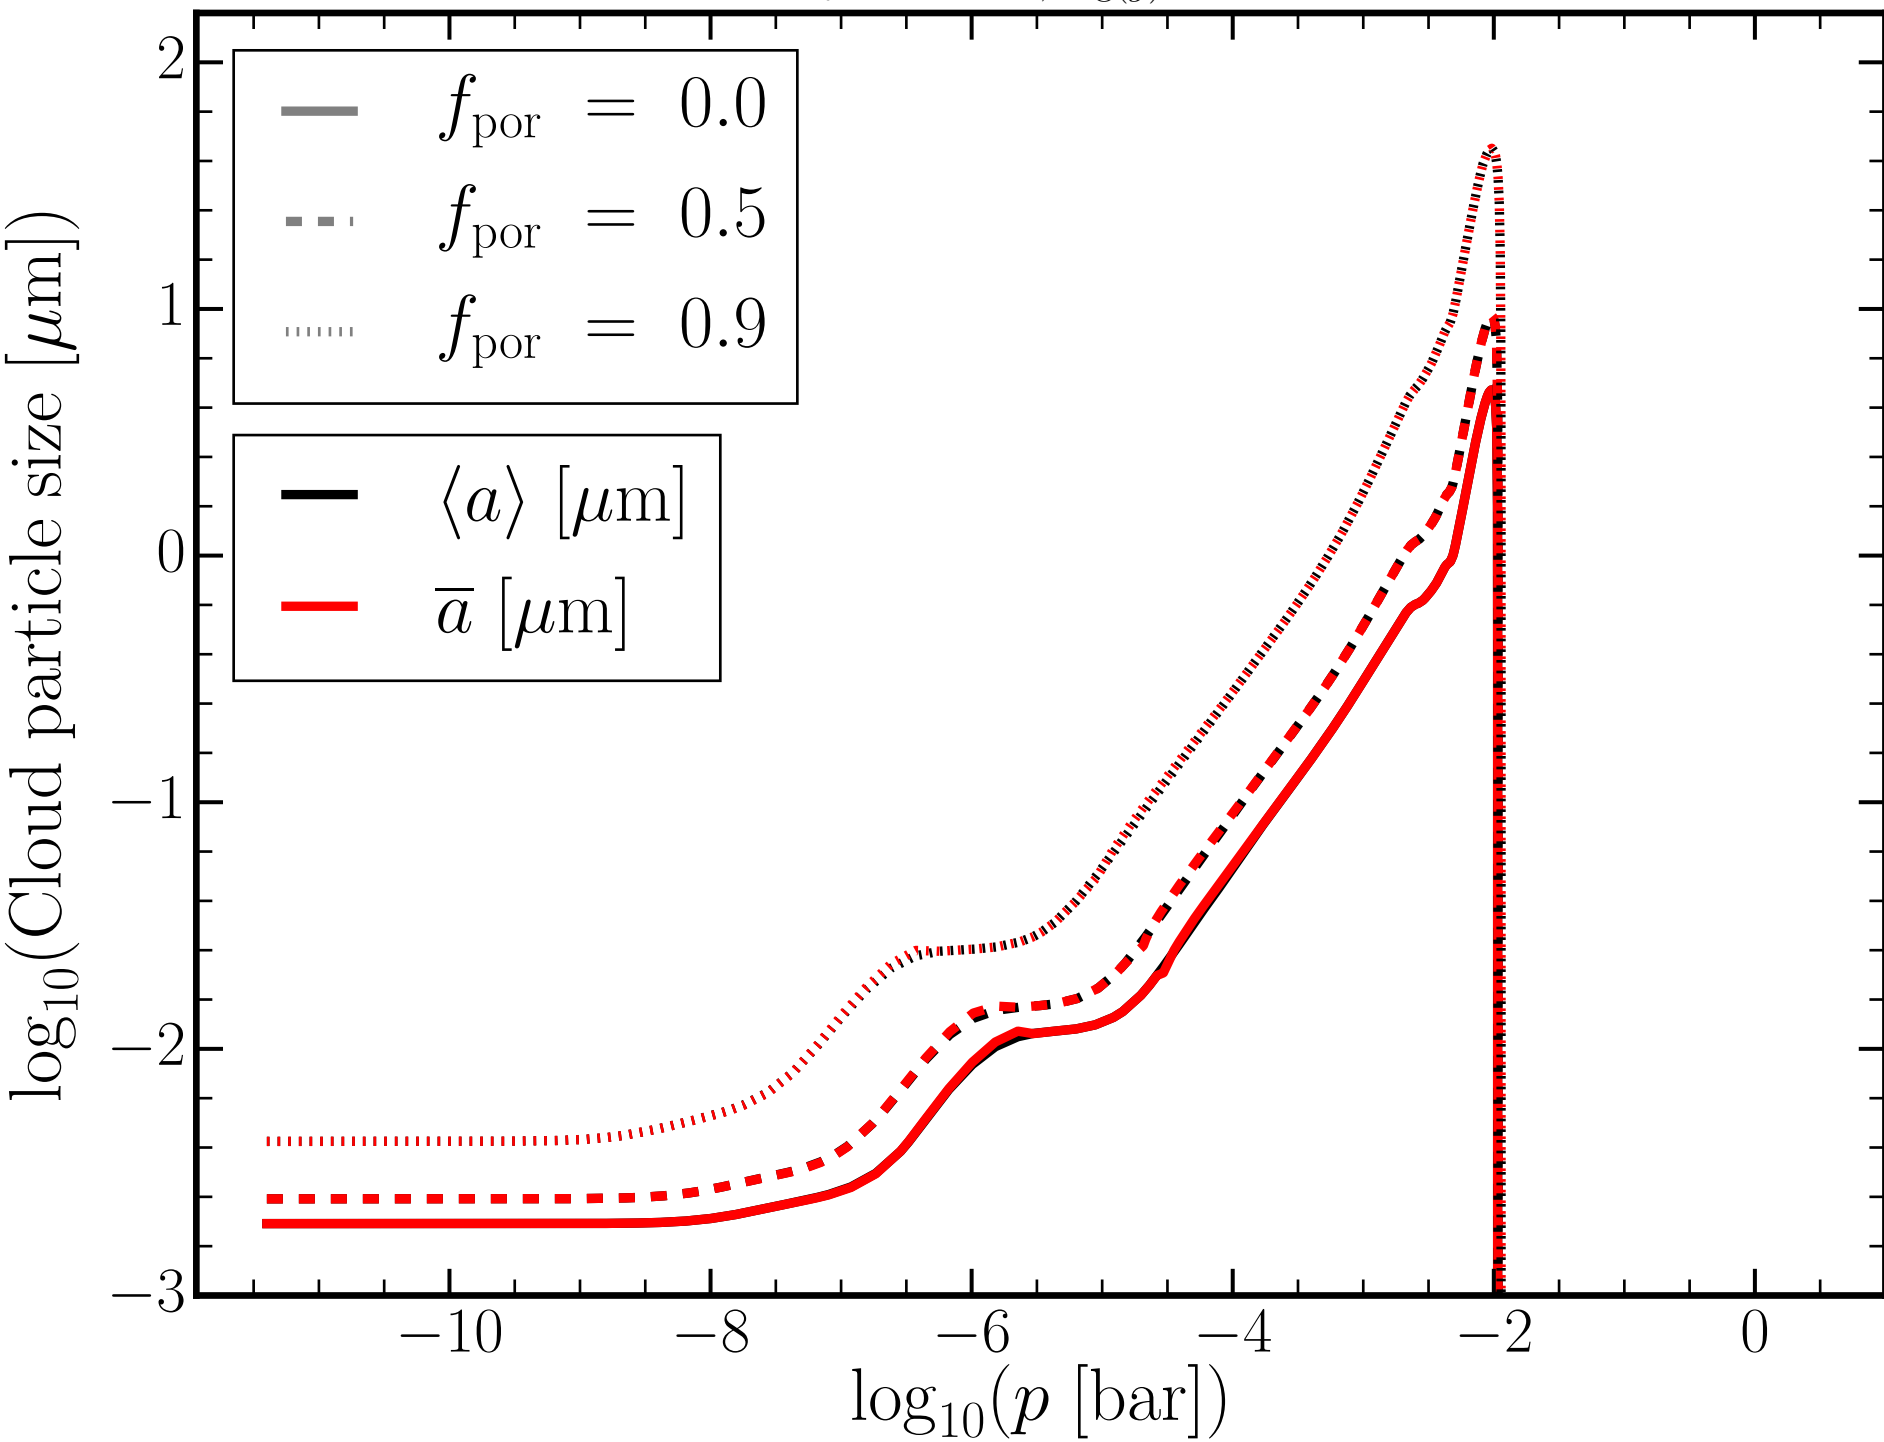

$T_{\text{eff}} = 1800 \text{ K}, \log(g) = 3.0$

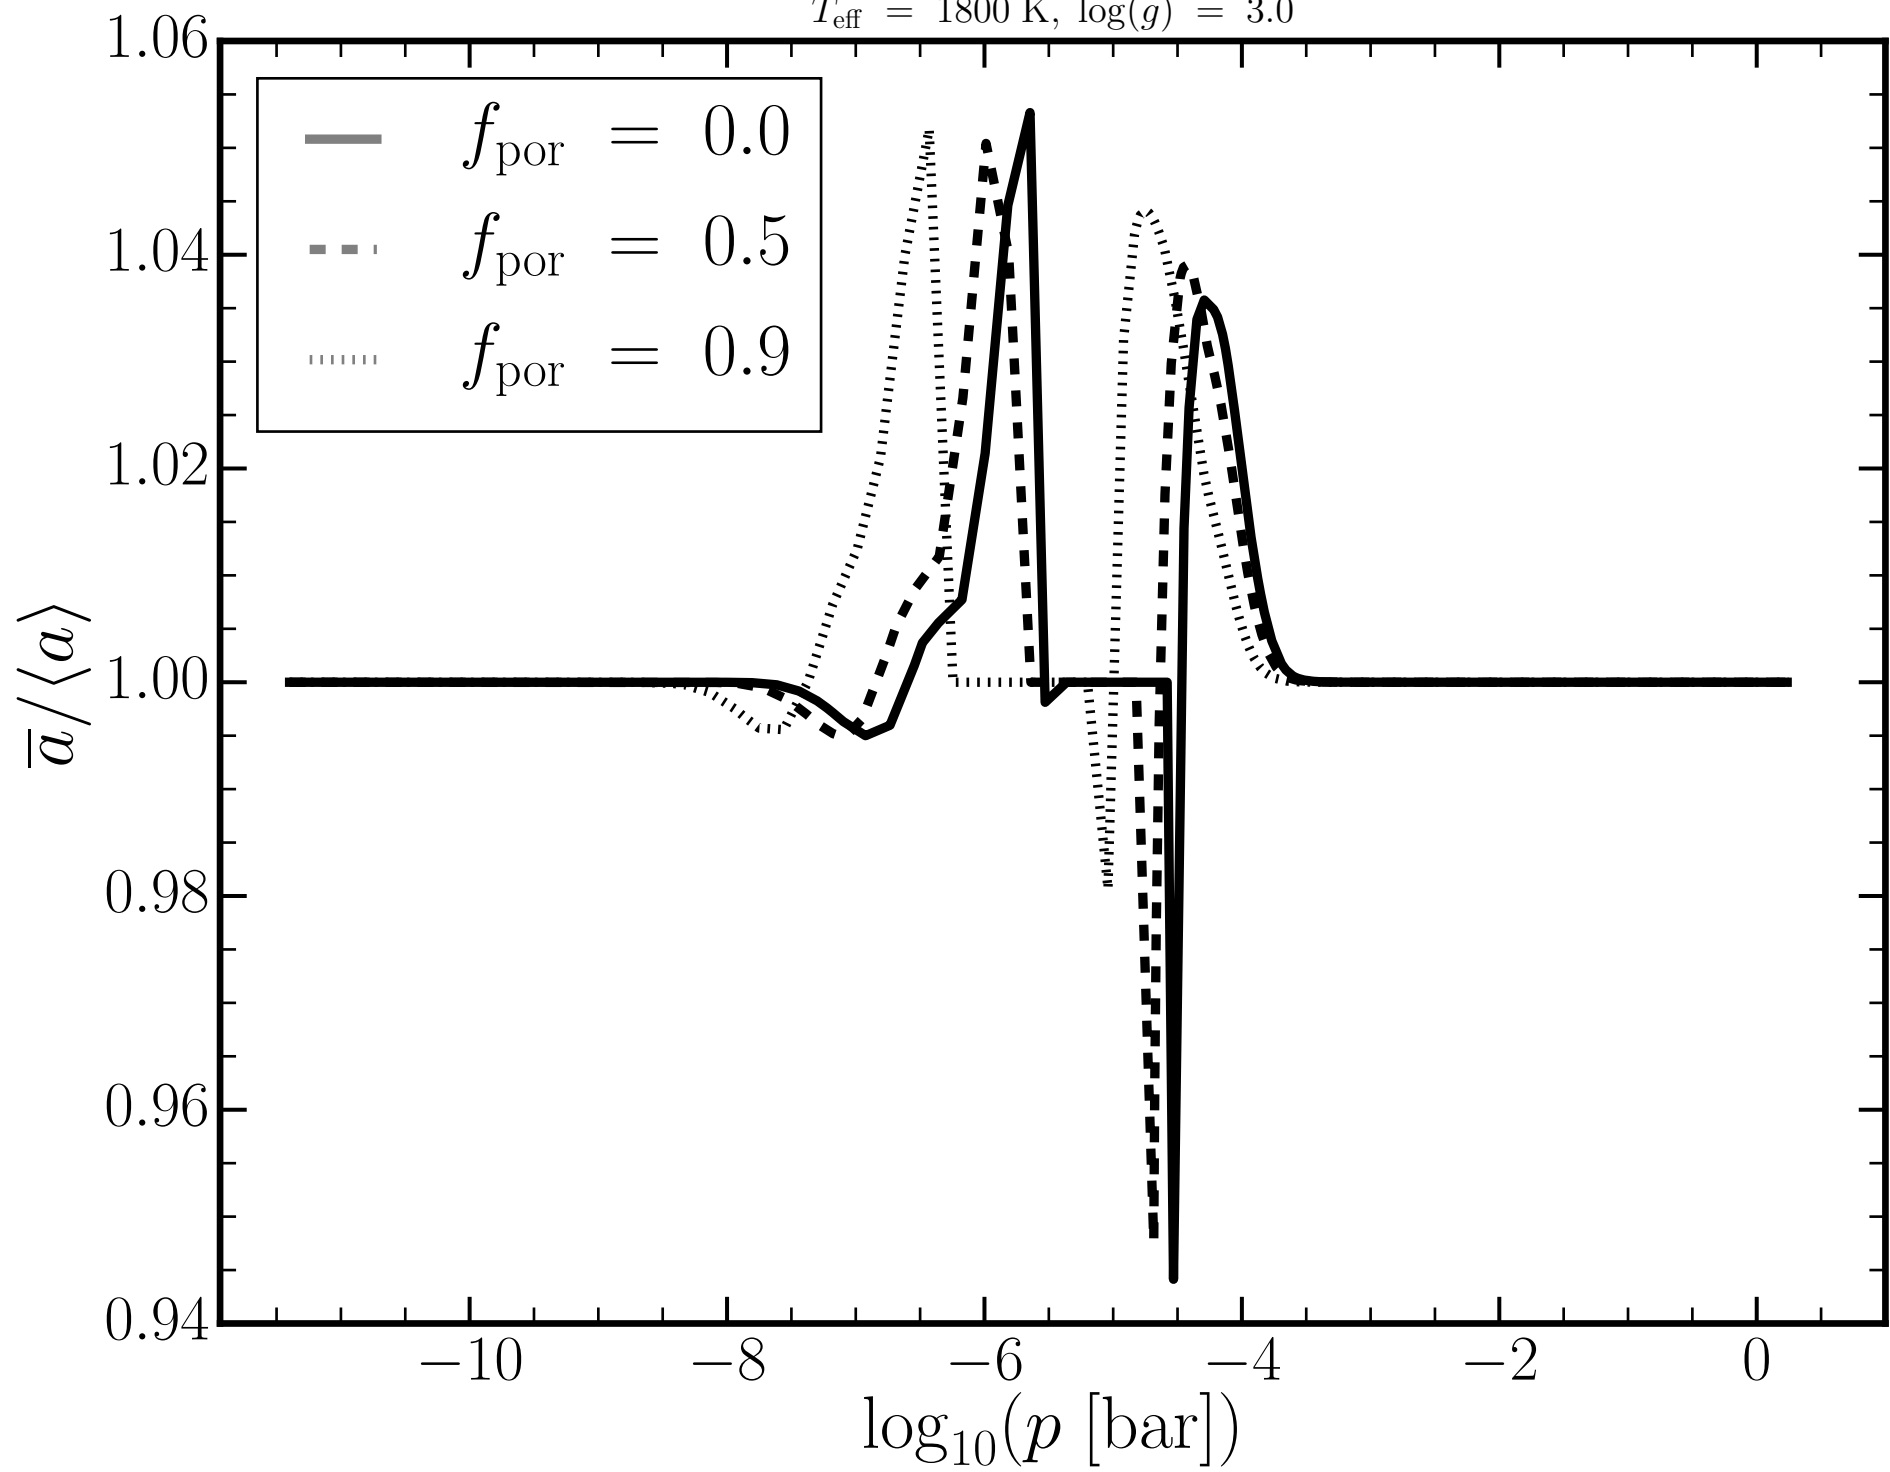

$T_{\text{eff}} = 1800 \text{ K}, \log(g) = 5.0$

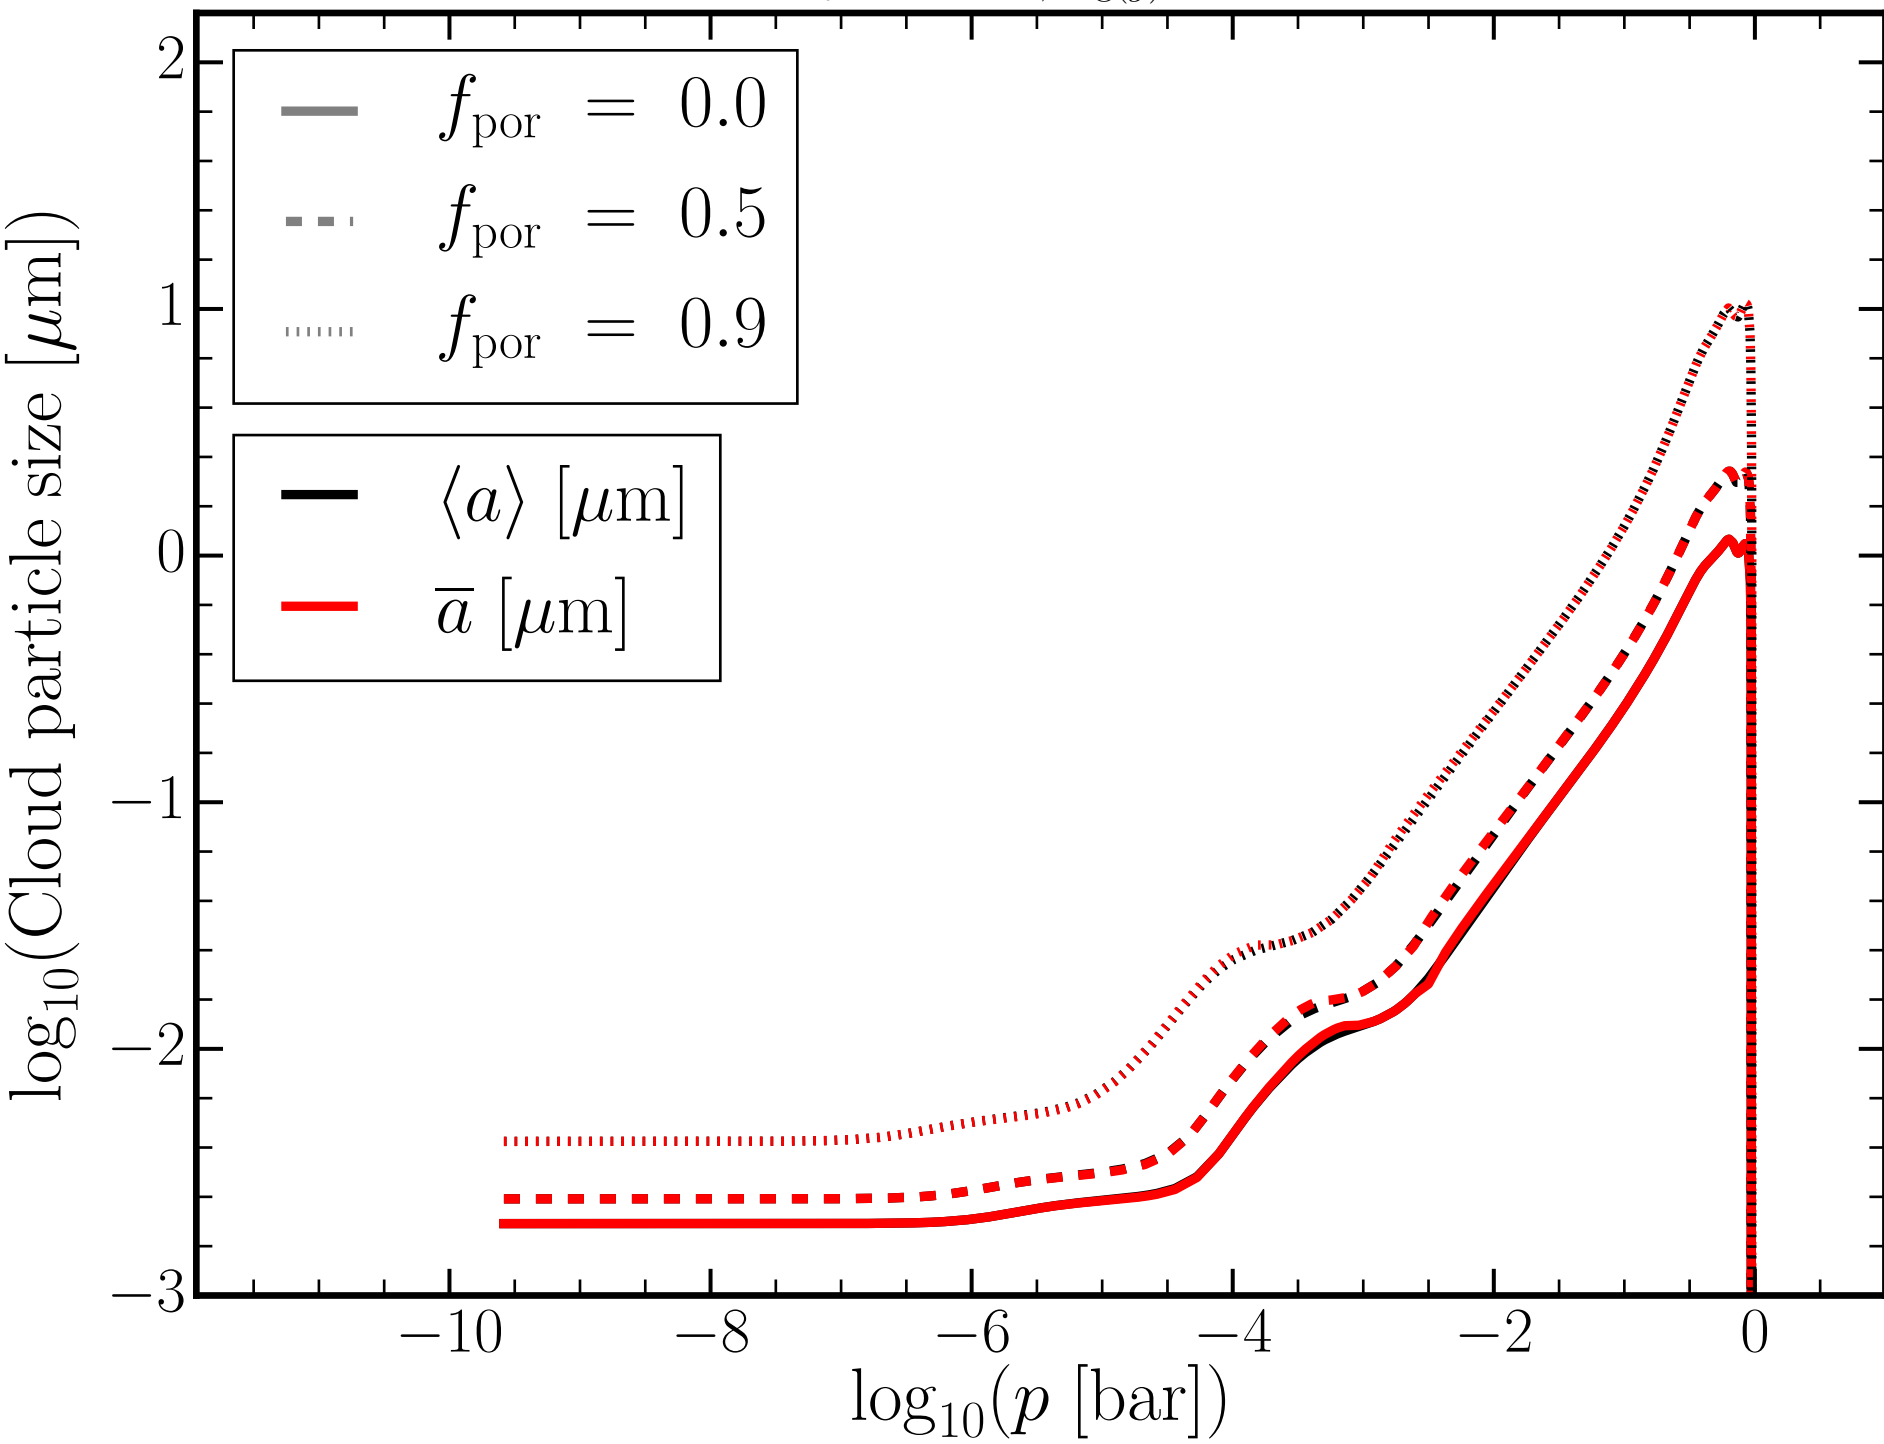

$T_{\text{eff}} = 1800 \text{ K}, \log(g) = 5.0$

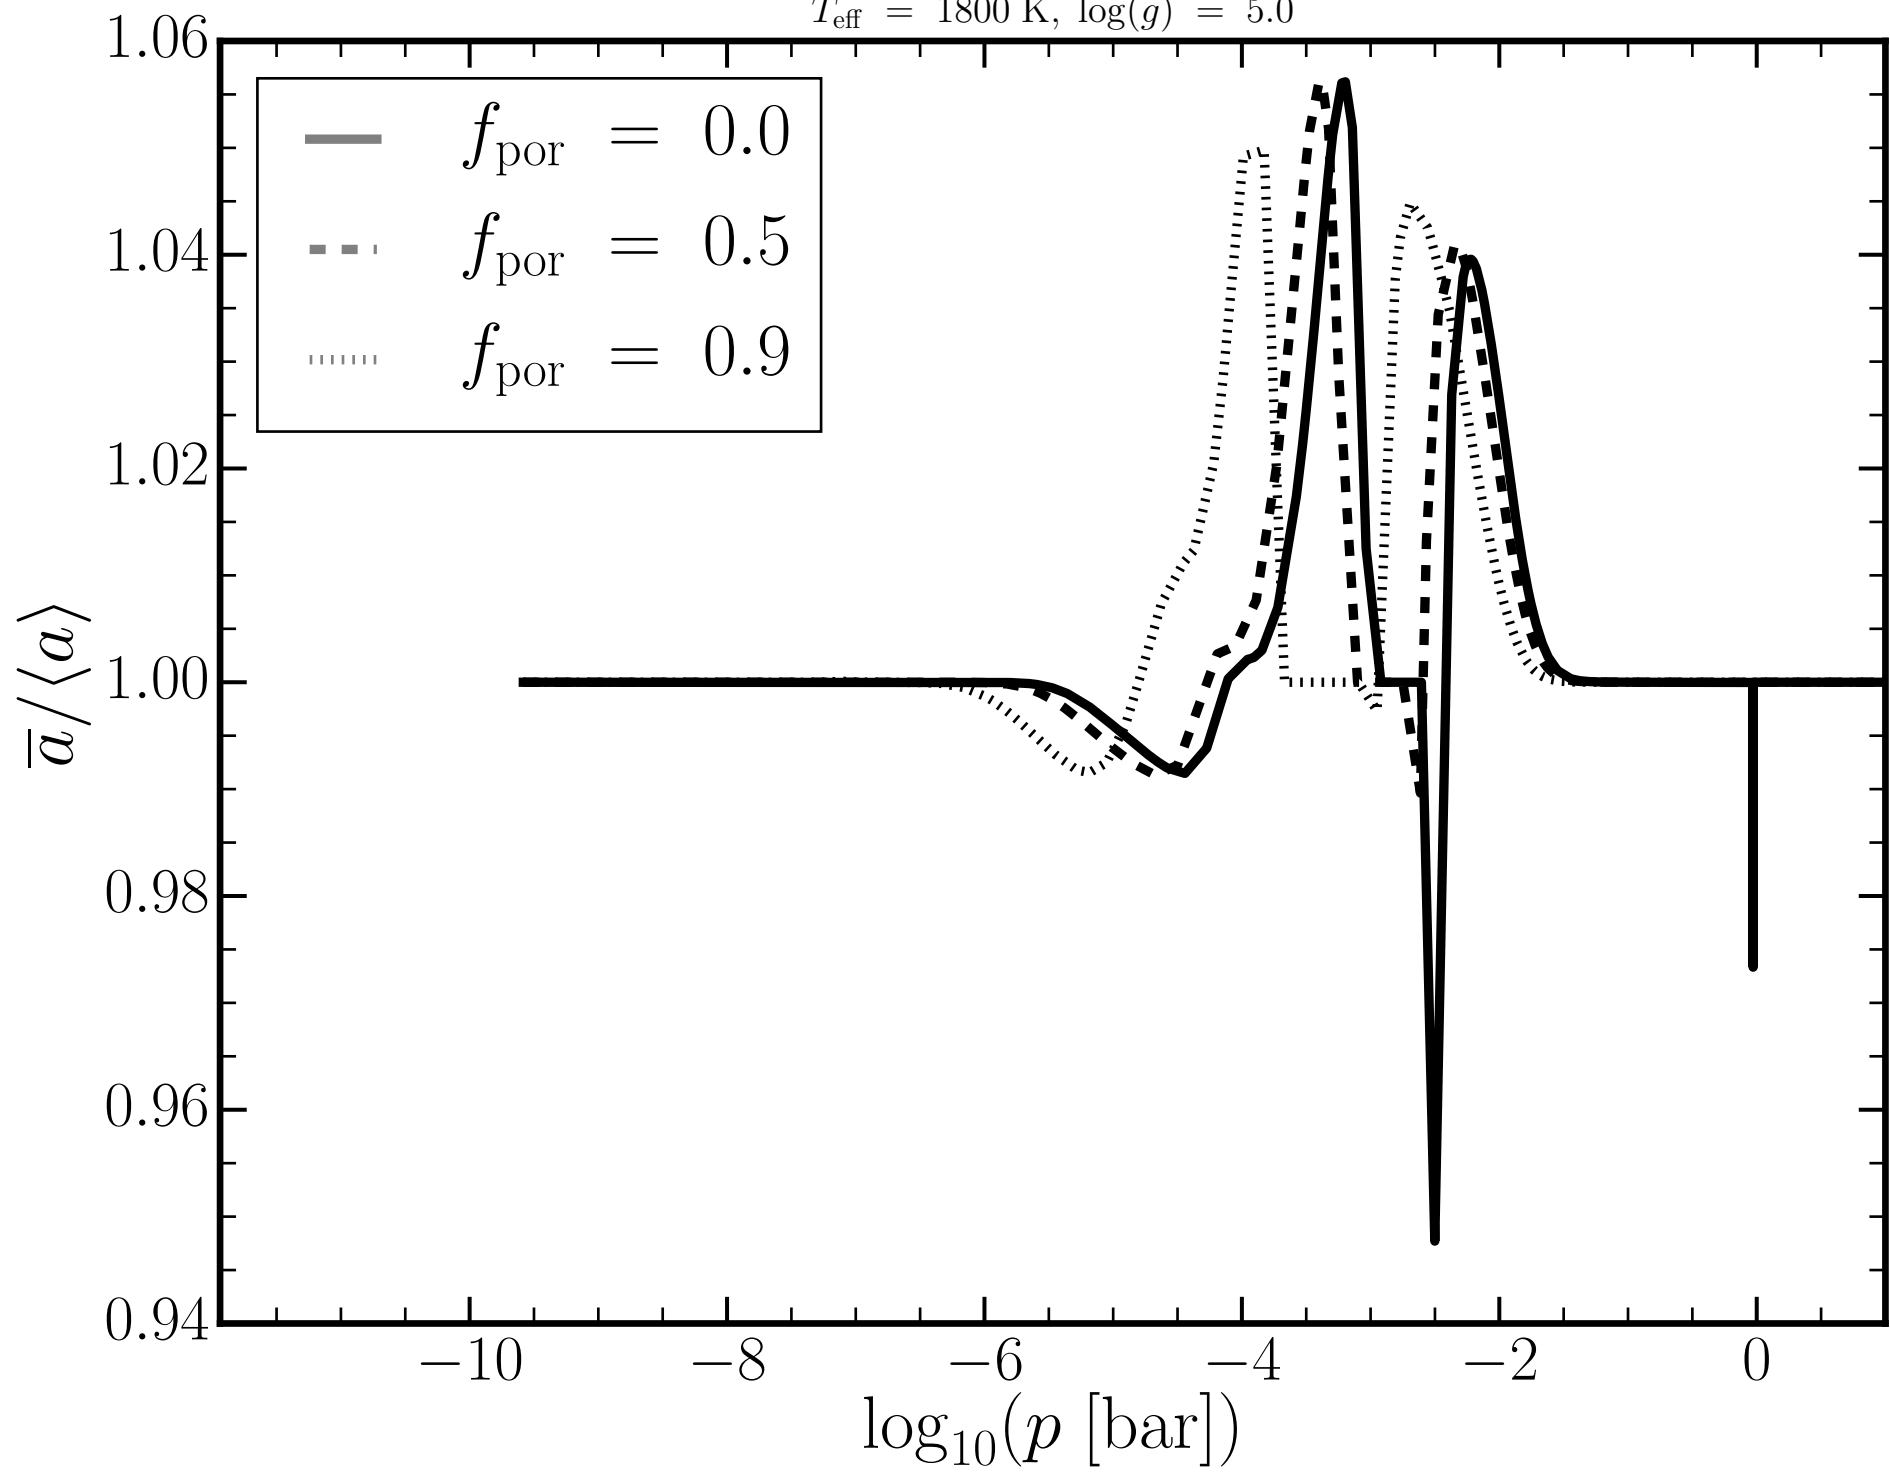



$T_{\text{eff}} = 2400 \text{ K}, \log(g) = 3.0$

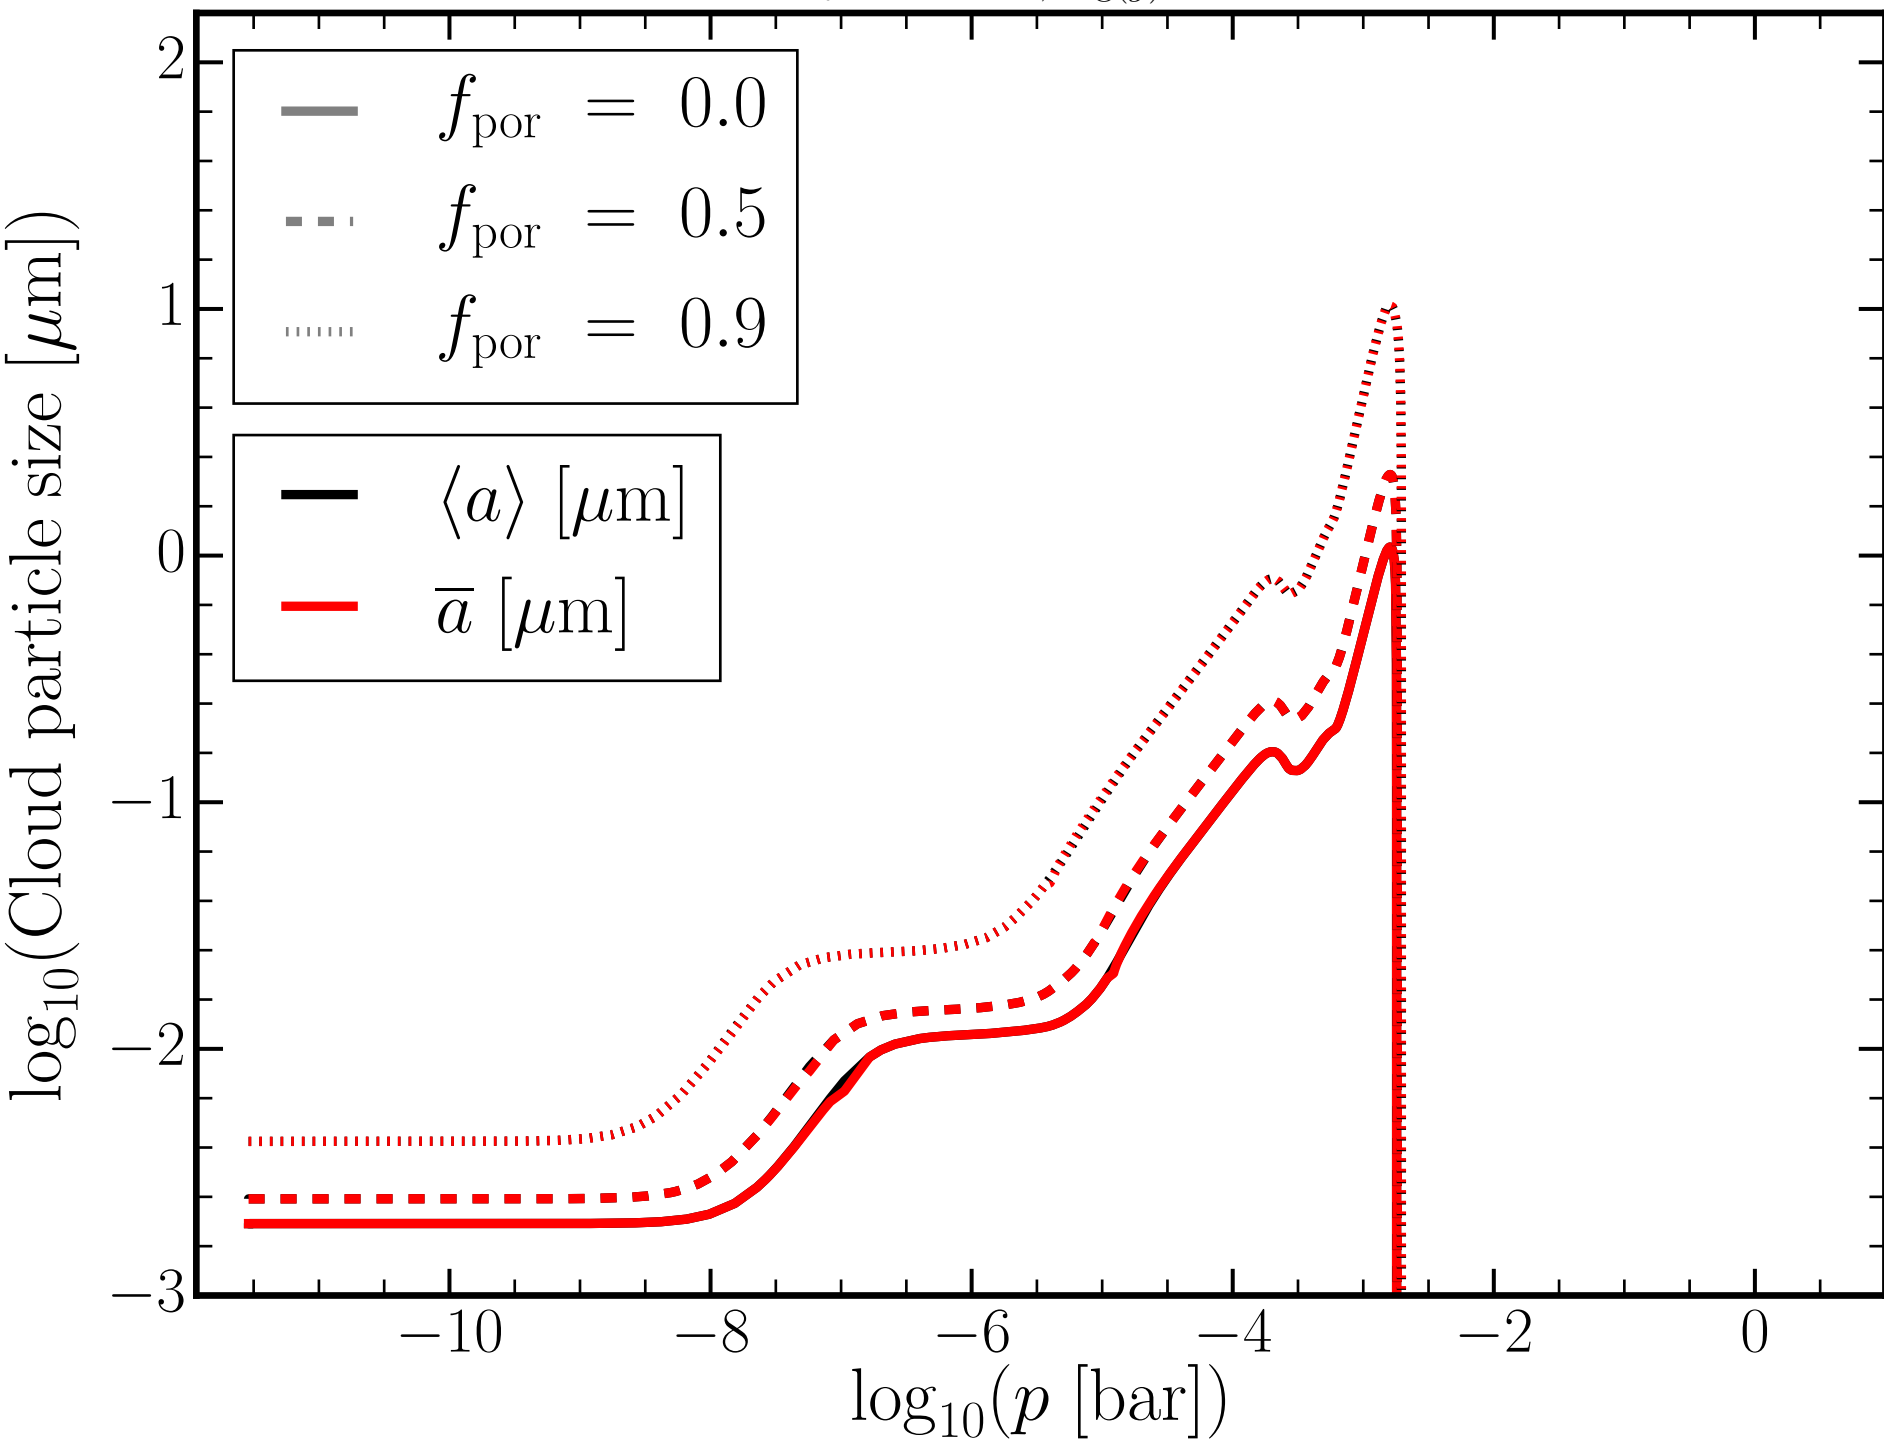

$T_{\text{eff}} = 2400 \text{ K}, \log(g) = 3.0$

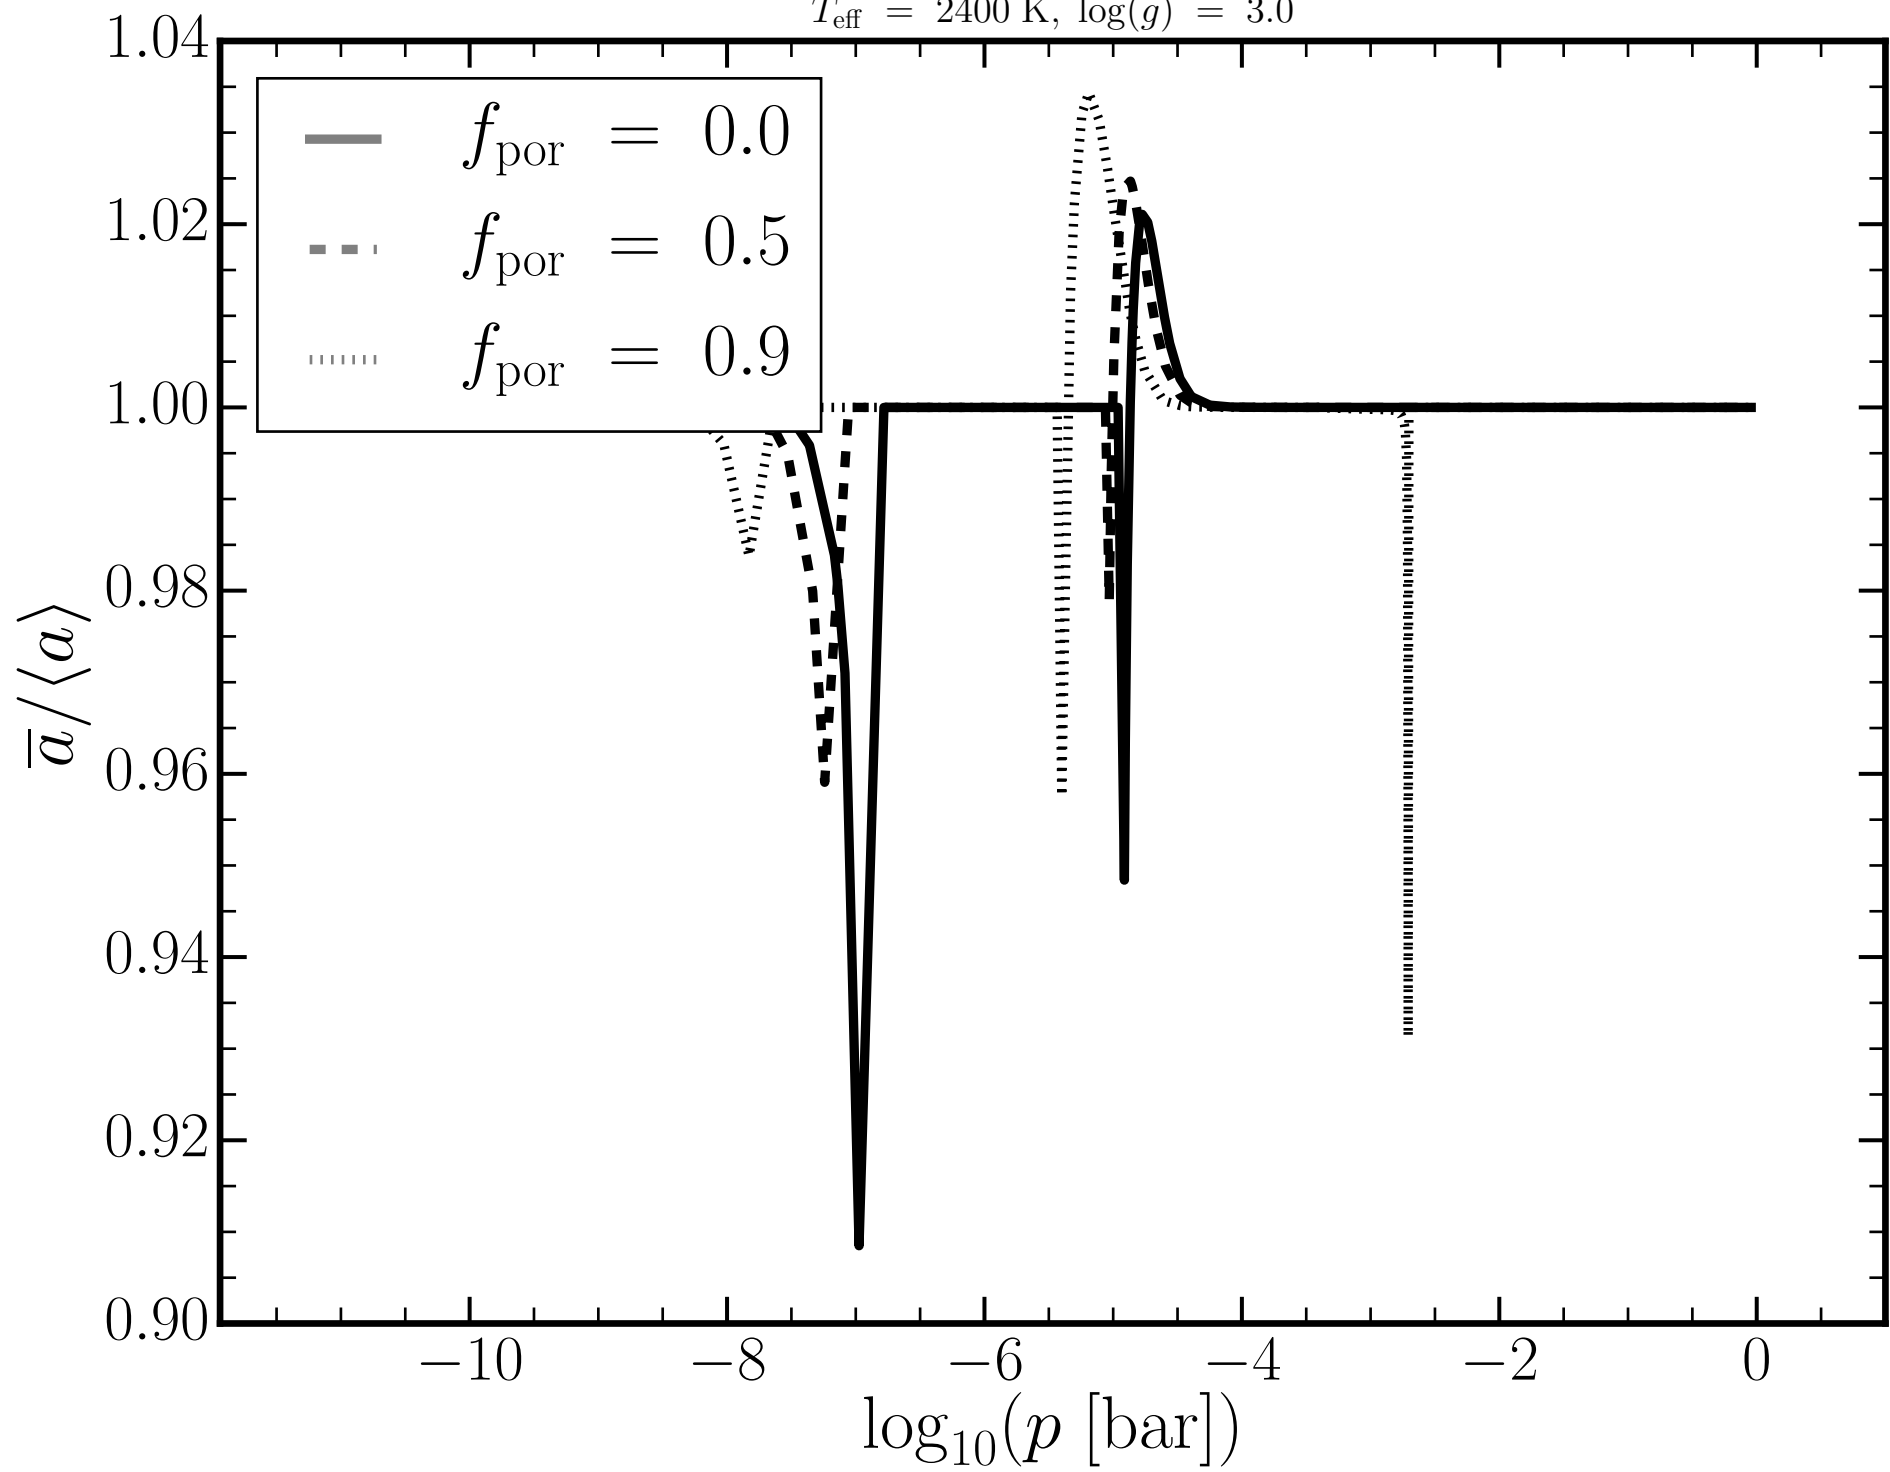



$T_{\text{eff}} = 2400 \text{ K}, \log(g) = 5.0$

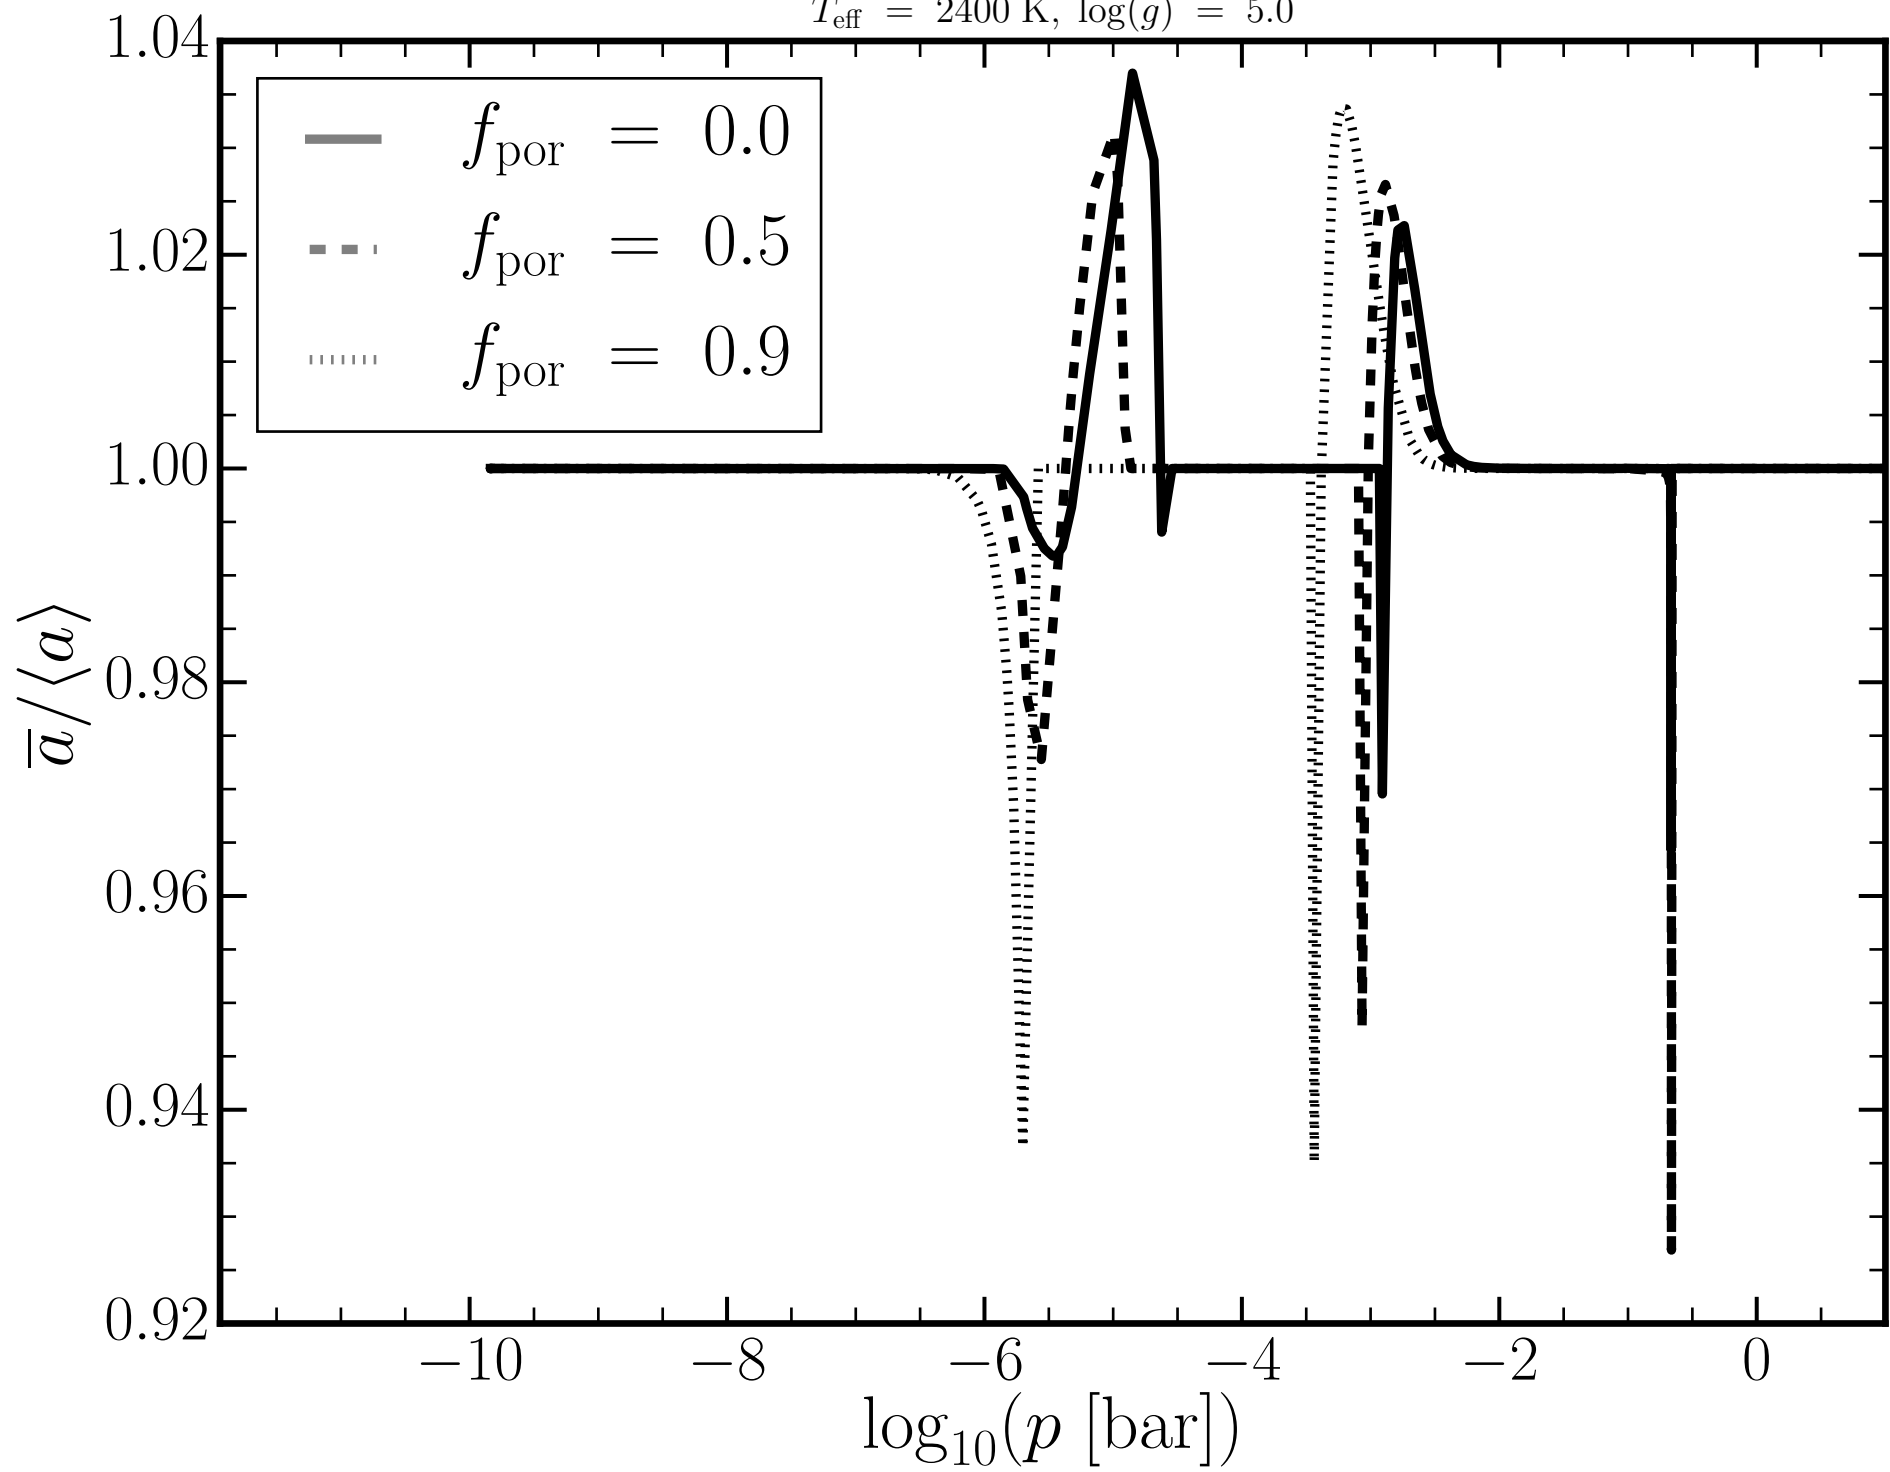

Supplement: Supplementary file 2 [file Radii_Comparison_LRGRTXT.pdf]
