# Supplementary material for: Mineral snowflakes on exoplanets and brown dwarfs: Effects of micro-porosity, size distributions, and particle shape
Source: arXiv:2004.13502 source file (2020-04-28)

TiO<sub>2</sub>[s]

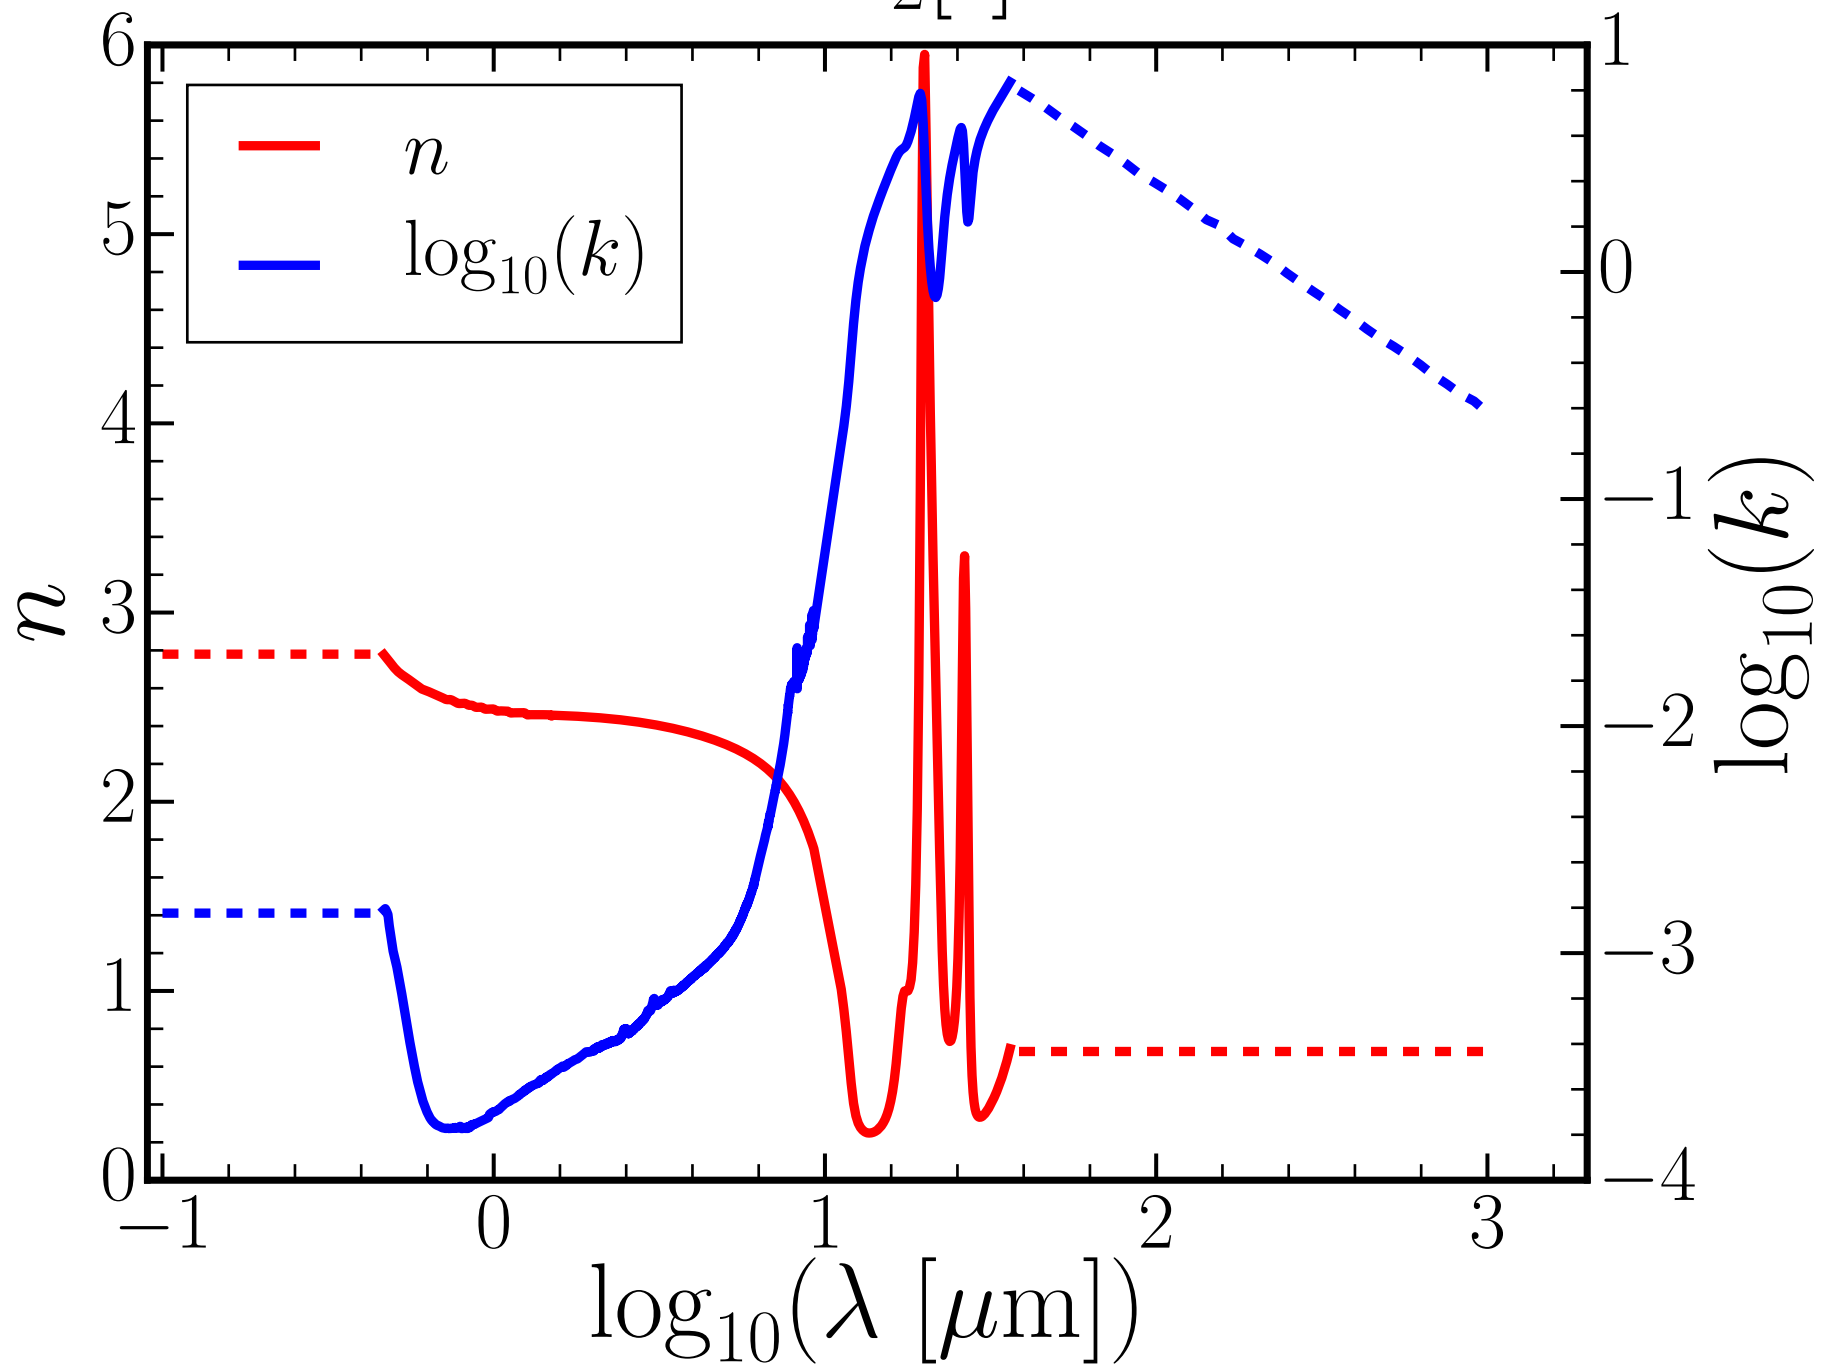

$\text{Mg}_2\text{SiO}_4[\text{s}]$

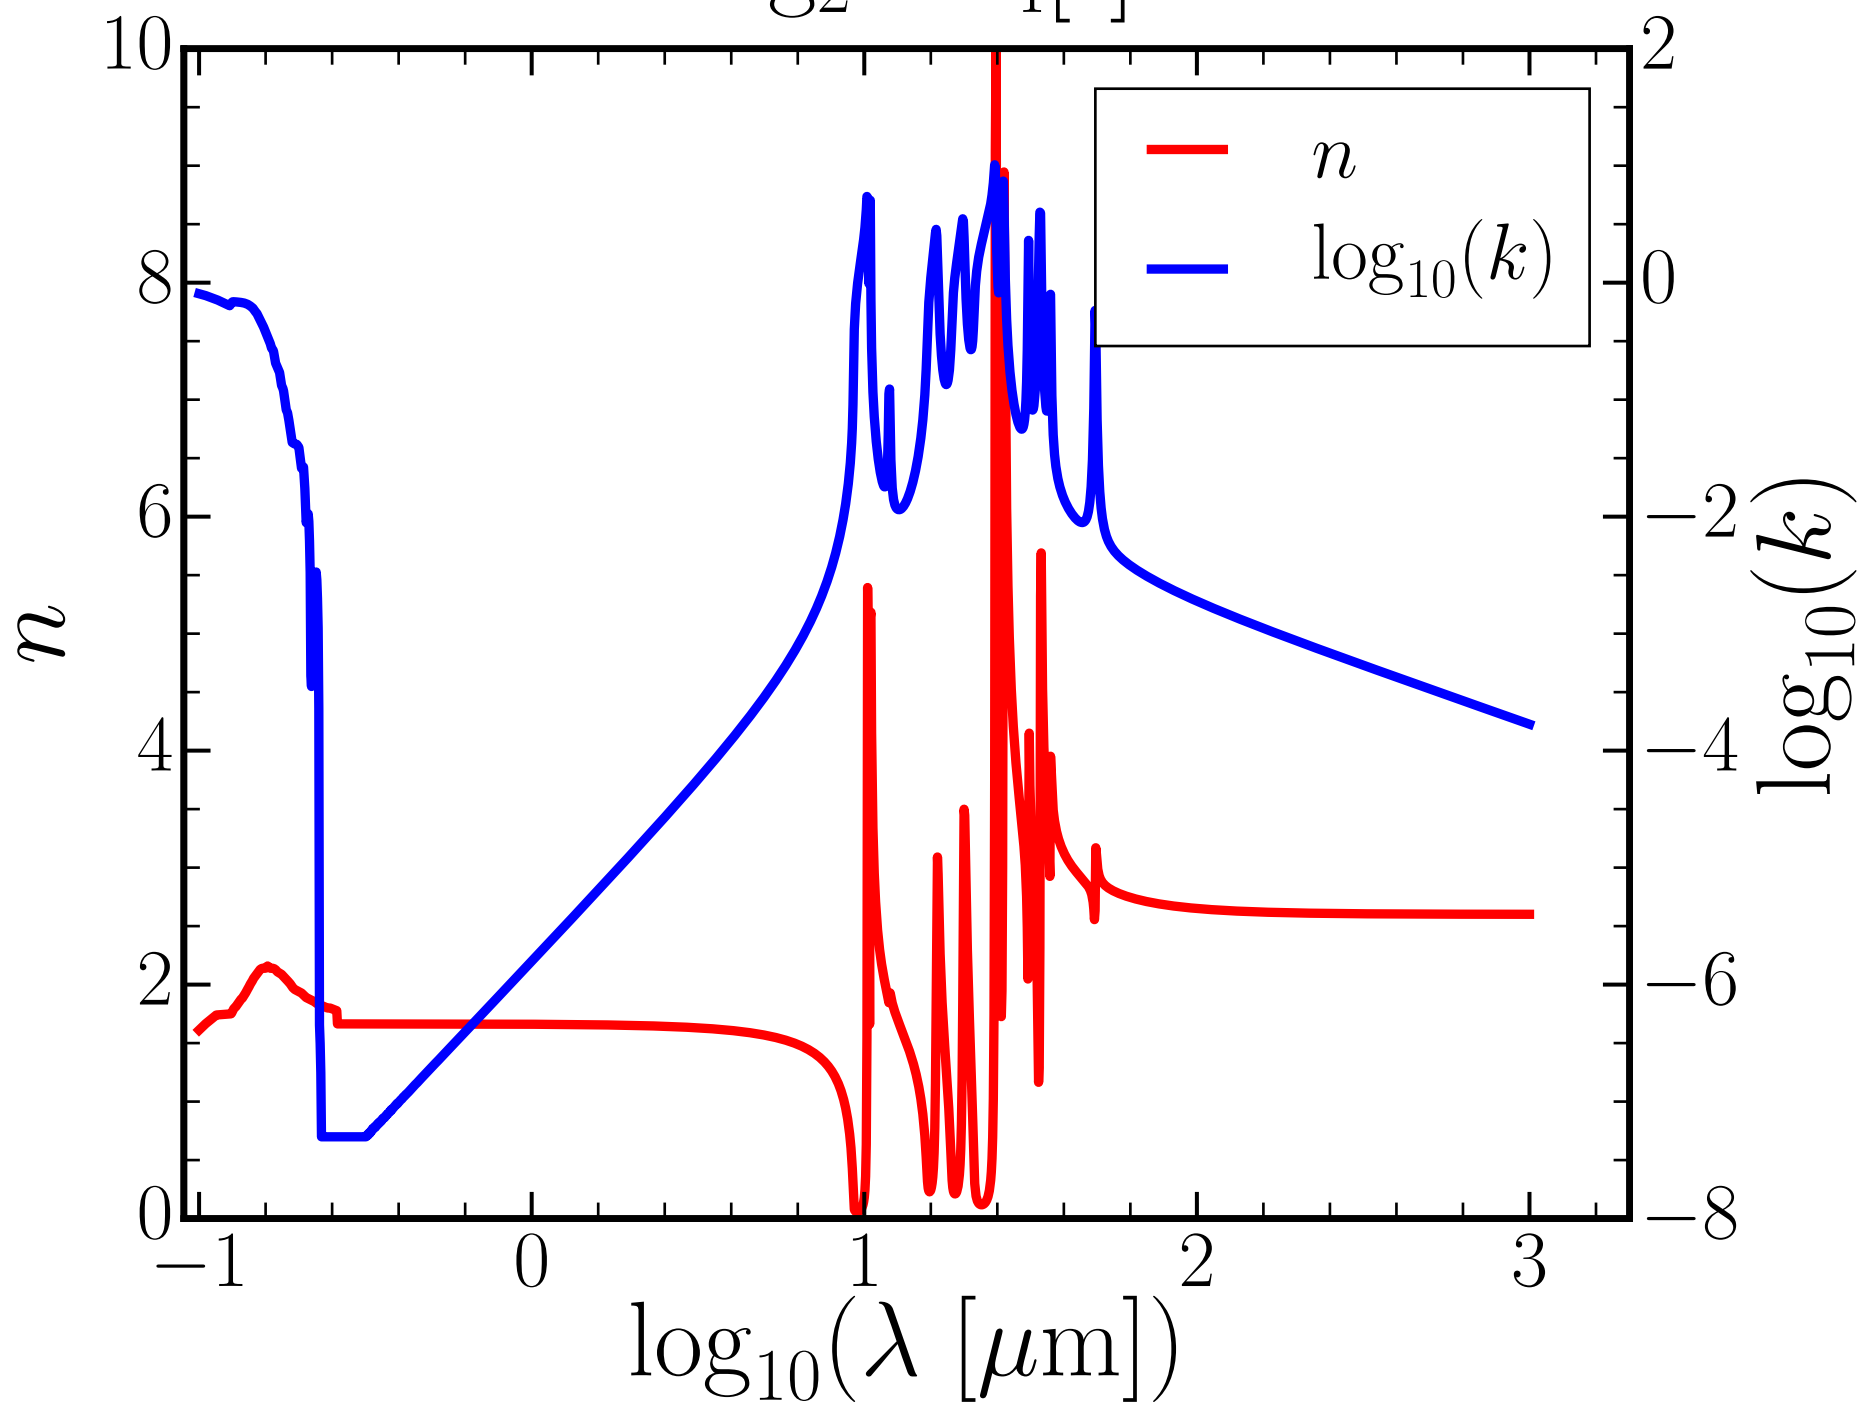

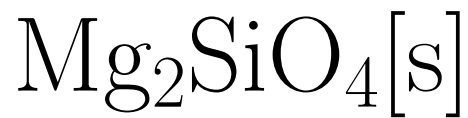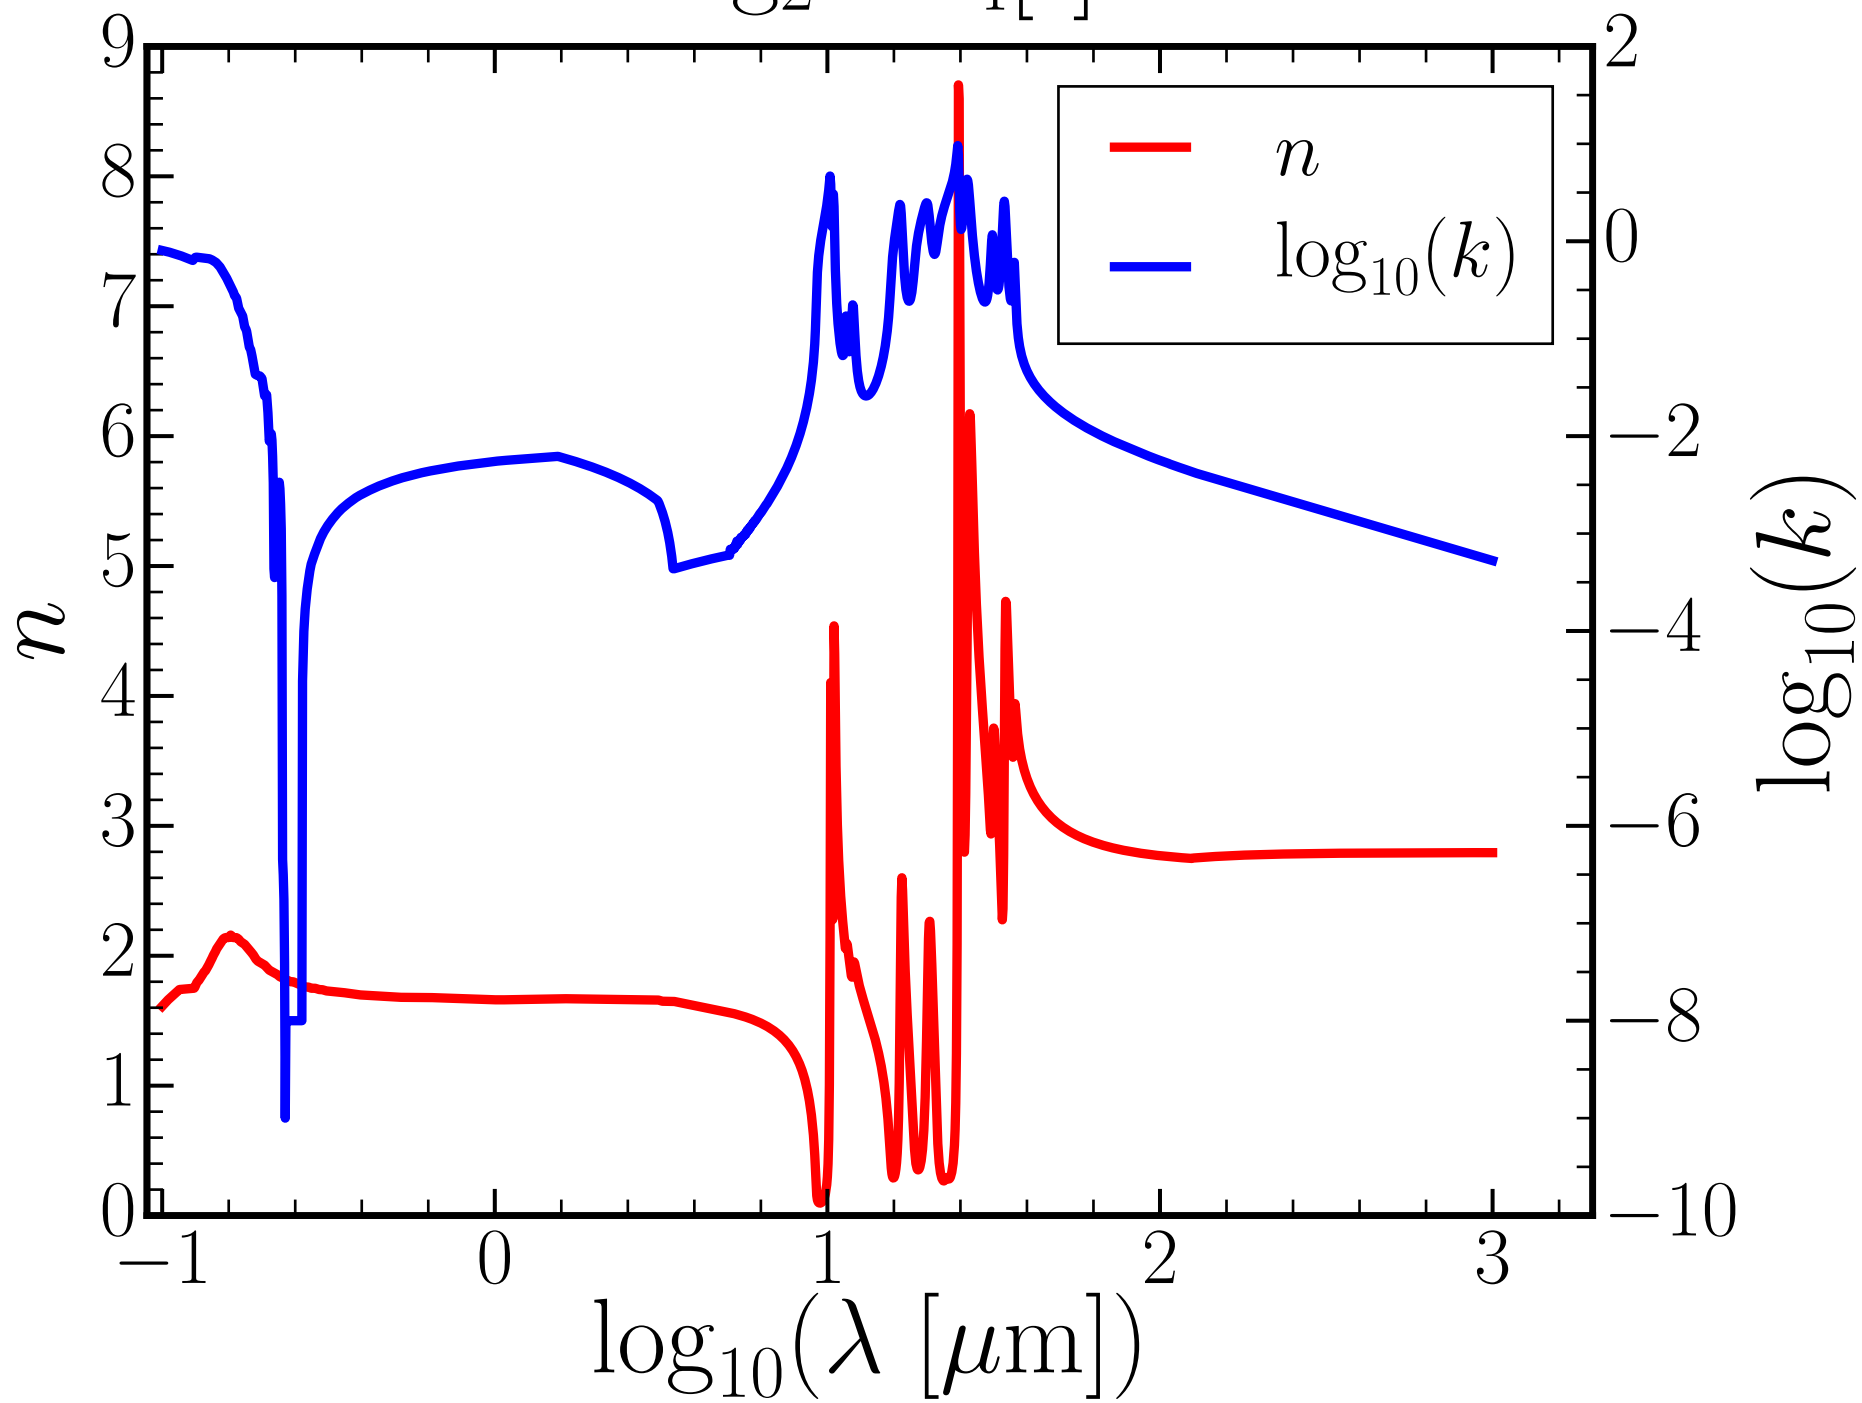

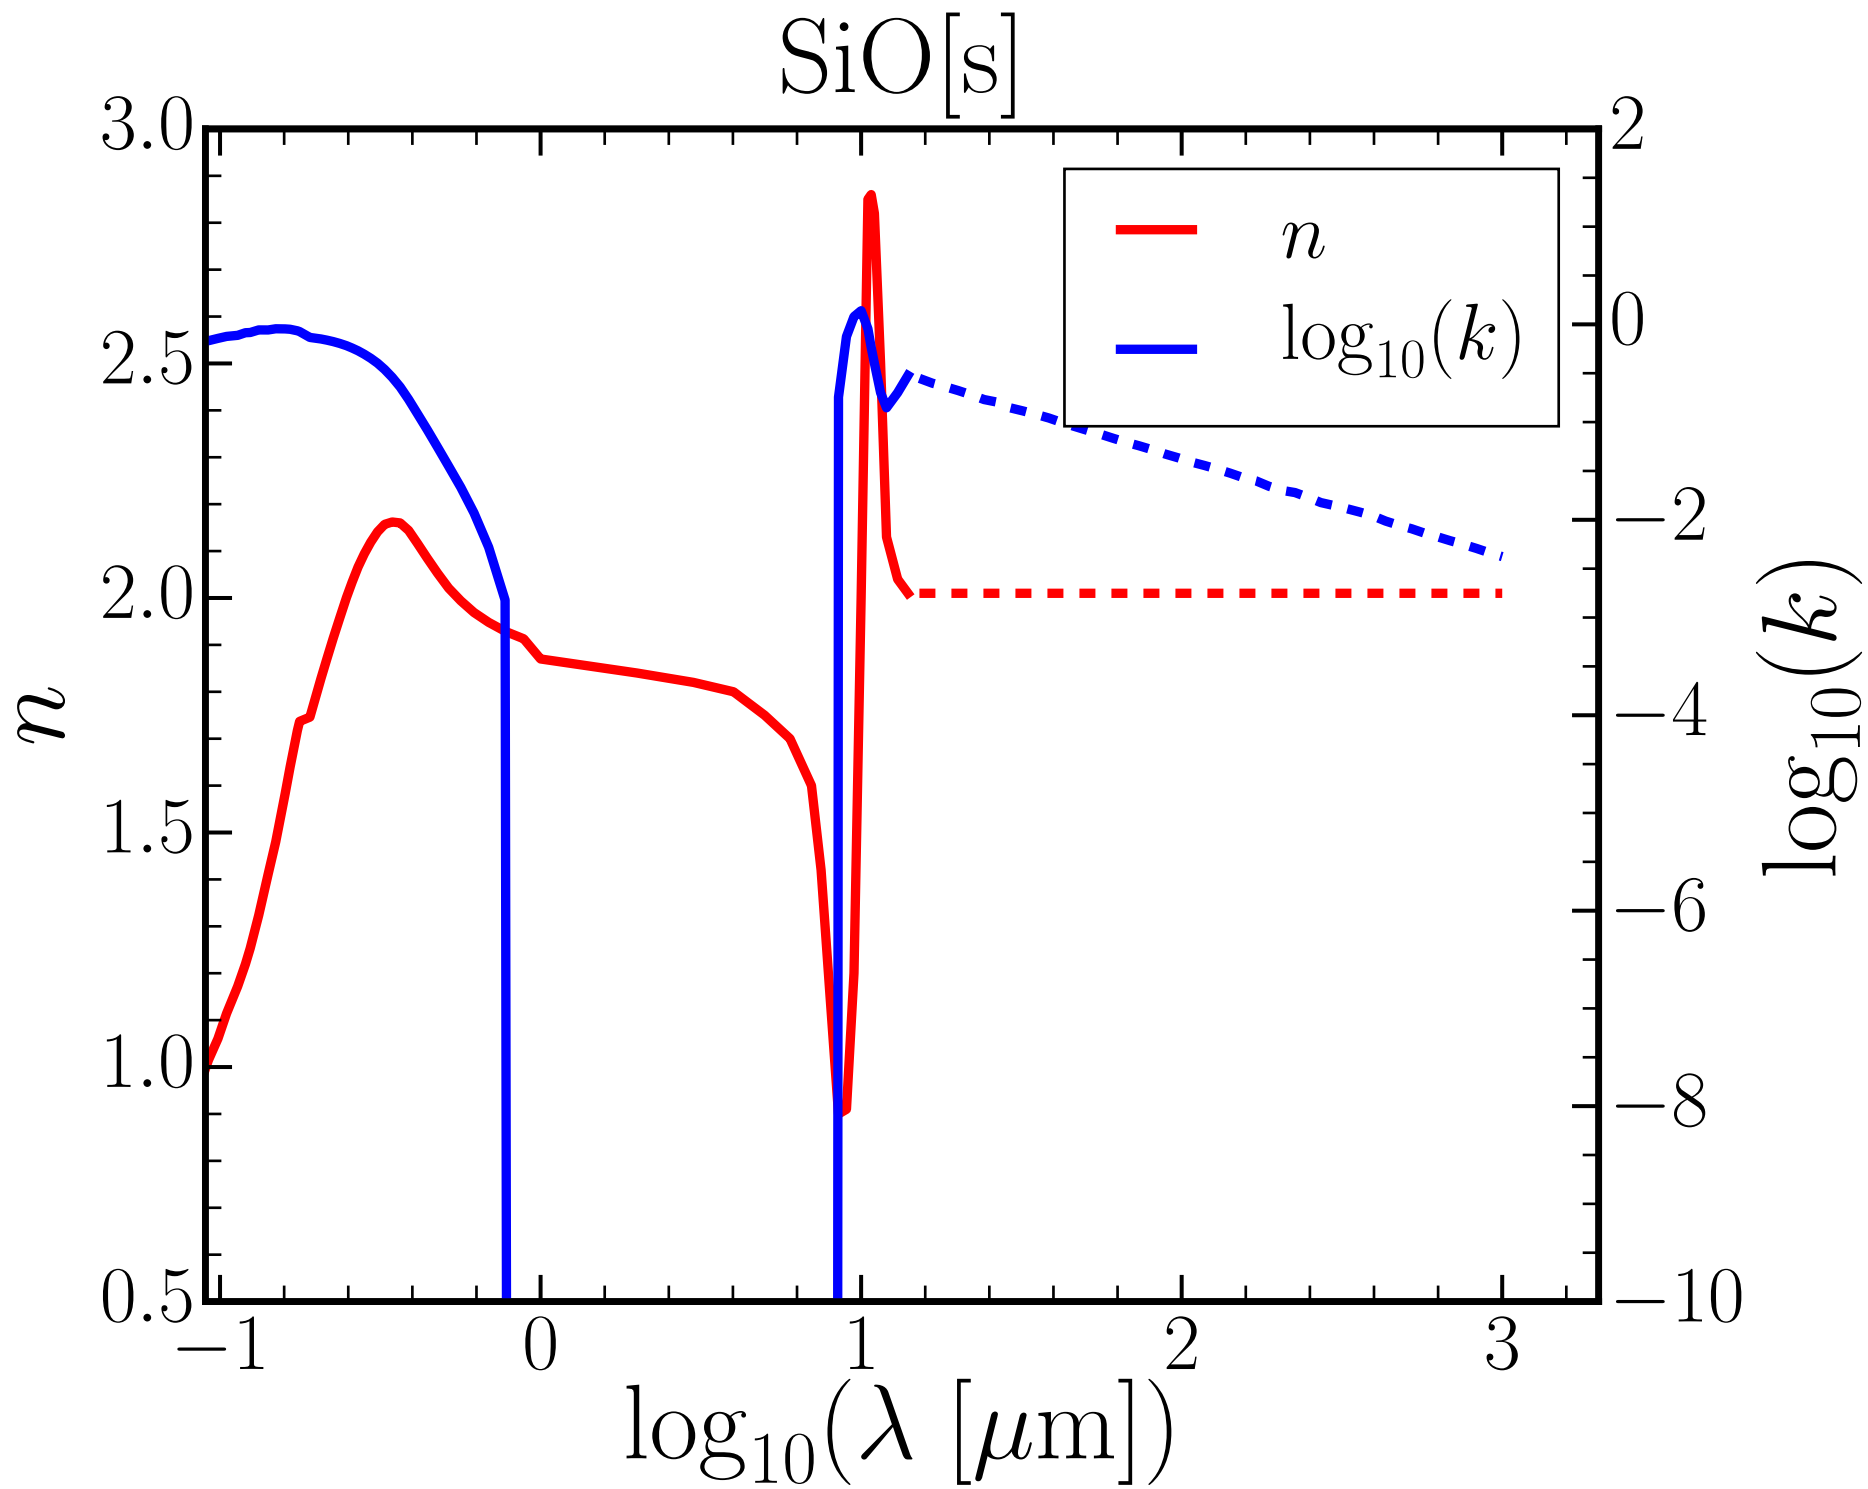

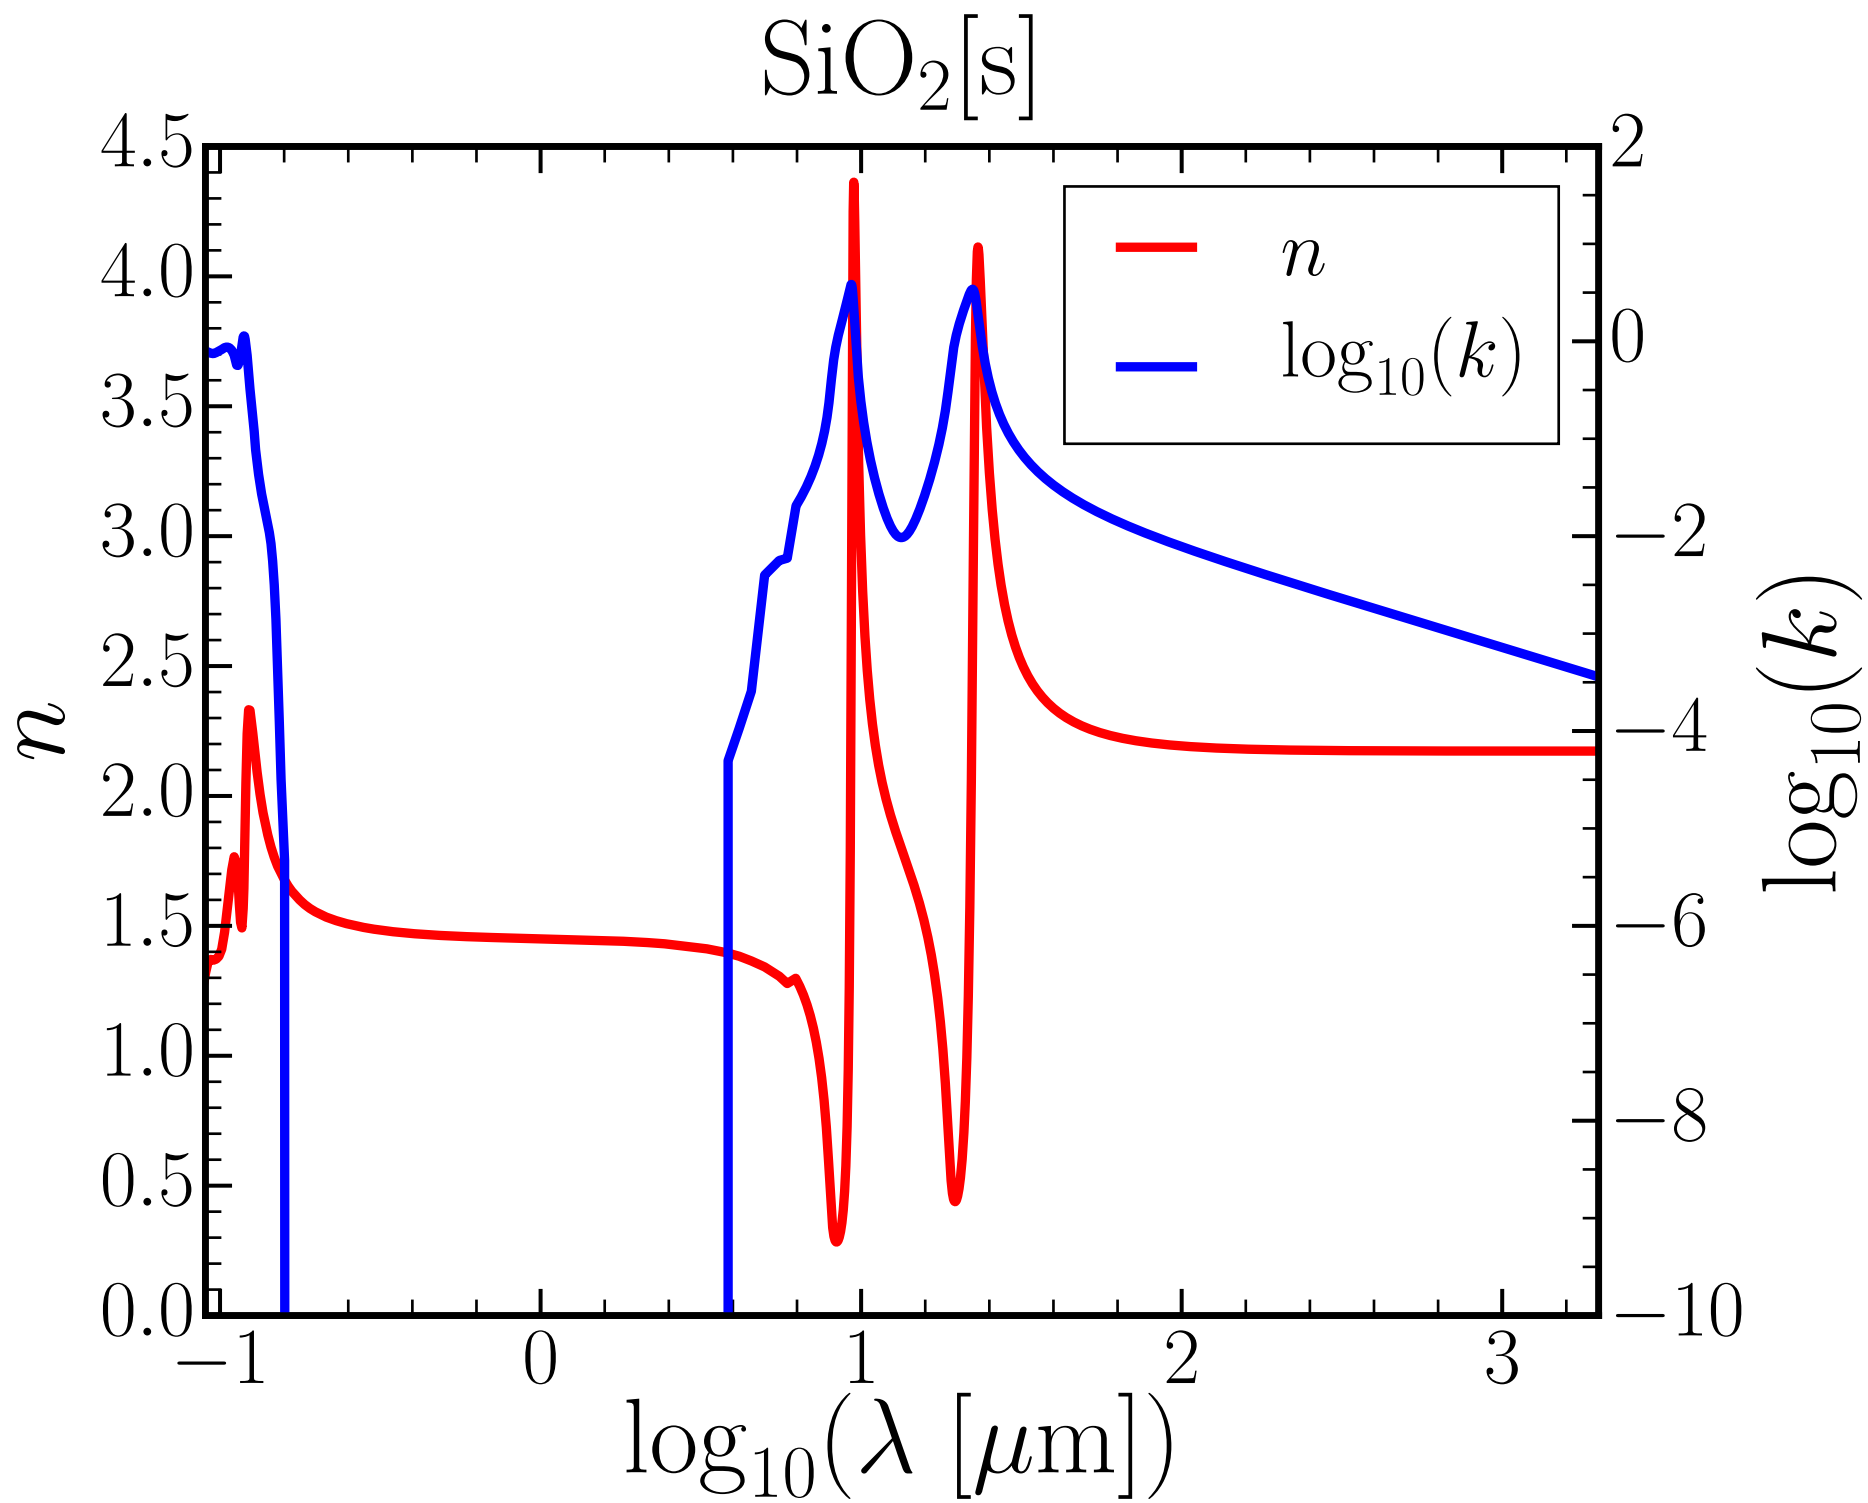

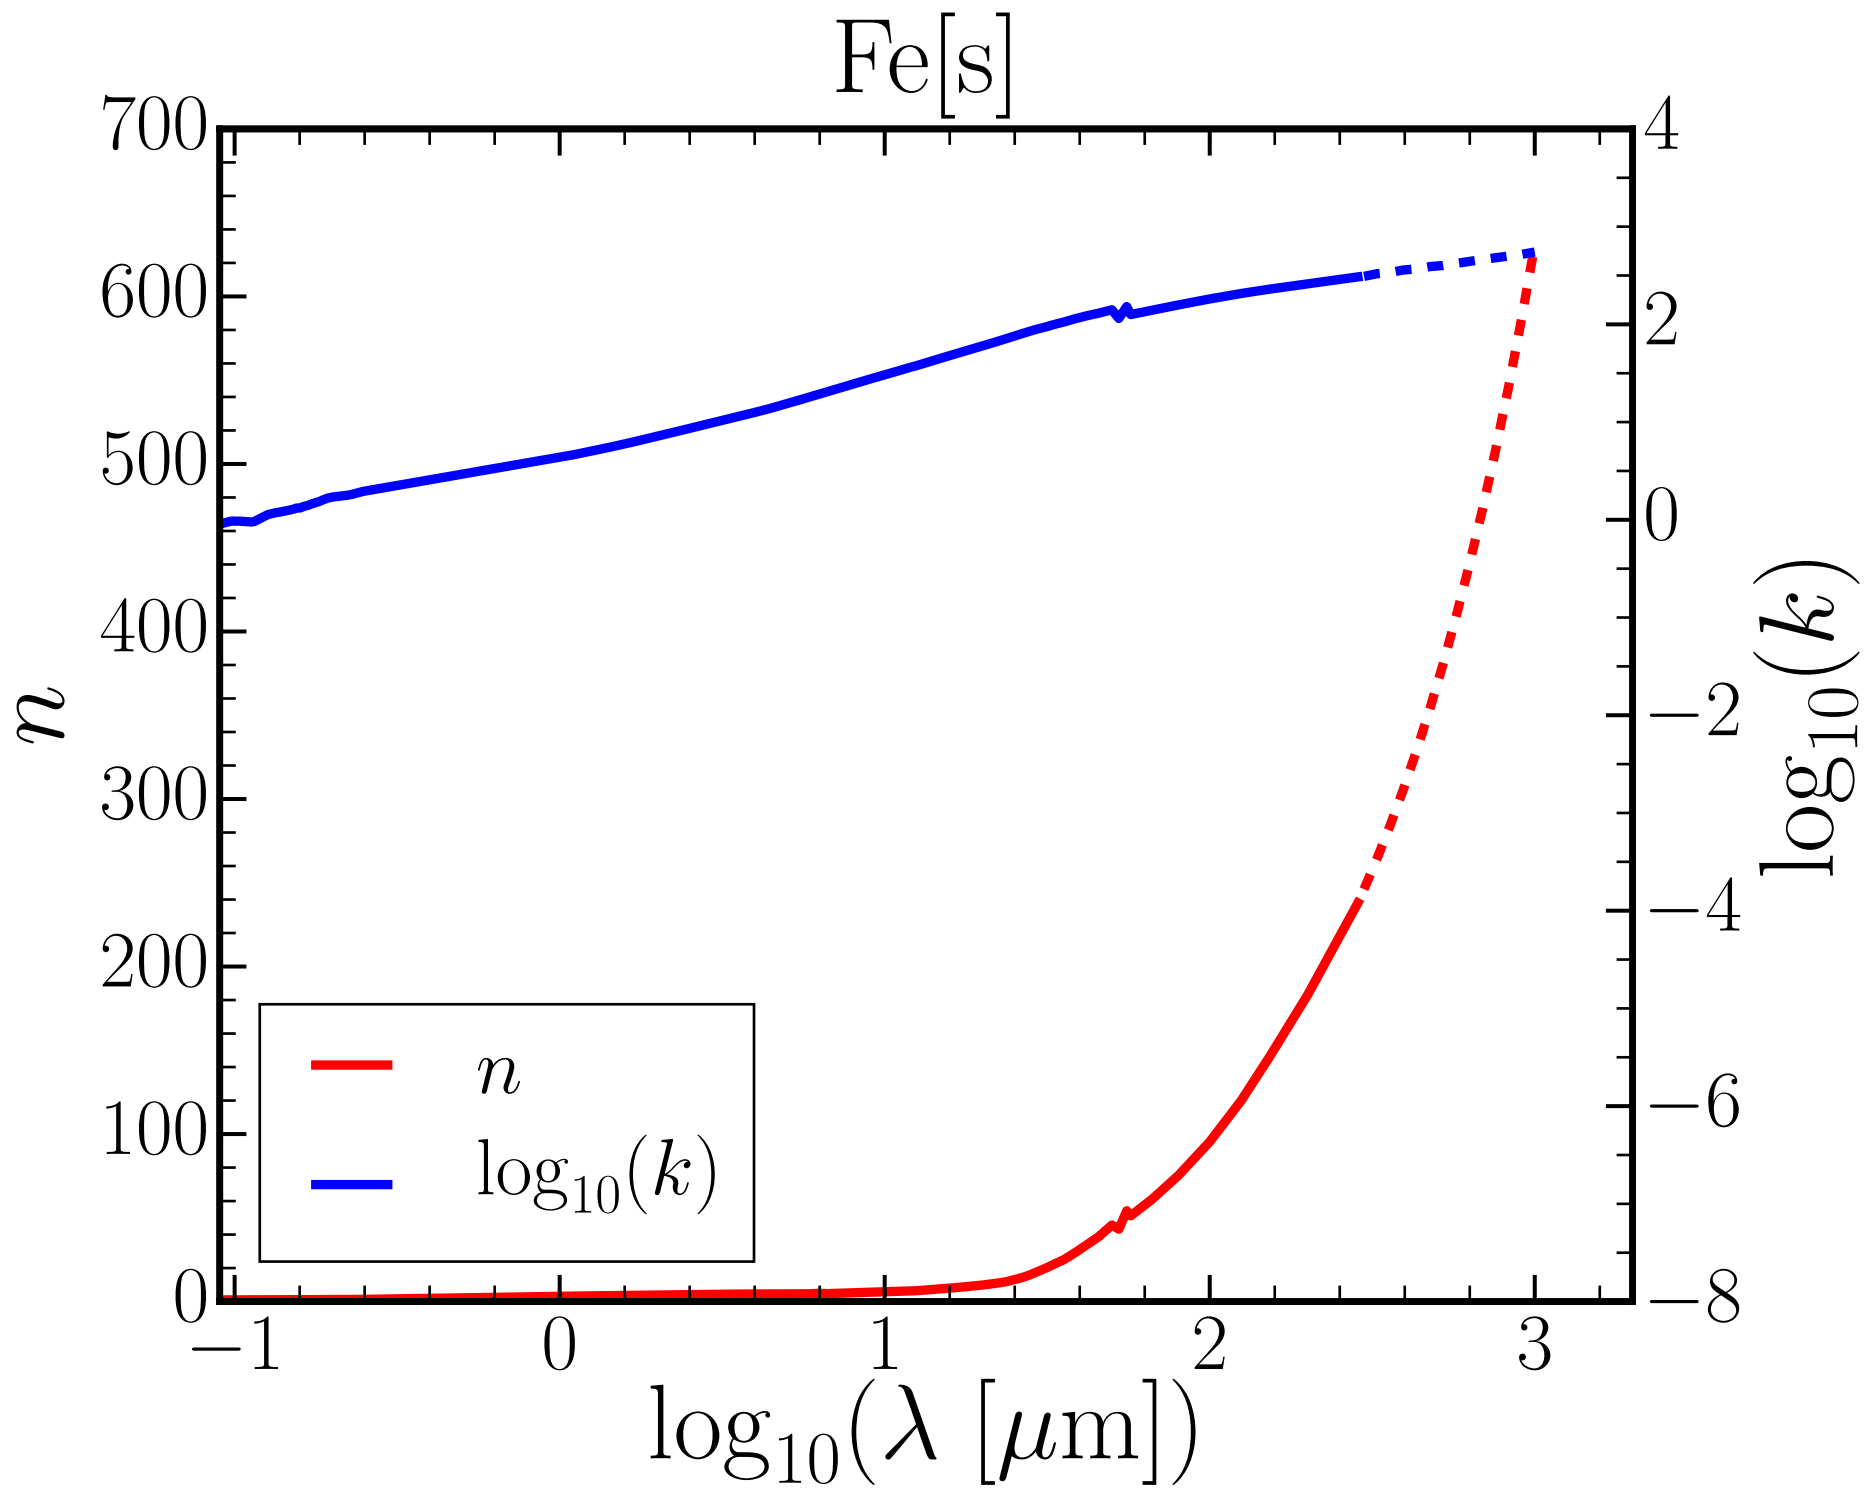

$\text{Al}_2\text{O}_3[\text{s}]$

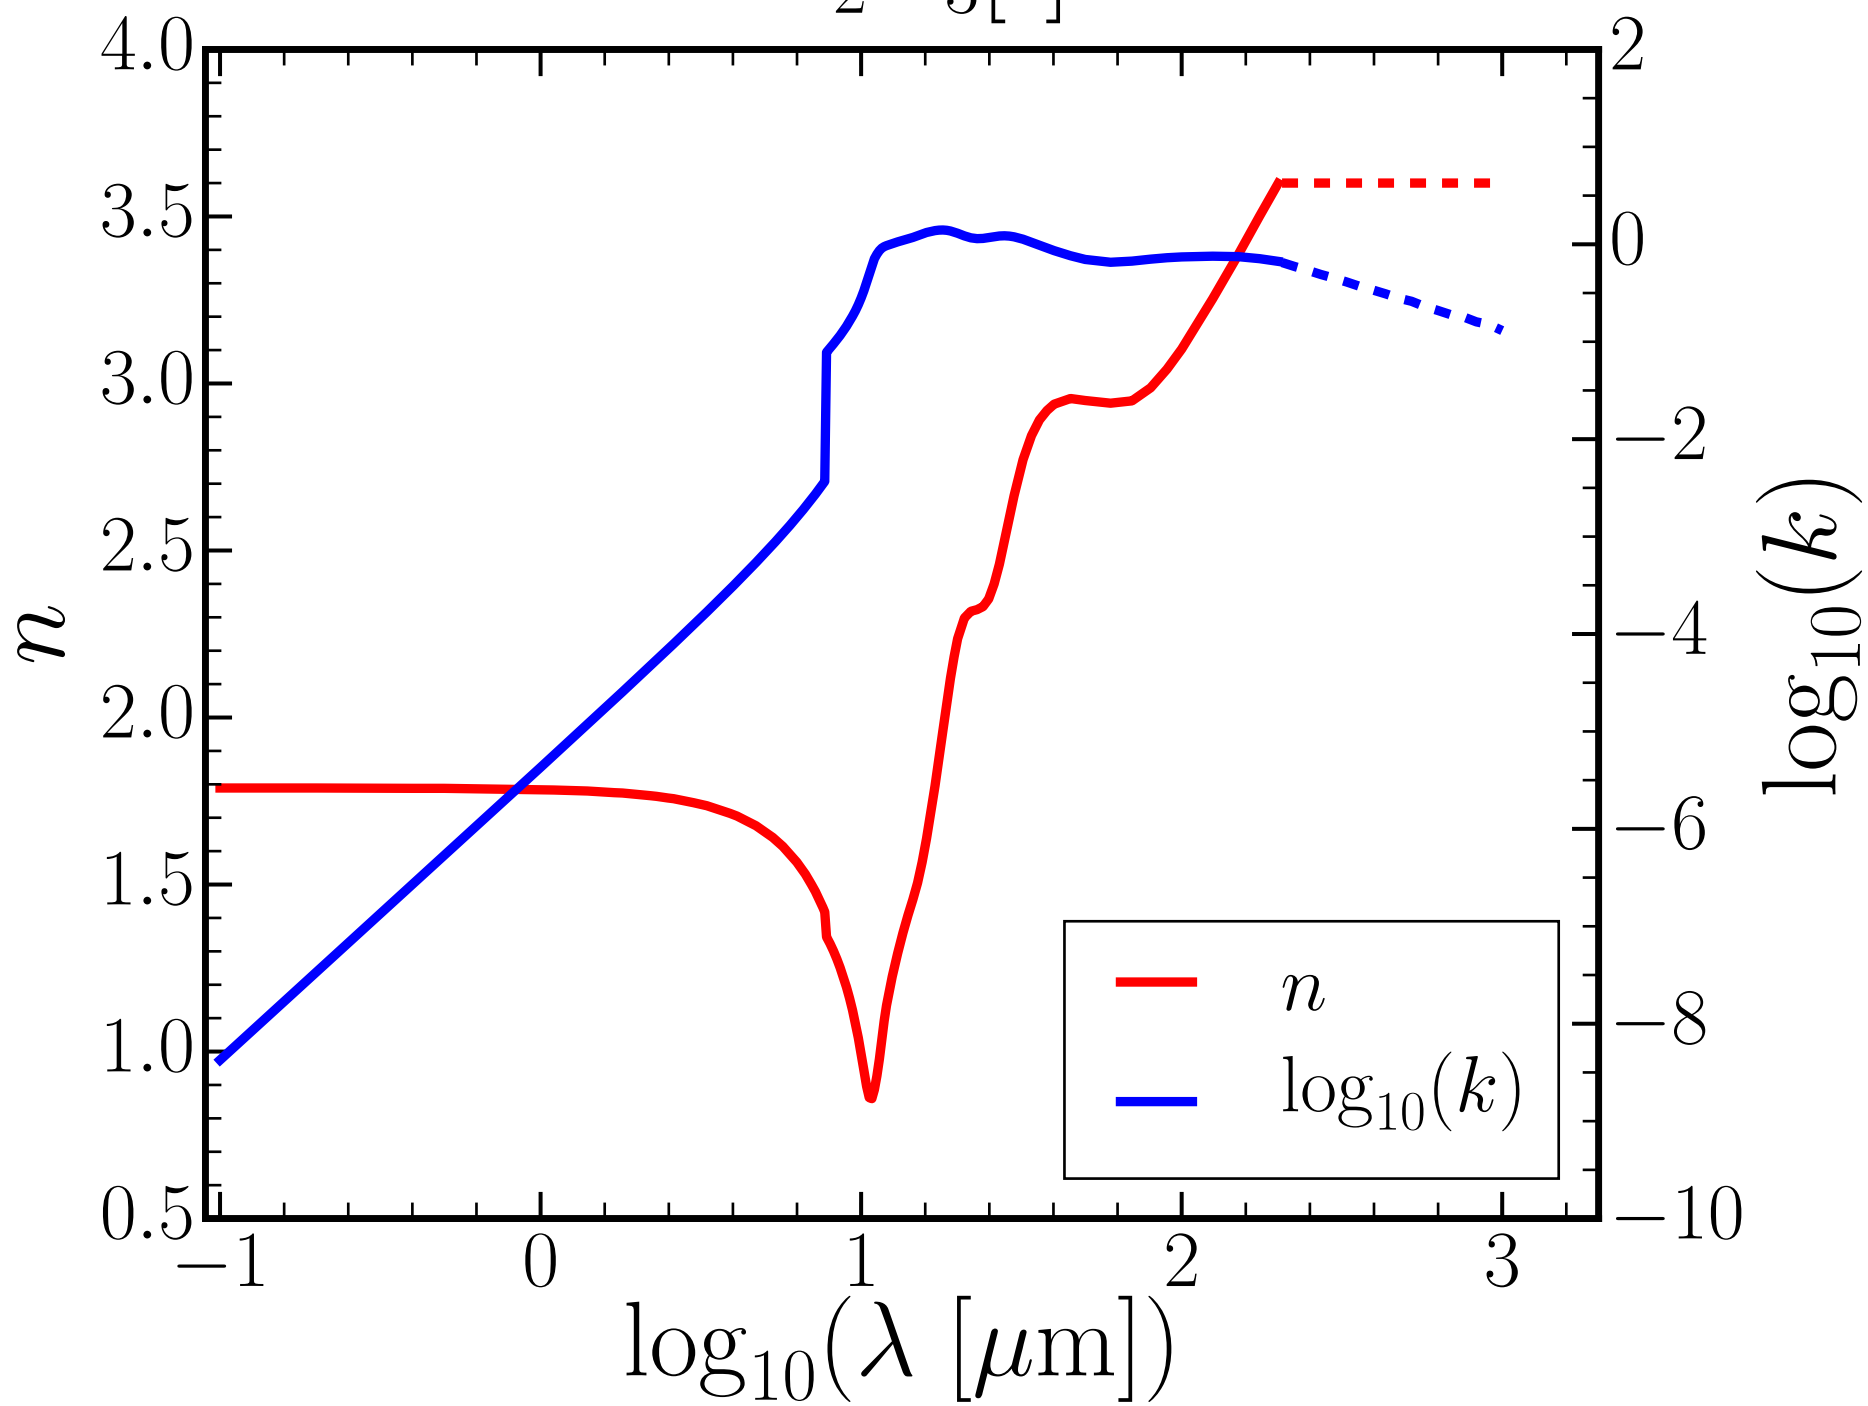

CaTiO<sub>3</sub>[s]

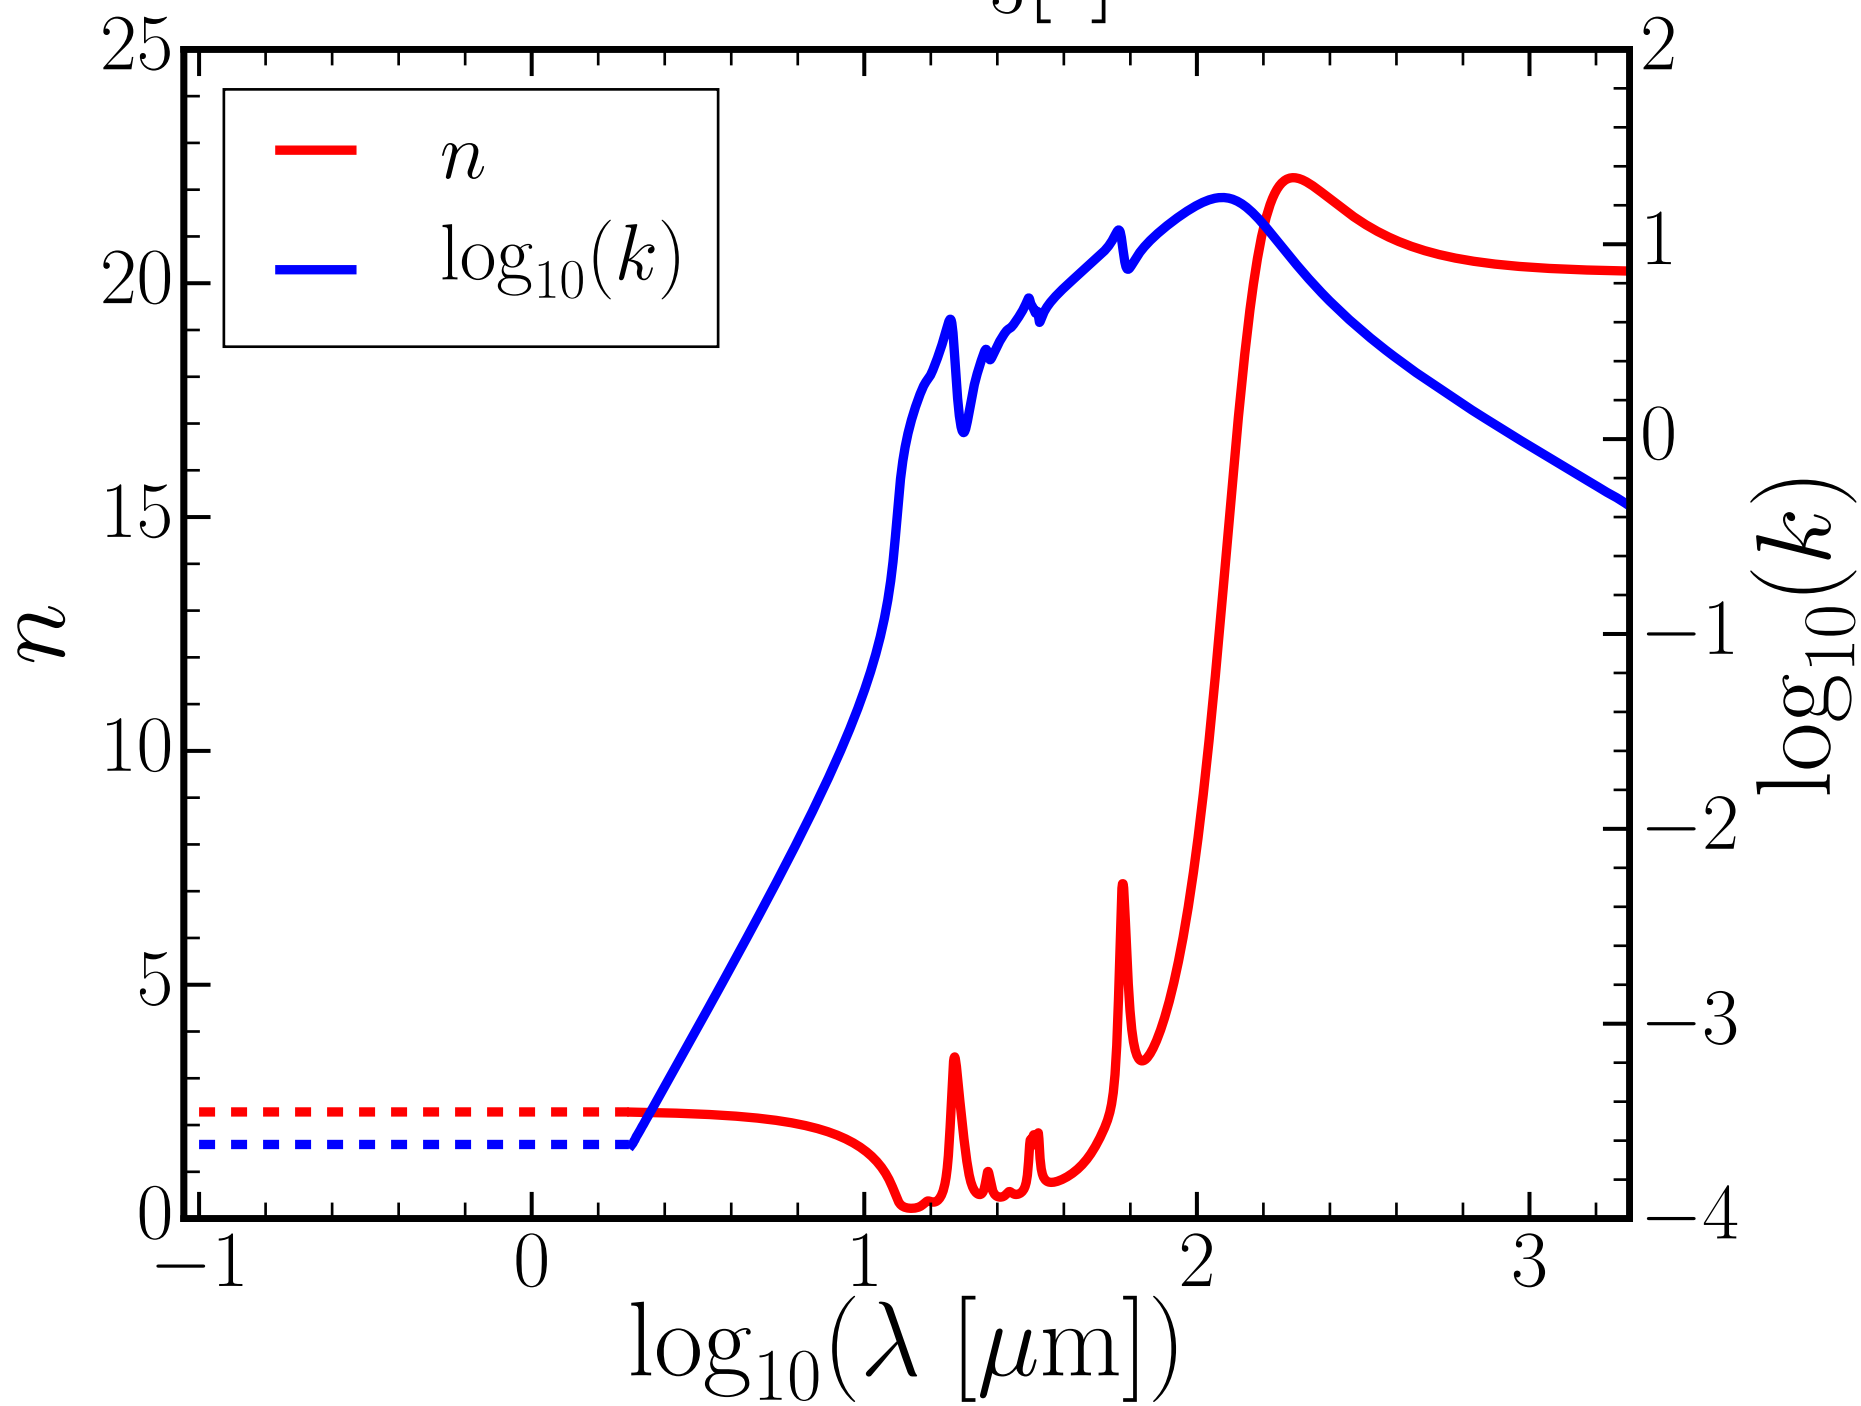



CaTiO<sub>3</sub>[s]

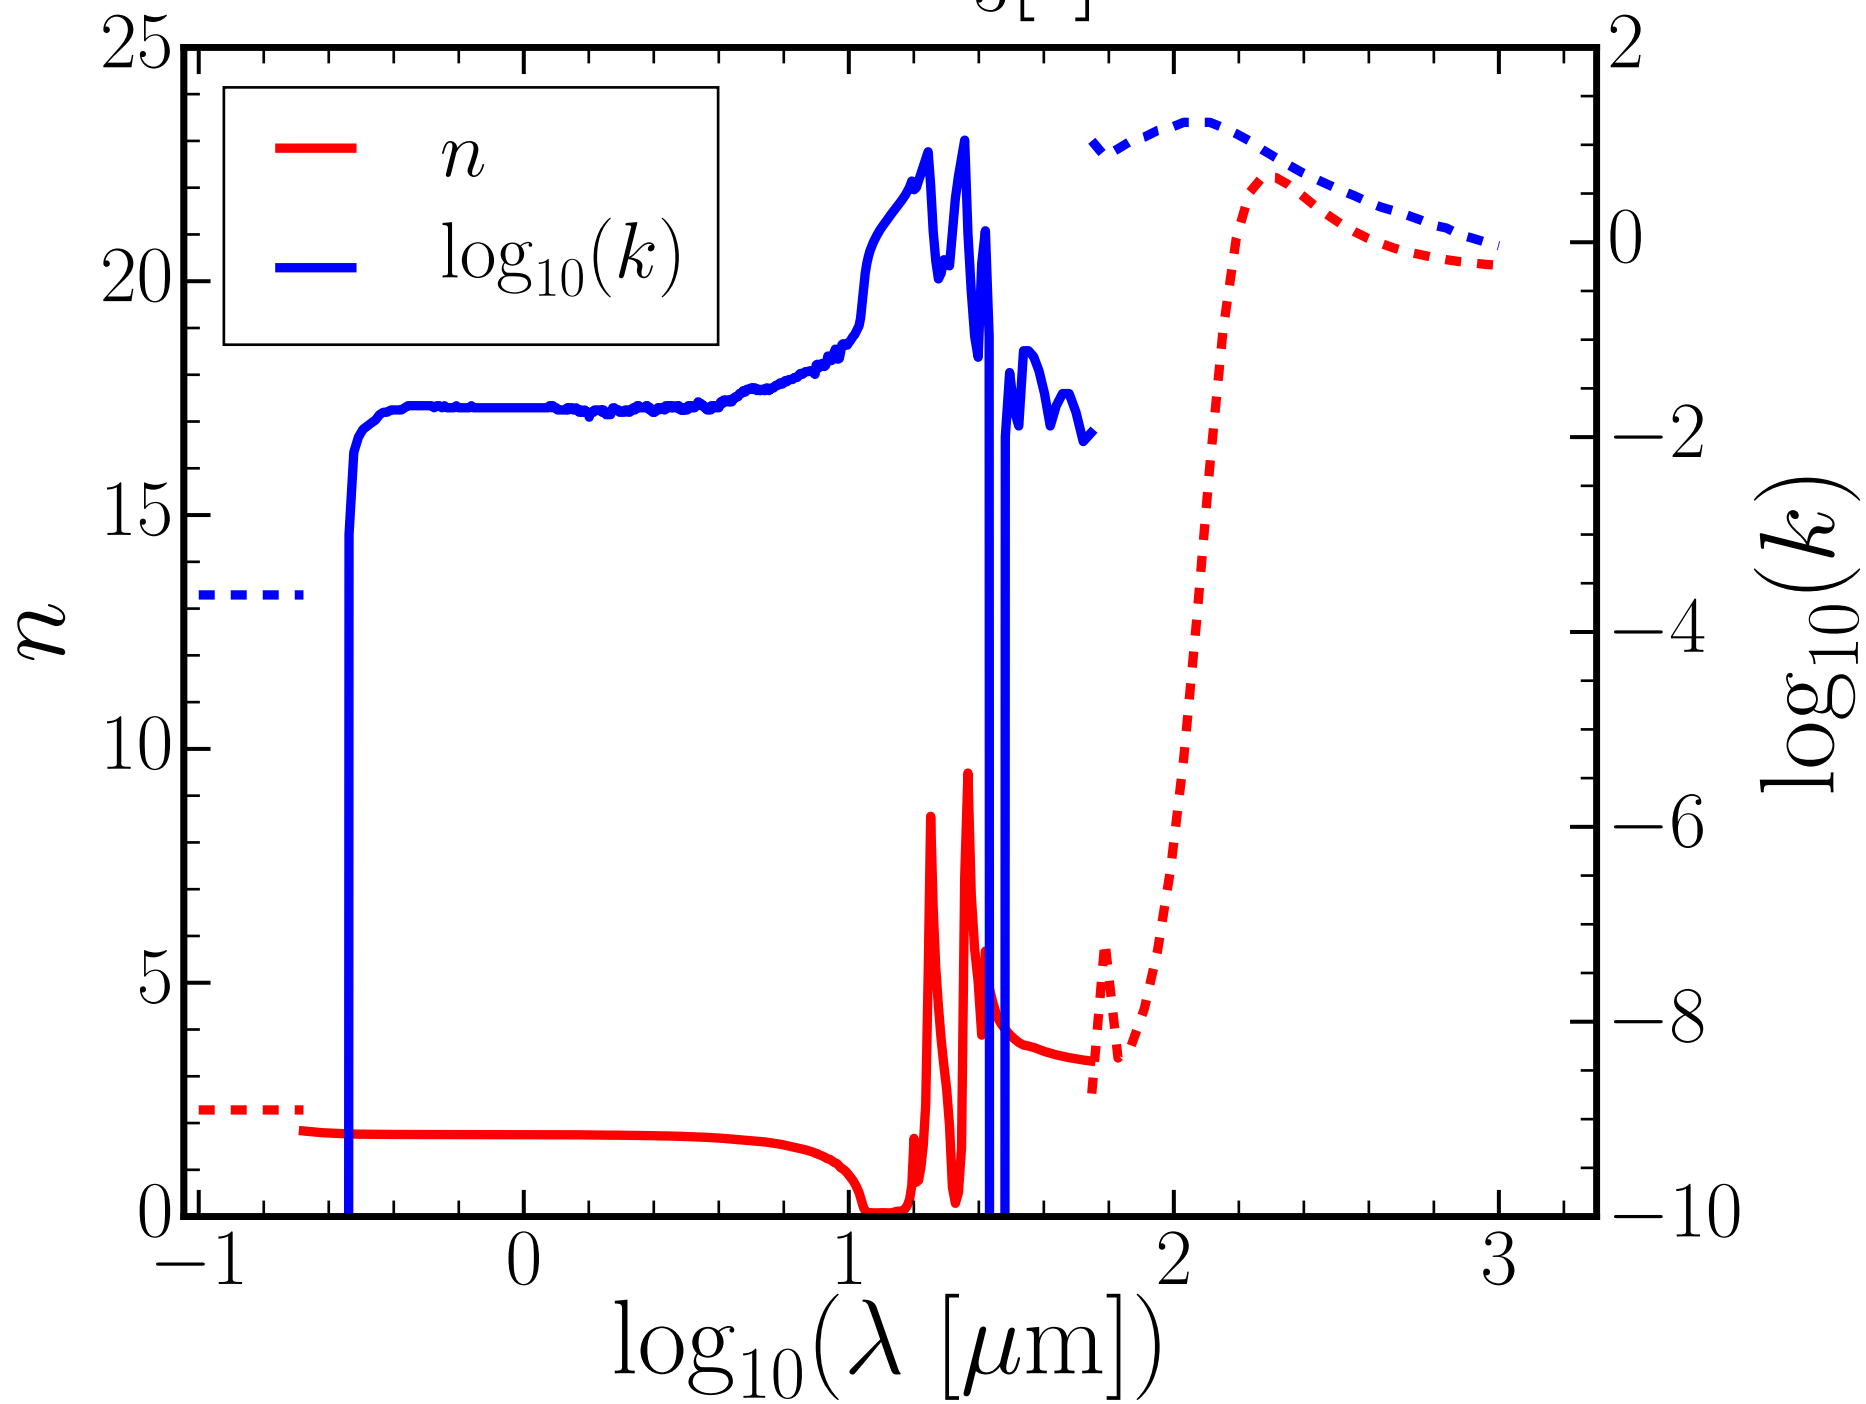

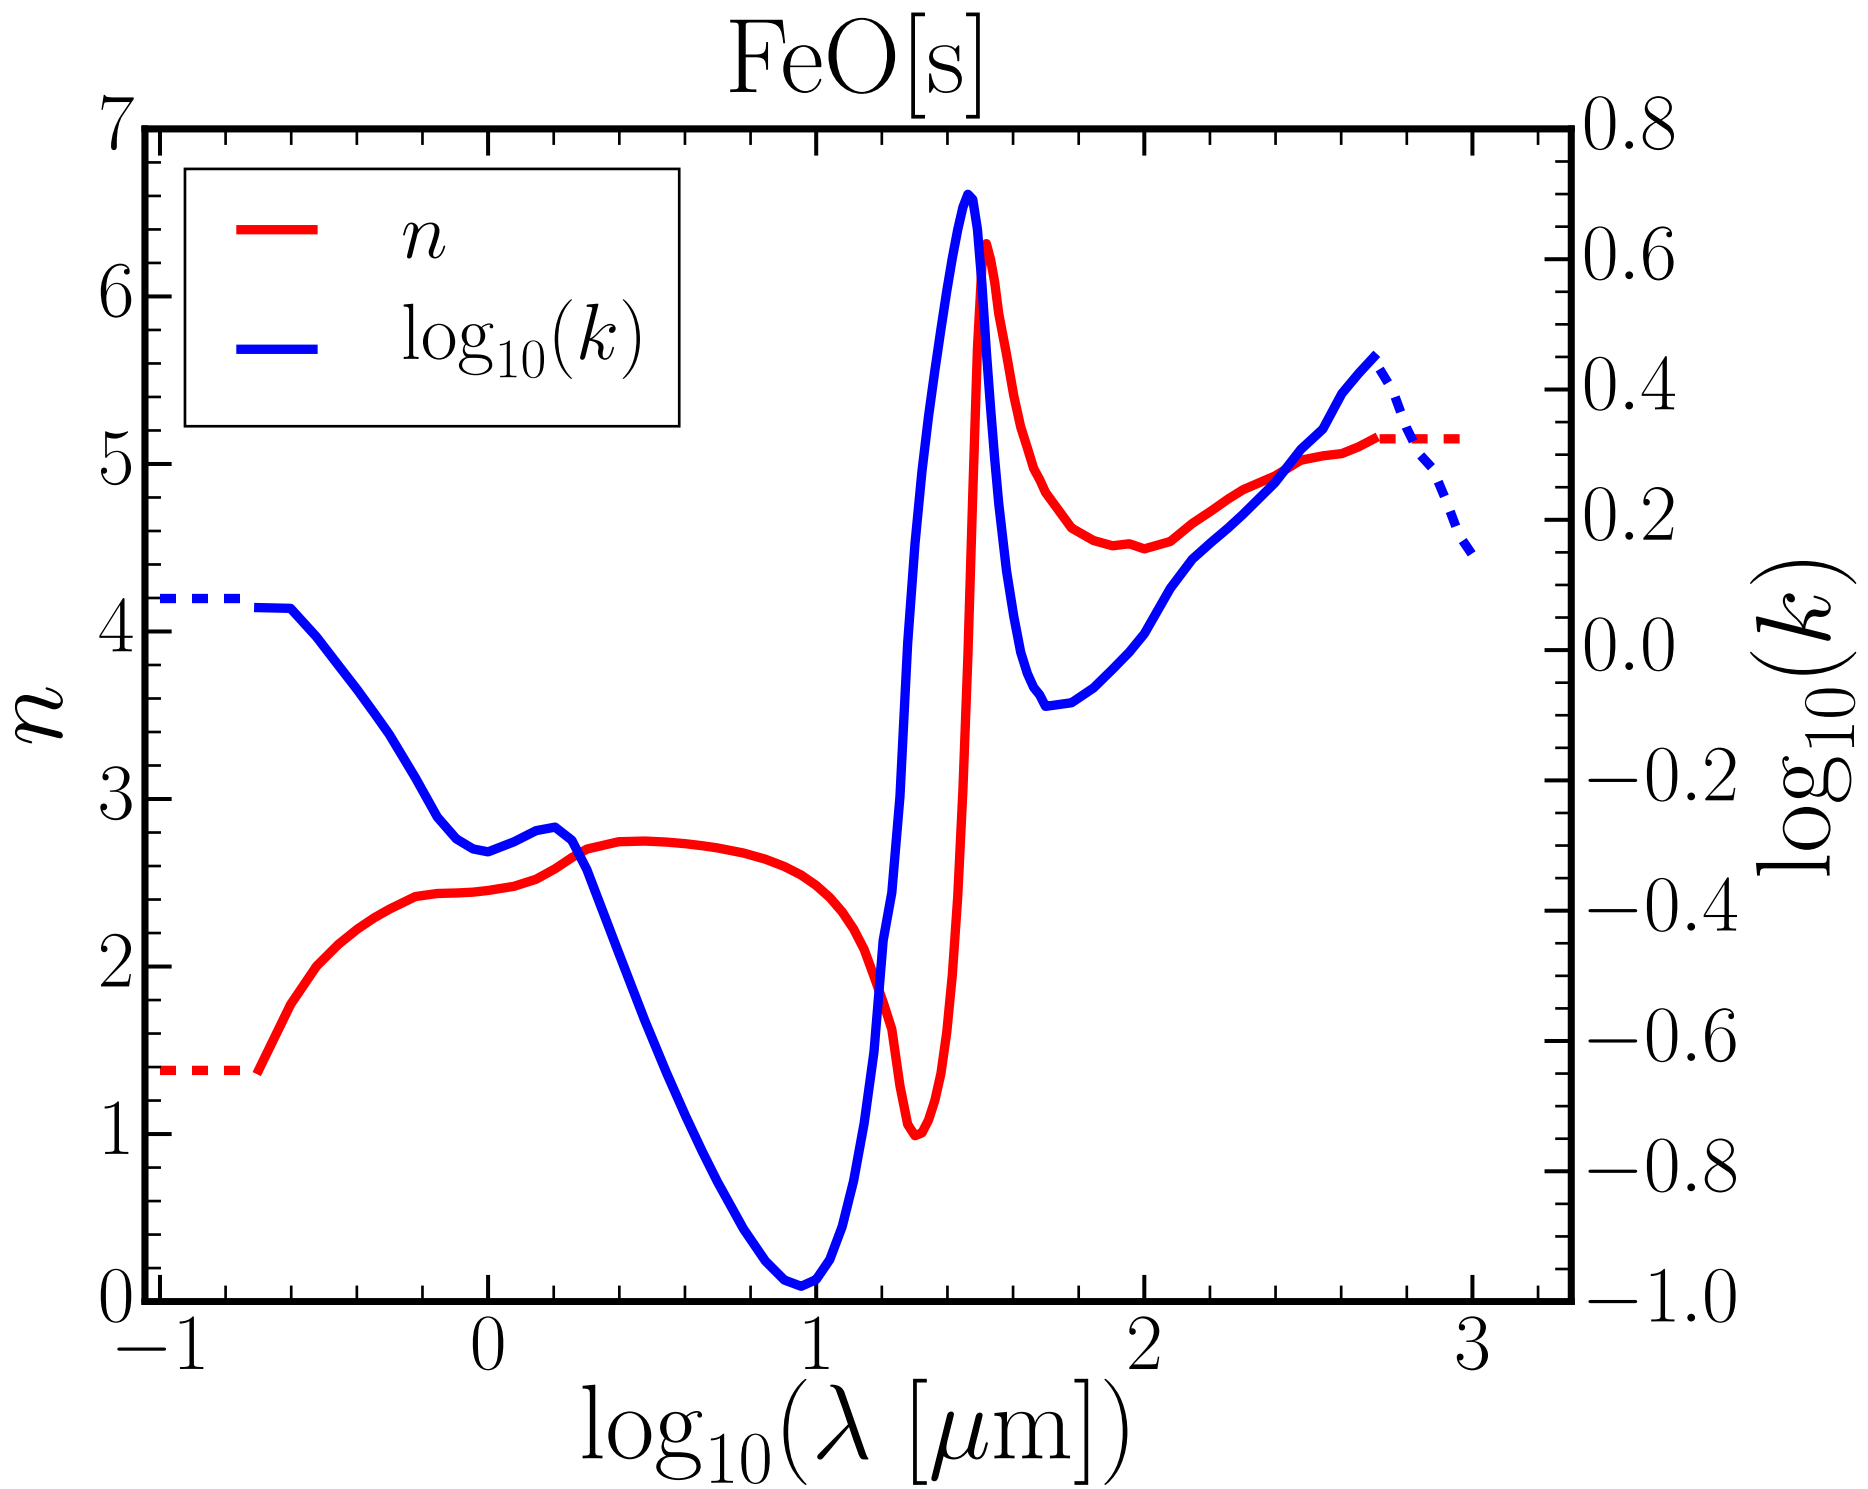

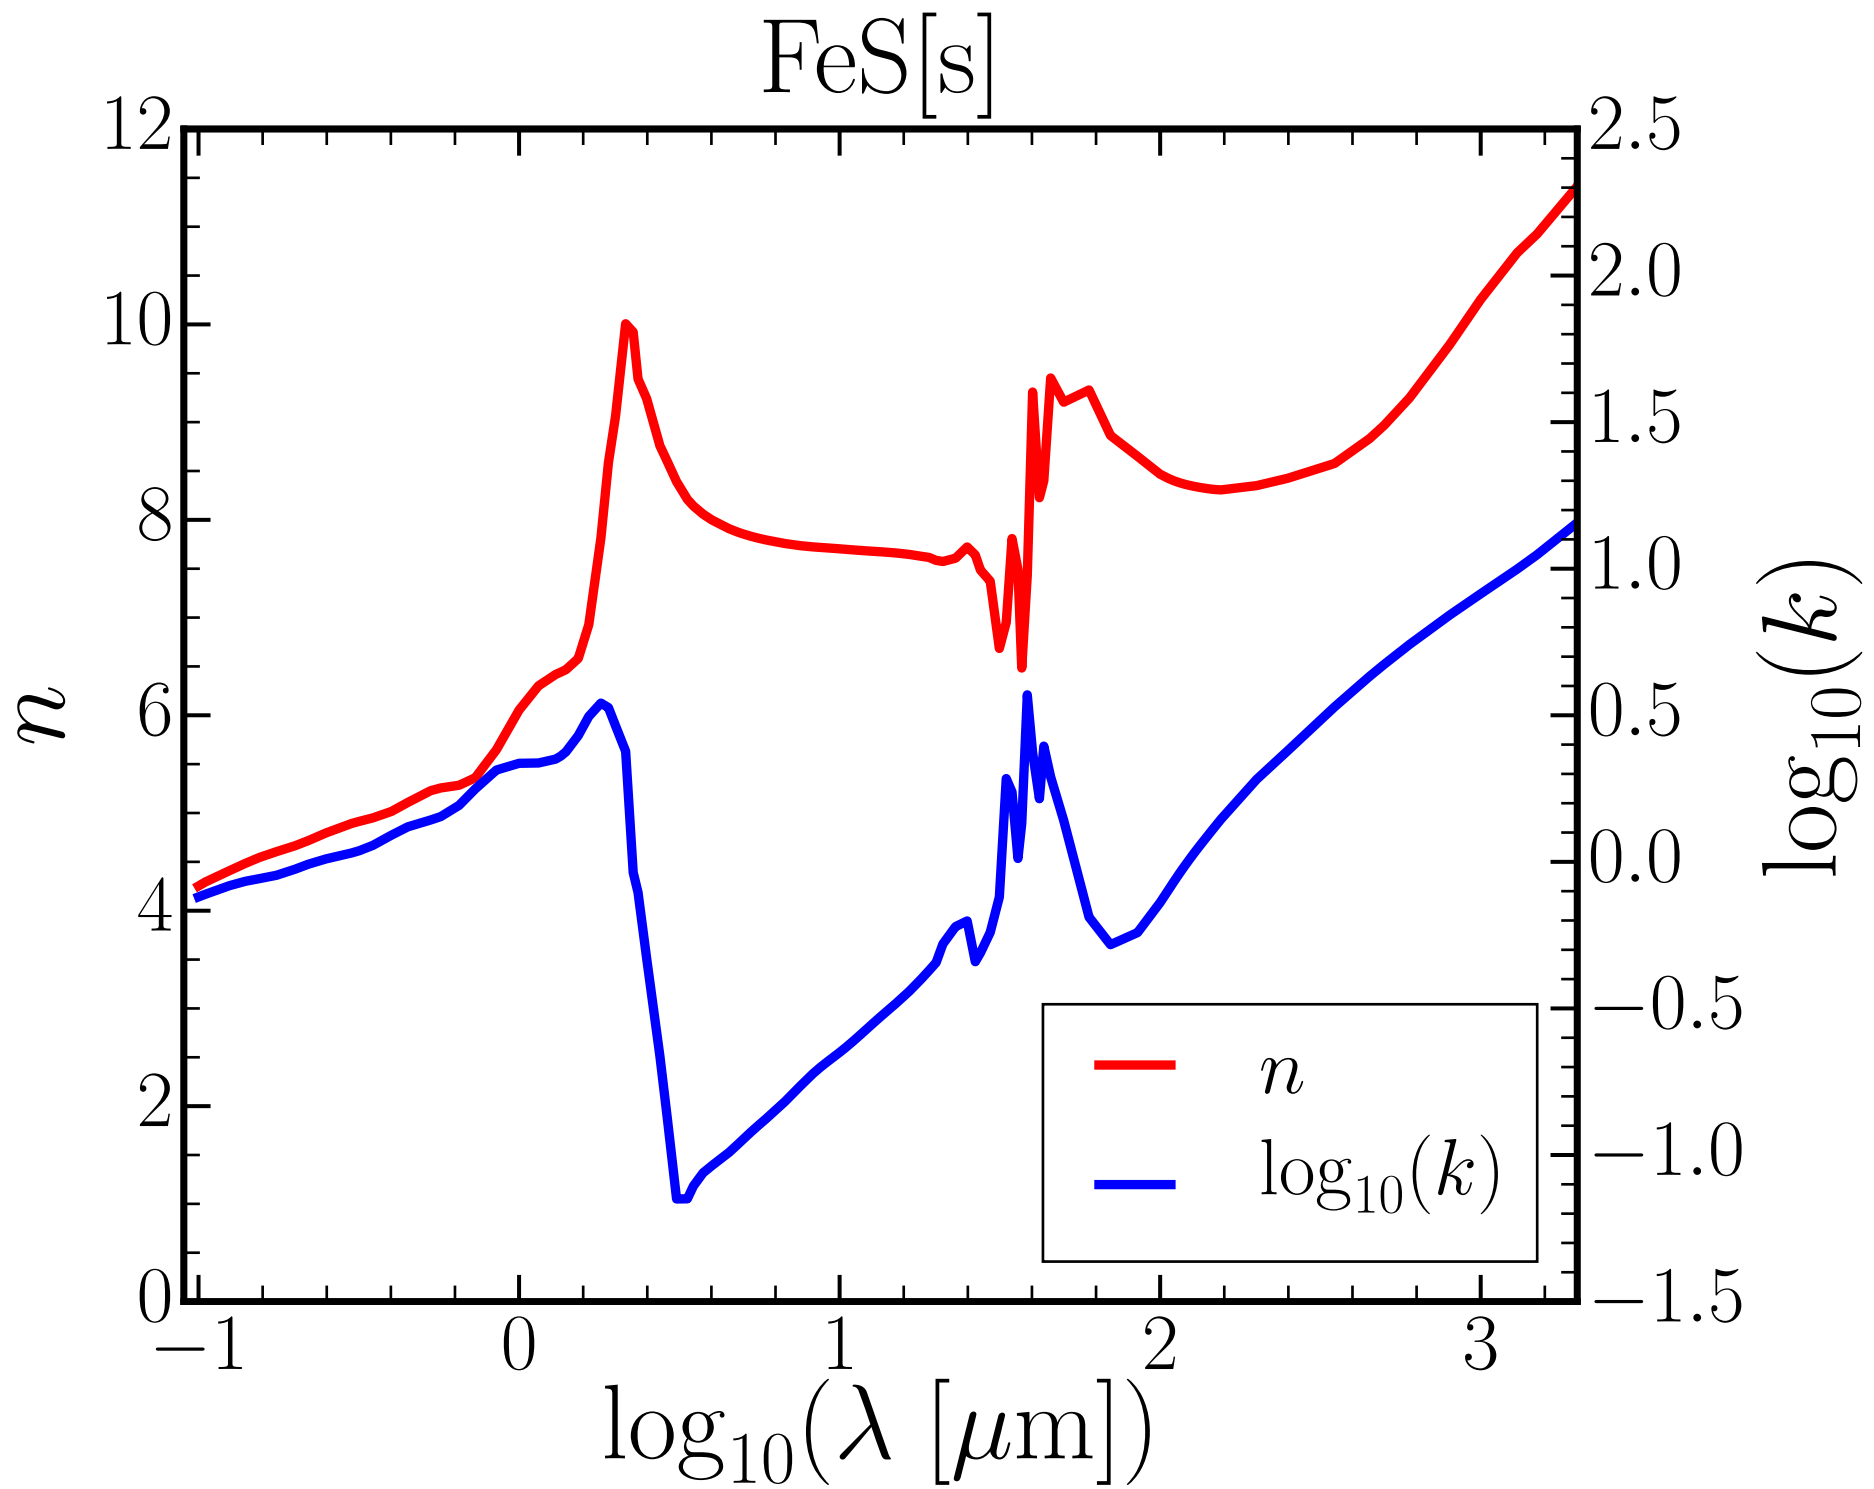

$\text{Fe}_2\text{O}_3[\text{s}]$

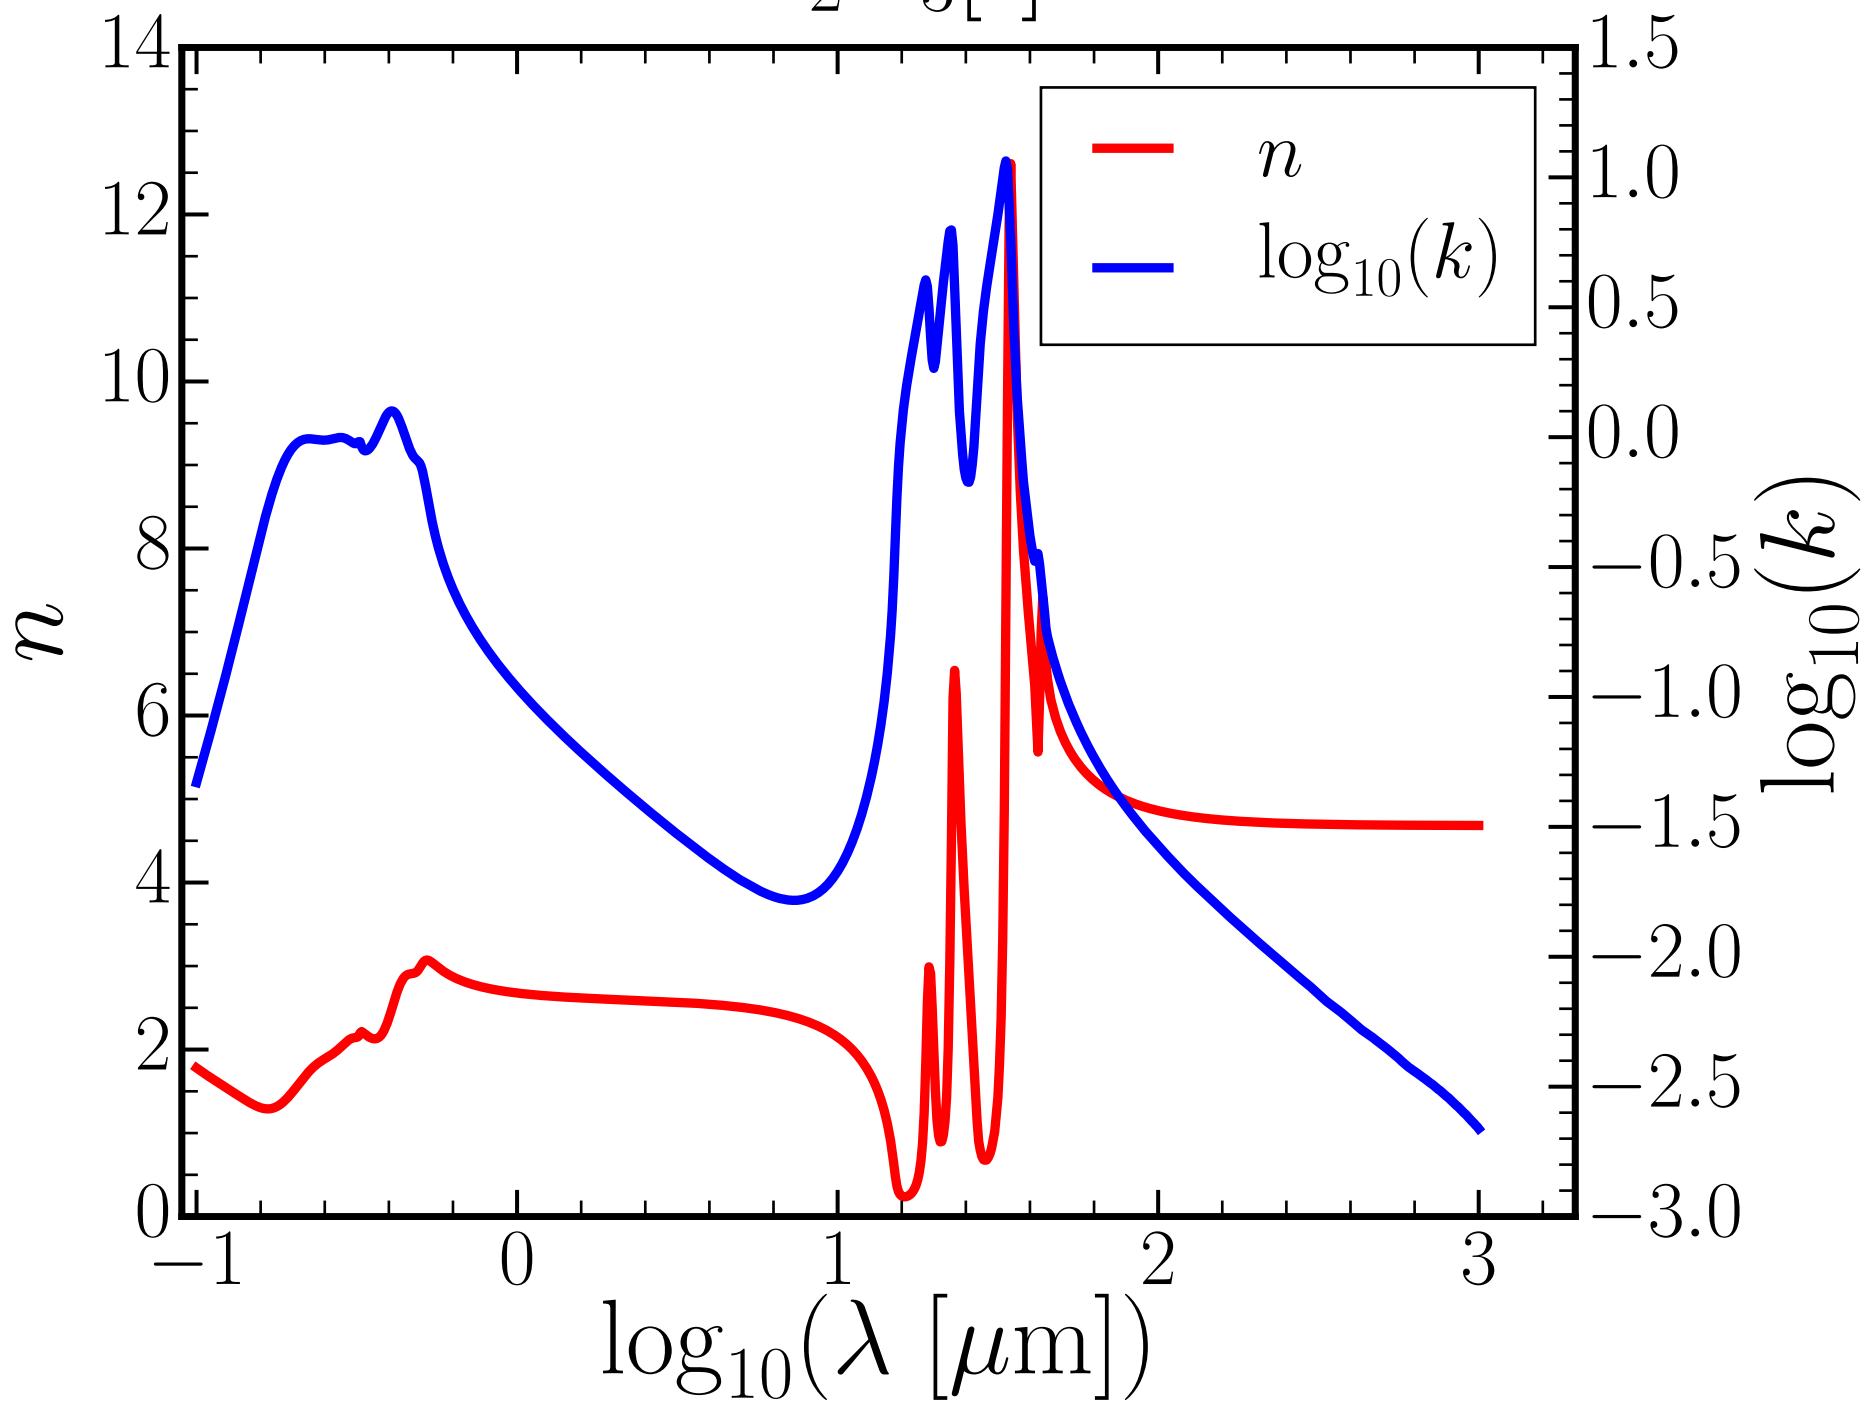

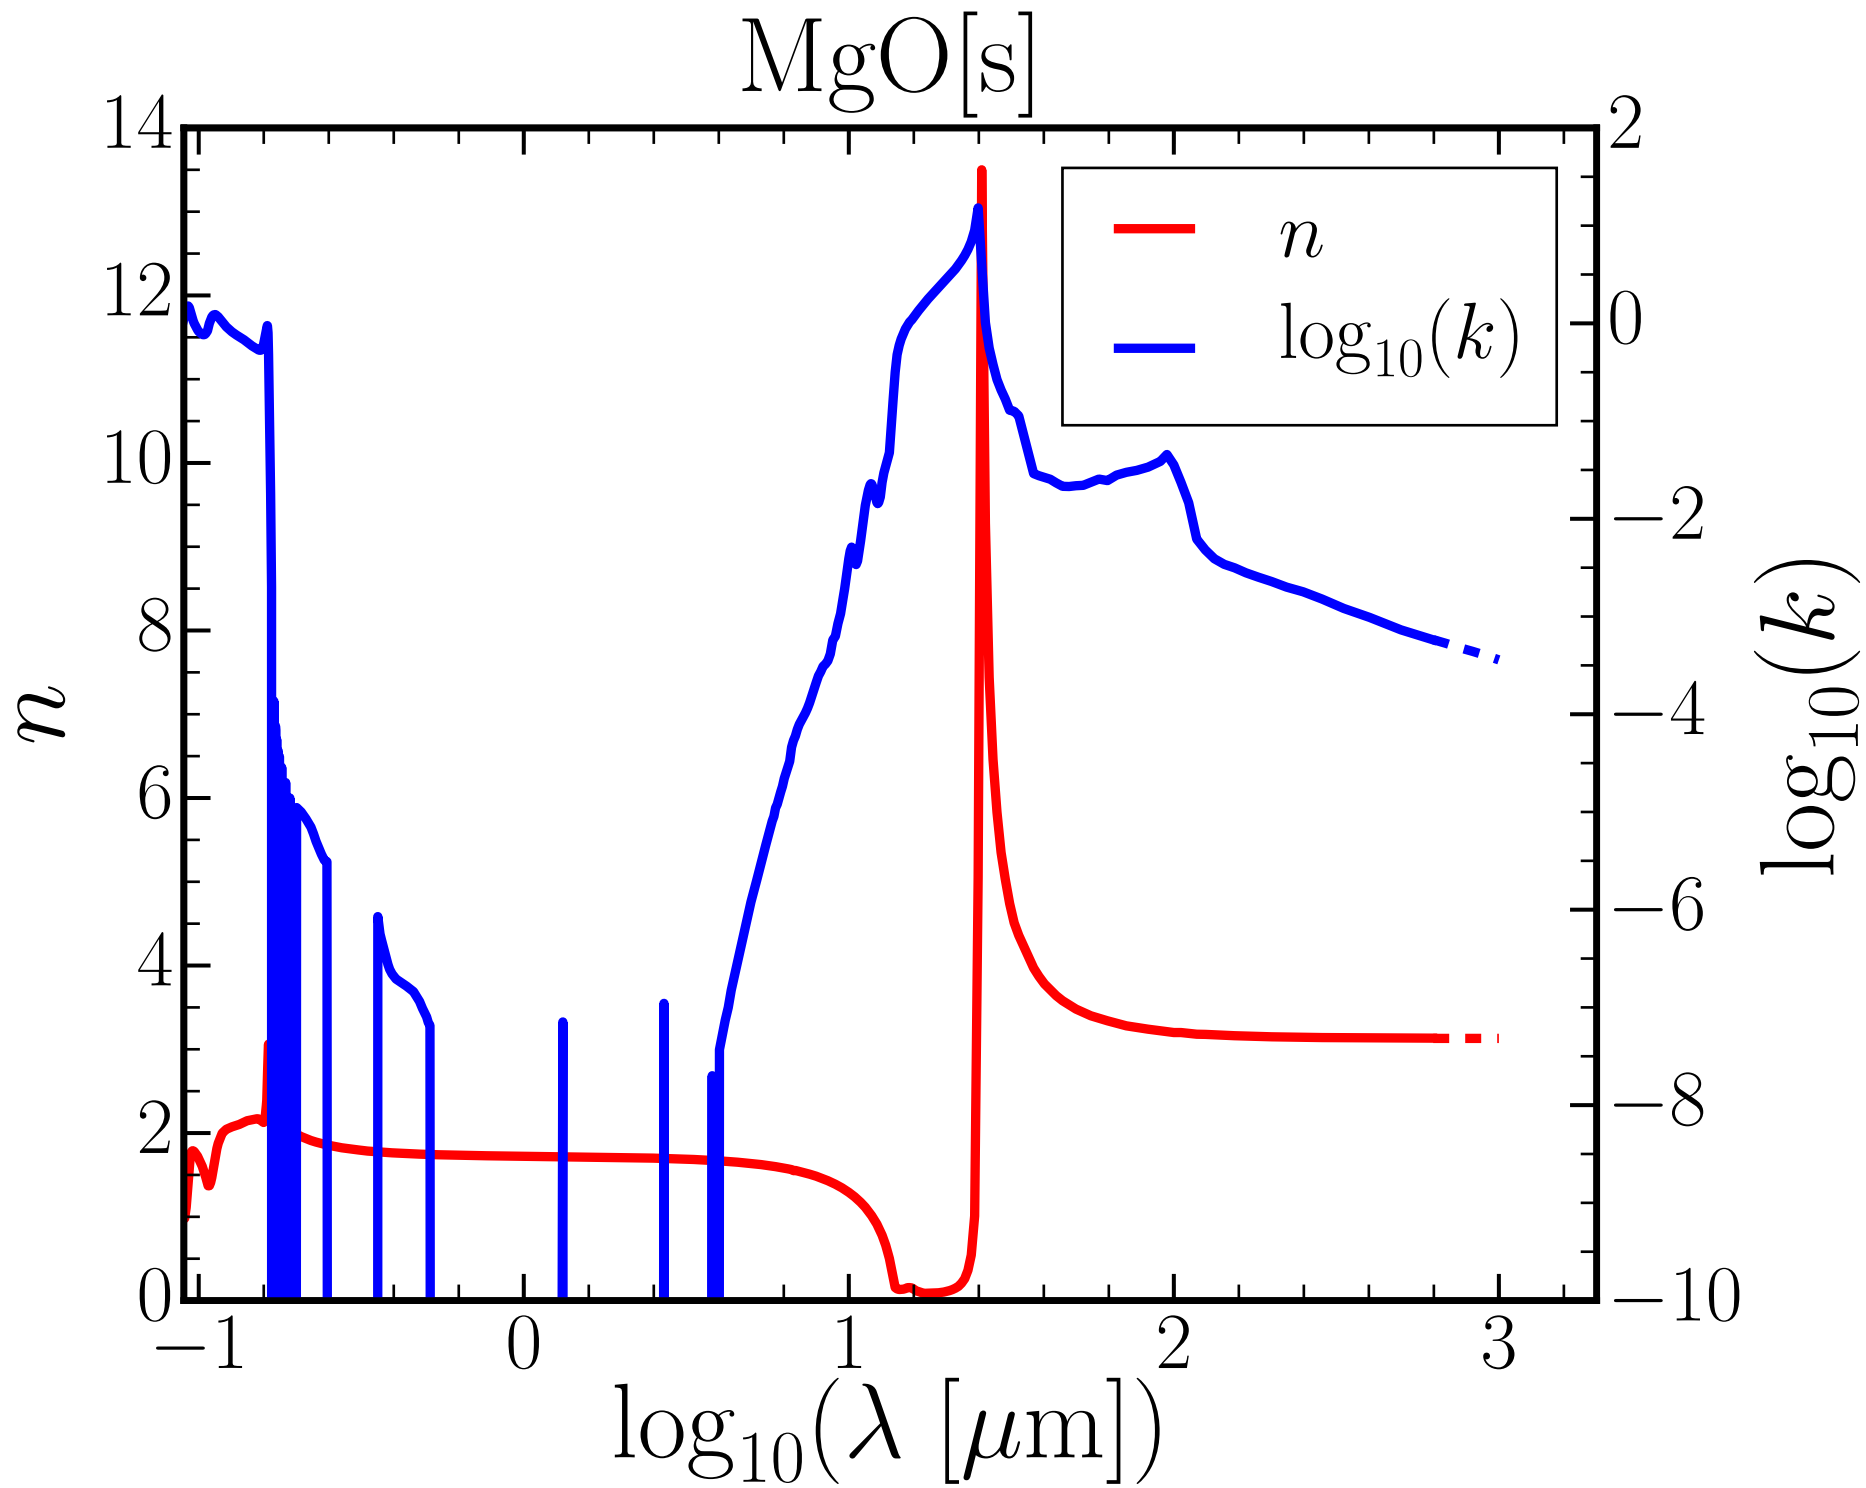

MgSiO<sub>3</sub>[s]

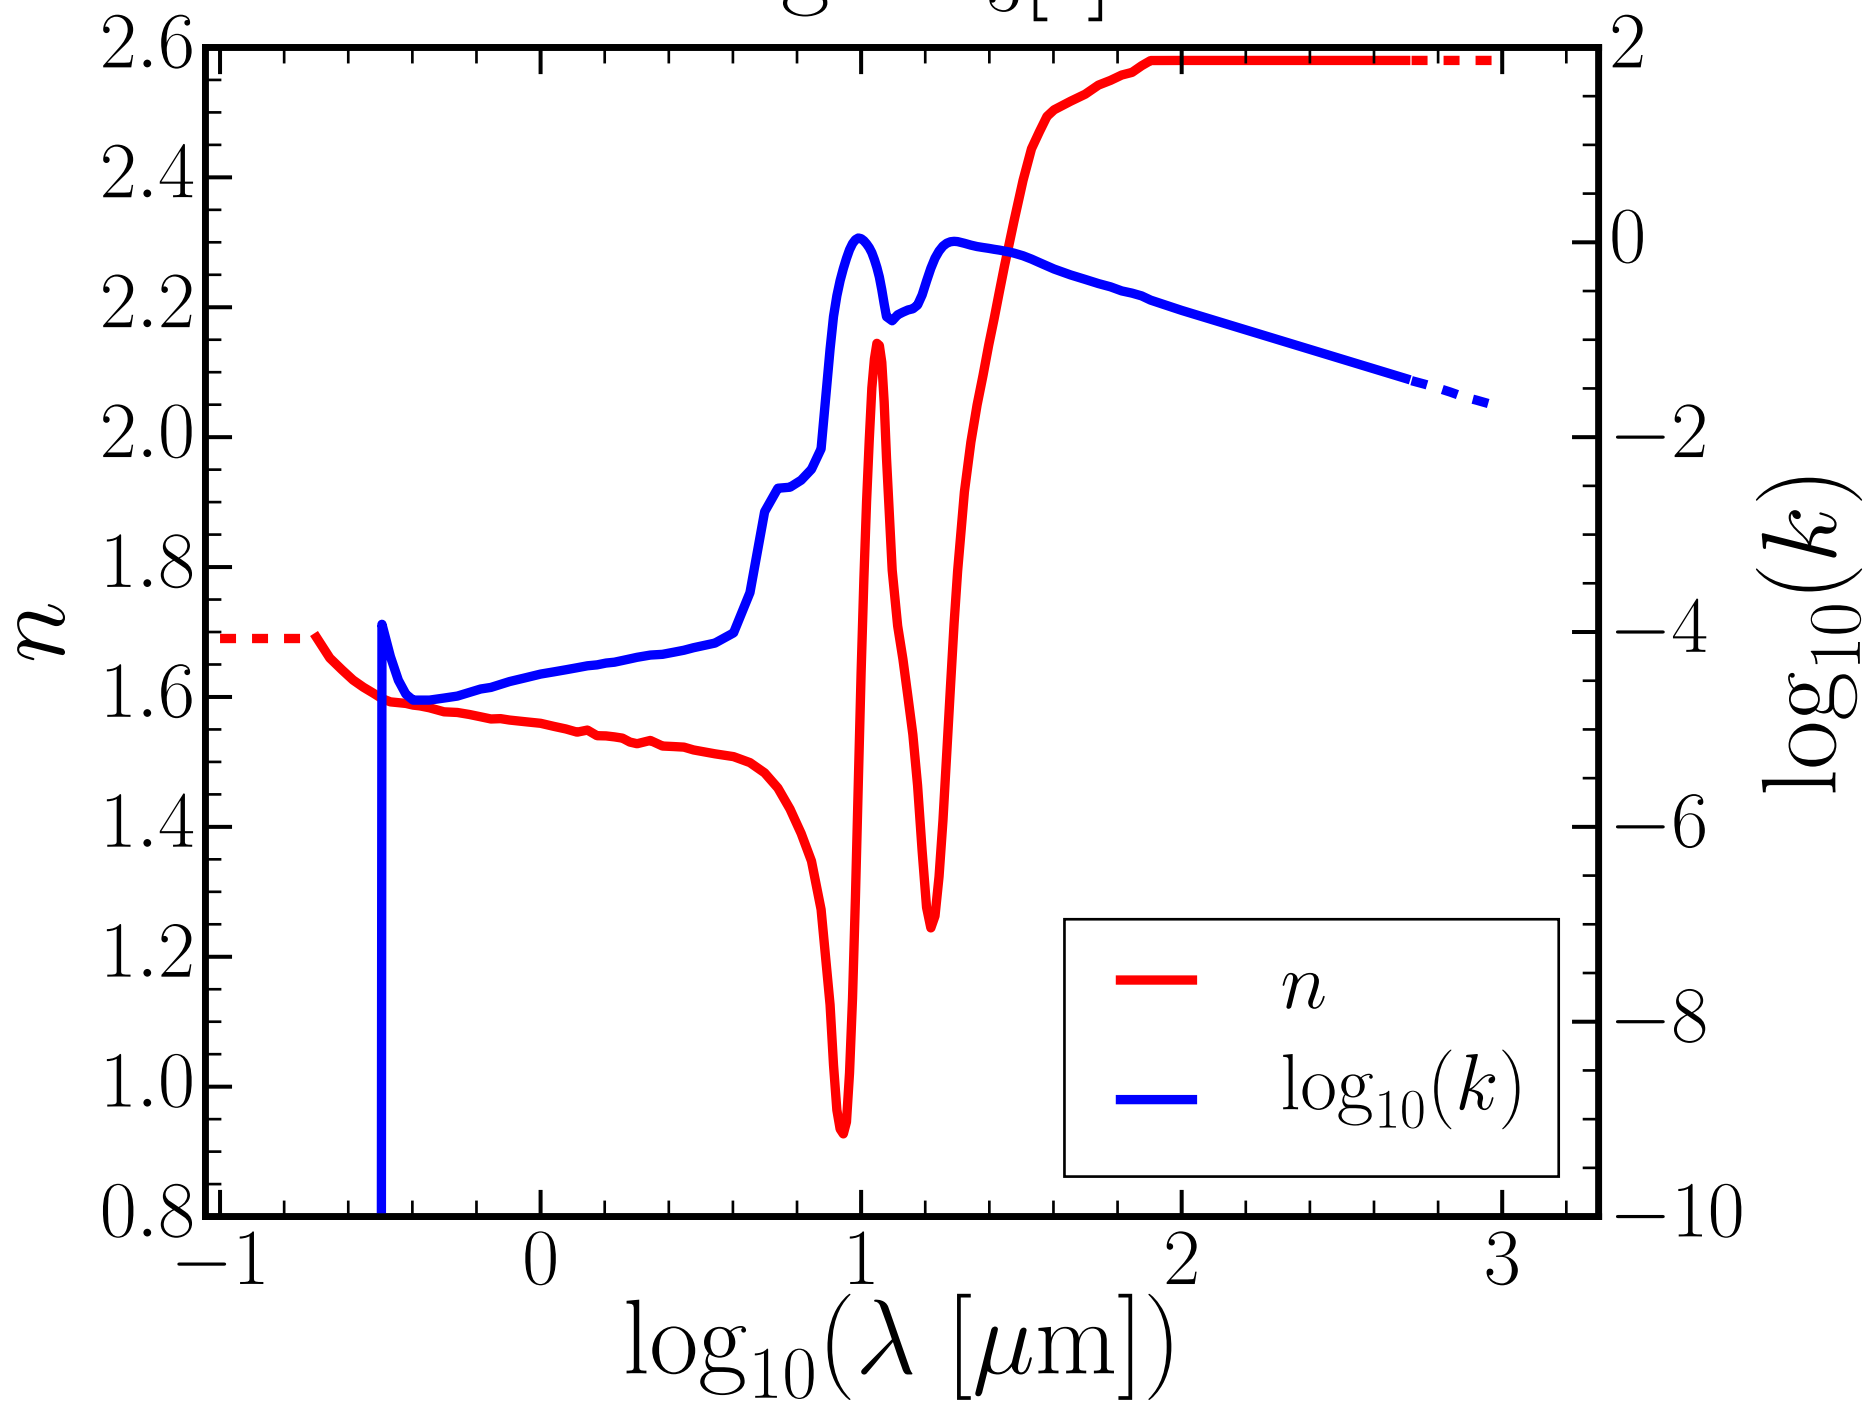

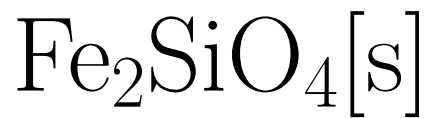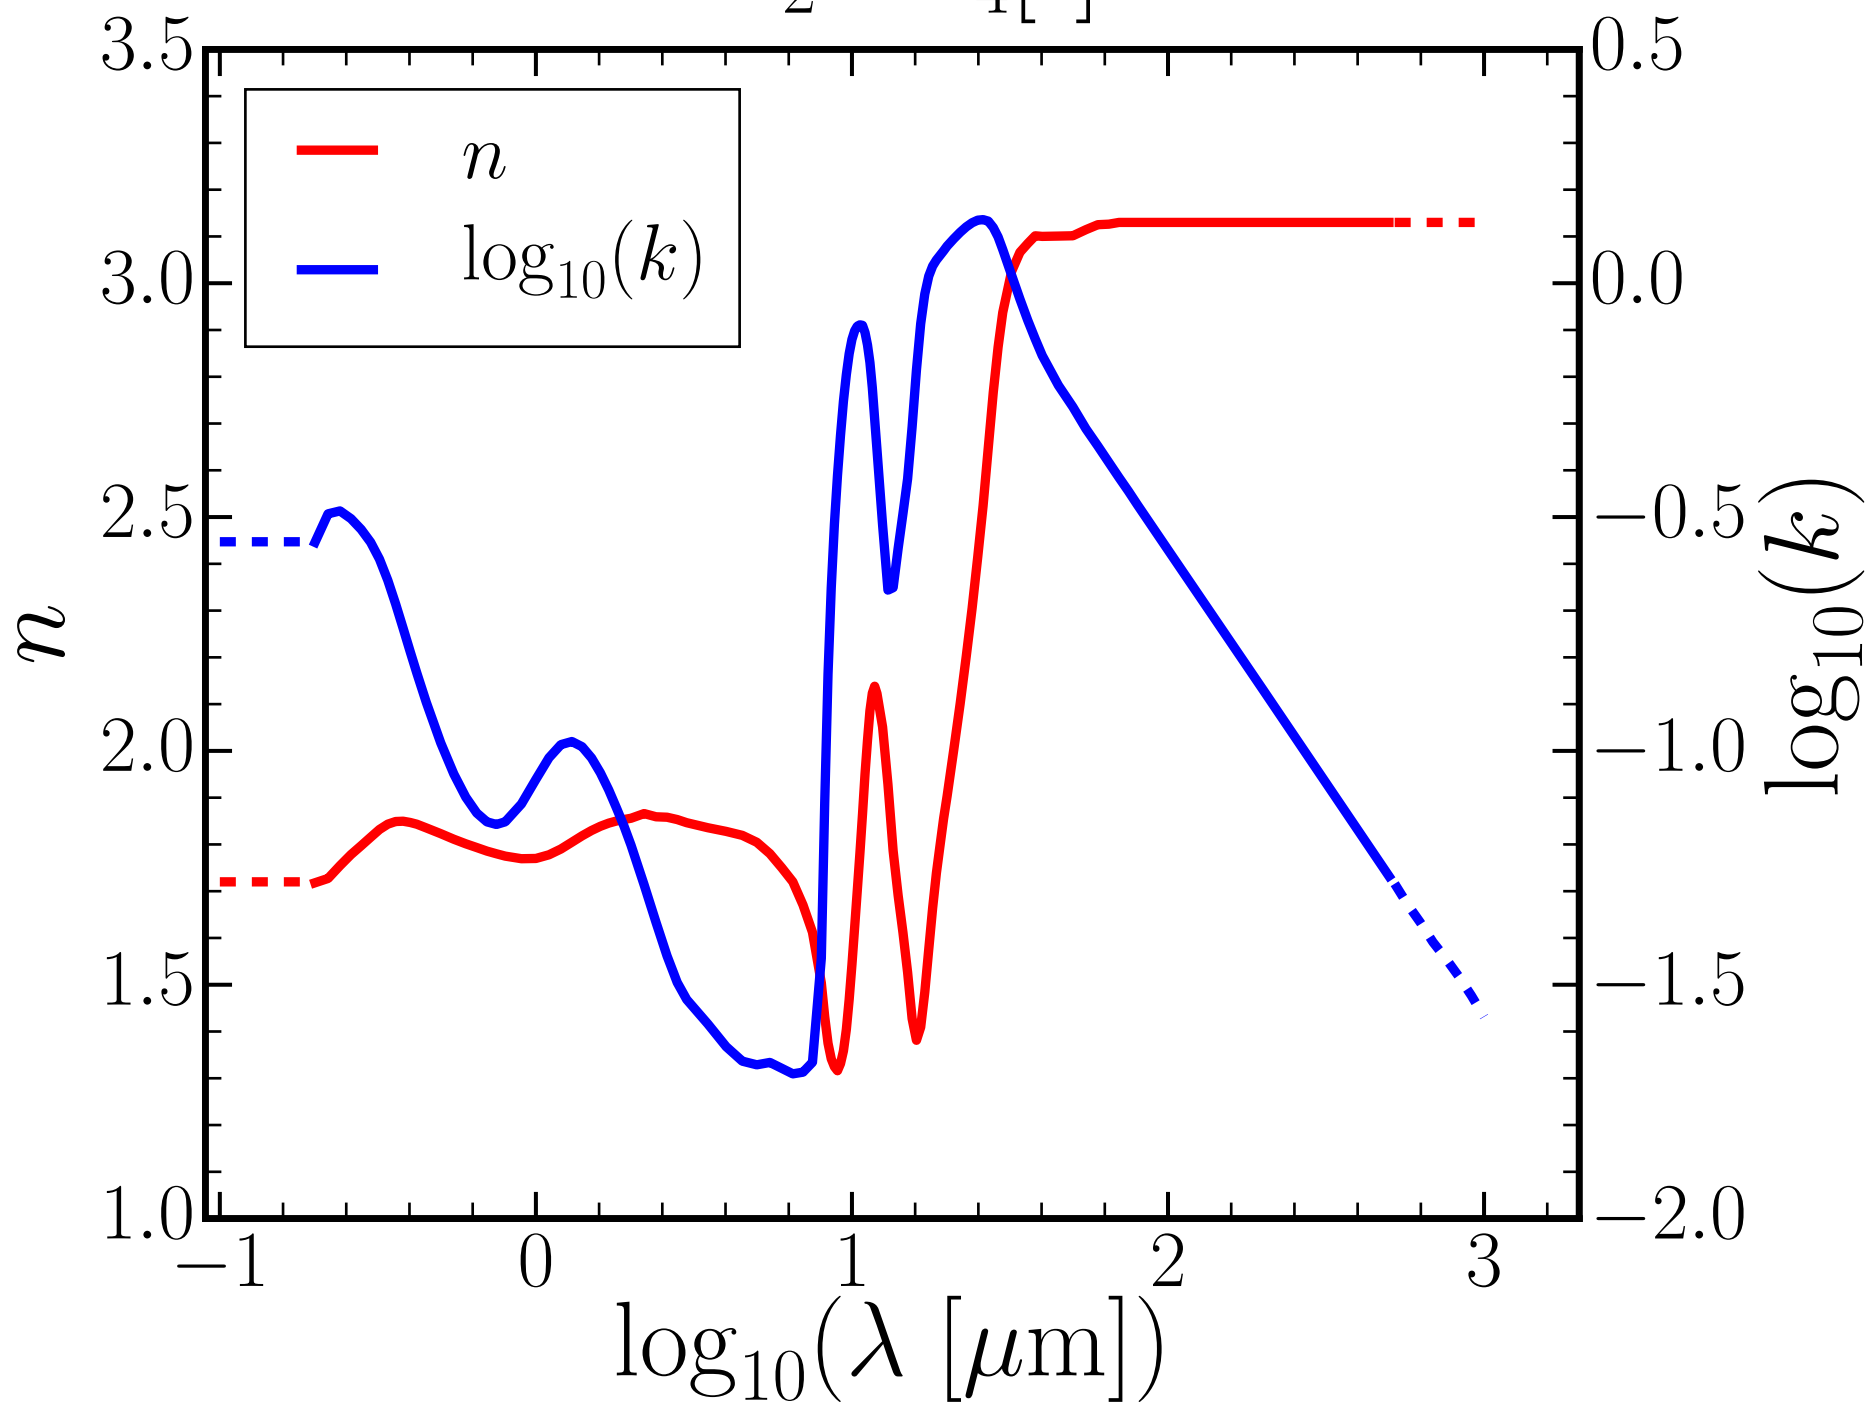

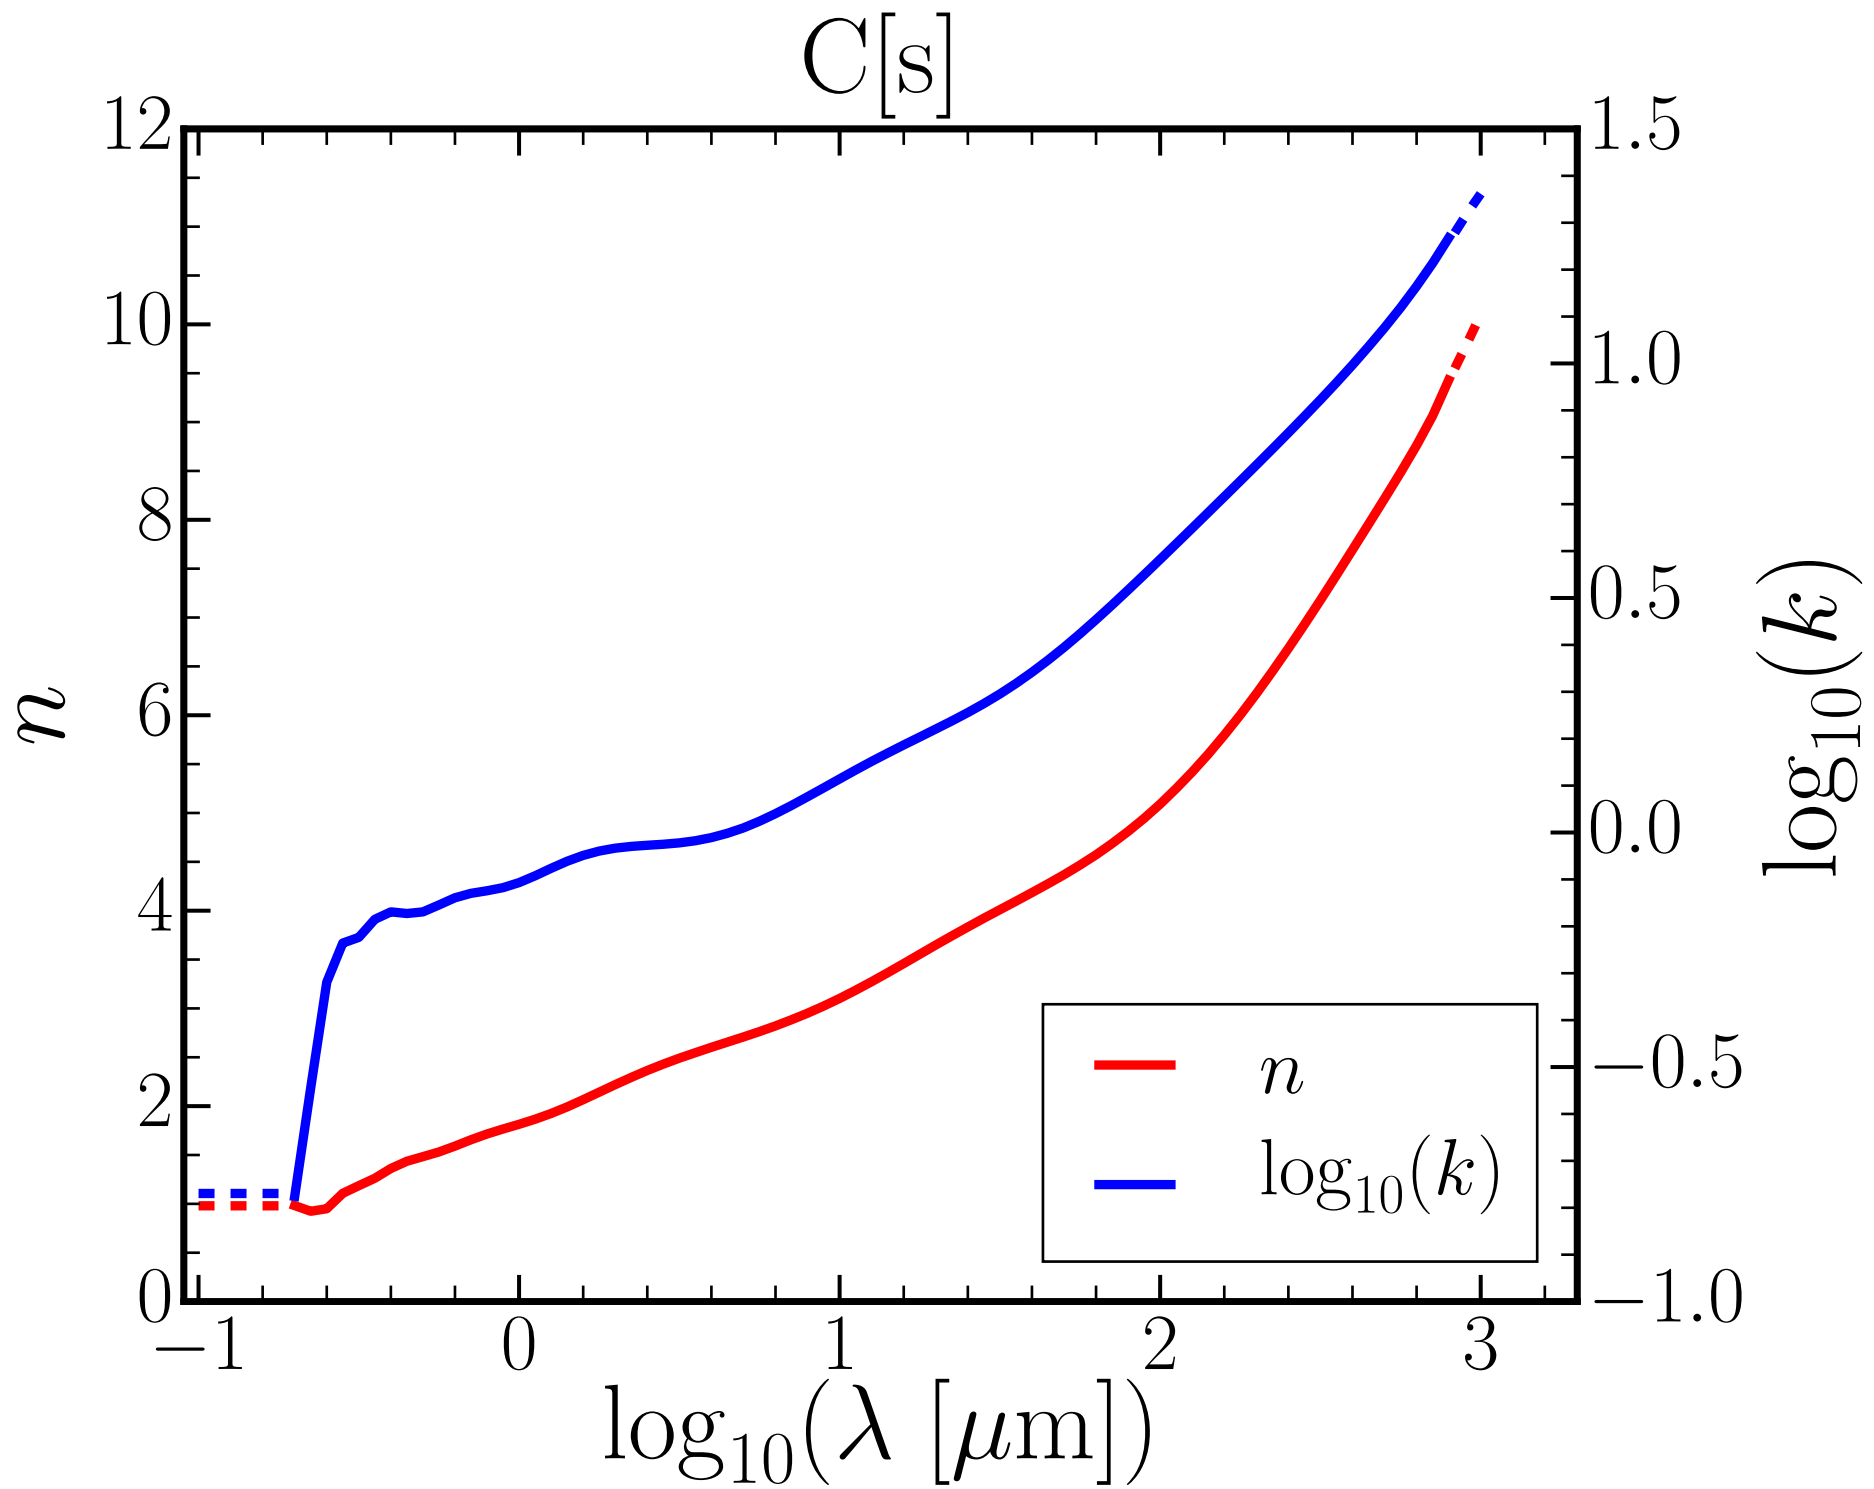

Supplement: Supplementary file 3 [file SW_Material_Refractive_Indexes_APPENDIX.pdf]
